# Supplementary material for: Neon in ultrashort and intense x rays from free electron lasers
Source: arXiv:1705.07521 ancillary file (2022-11-07)
Supplement: Supplementary file 1 [file neon_Bhalla.pdf]

```
Get["NeonRateEquations.m", Path -> NotebookDirectory[]]
```

```
HartreeToeV := 27.2113845
eVToHartree := 1/HartreeToeV
HartreeTomeV := 1000 * HartreeToeV
JouleToHartree := 2.29371269*^17
MilliJouleToHartree := 1*^-3 * JouleToHartree
BohrToAngstroem := 0.5291772083
AngstroemToBohr := 1/BohrToAngstroem
MicrometerToBohr := 1*^4 * AngstroemToBohr
BohrToMicrometer := 1/MicrometerToBohr
t0ToSecond := 24.18884326505*^-18
t0ToFemtoSecond := 24.18884326505*^-3
FemtoSecondTot0 := 1/t0ToFemtoSecond
crossSectionAUtoBarn := 1*^8 * BohrToAngstroem^2
crossSectionAUtocm2 := crossSectionAUtoBarn * 1*^-24
crossSectioncm2toAU := 1/crossSectionAUtocm2
intensityAUtoSI := 6.436409085121321*^15
intensitySItoAU := 1/intensityAUtoSI
```

# Hartree-Fock-Slater versus CAESR for neon

Christian Buth, 11 May 2017

Theoretische Chemie, Physikalisch-Chemisches Institut, Ruprecht-Karls-Universität Heidelberg, Im  
Neuenheimer Feld 229, 69120 Heidelberg, Germany

---

## Parameters

```
histen := {-5, 15, 1}
histrad := {-5, 3, 0.3}
histrange := {0, 30, 2}
histex := {-3, 22, 2}
```

Energies for the normal configurations to convert the energy shifts in Table I of Ref. [1]:

$E_X(2p \rightarrow 1s) = 848.5 \text{ eV}$ ;  $E_A(2s-2s) = 747.3 \text{ eV}$ ;  $E_A(2s-2p) = 780.0 \text{ eV}$ ;  $E_A(2p-2p) = 807.7 \text{ eV}$

$\text{enR225v126} * \text{HartreeToeV}$

849.65

enA206v126 \* HartreeToeV

747.534

enA215v126 \* HartreeToeV

780.674

enA224v126 \* HartreeToeV

808.625

---

## Bhalla's Auger transition energy shifts

### 2p–2p decay of single core holes

bhenA224v126 := 0.0 \* eVToHartree

bhenA223v125 := -19.5 \* eVToHartree

bhenA222v124 := -40.4 \* eVToHartree

bhenA221v123 := -62.7 \* eVToHartree

bhenA220v122 := -86.3 \* eVToHartree

bhenA214v116 := -16.3 \* eVToHartree

bhenA213v115 := -37.0 \* eVToHartree

bhenA212v114 := -59.1 \* eVToHartree

bhenA211v113 := -82.5 \* eVToHartree

bhenA210v112 := -106.9 \* eVToHartree

bhenA204v106 := -33.6 \* eVToHartree

bhenA203v105 := -55.5 \* eVToHartree

bhenA202v104 := -78.5 \* eVToHartree

bhenA201v103 := -102.8 \* eVToHartree

bhenA200v102 := -129.2 \* eVToHartree

bh = {bhenA223v125, bhenA222v124, bhenA221v123, bhenA220v122,  
bhenA214v116, bhenA213v115, bhenA212v114, bhenA211v113, bhenA210v112,  
bhenA204v106, bhenA203v105, bhenA202v104, bhenA201v103, bhenA200v102}

{-0.716612, -1.48467, -2.30418, -3.17147, -0.599014, -1.35973, -2.17189,  
-3.03182, -3.9285, -1.23478, -2.03959, -2.88482, -3.77783, -4.74801}

ga = {enA223v125, enA222v124, enA221v123, enA220v122, enA214v116,  
enA213v115, enA212v114, enA211v113, enA210v112, enA204v106,  
enA203v105, enA202v104, enA201v103, enA200v102} - enA224v126

{-0.71106, -1.47734, -2.29667, -3.16843, -0.587586, -1.34747, -2.16025,  
-3.02508, -3.94207, -1.23013, -2.03202, -2.88569, -3.79121, -4.74921}

(ga - bh) / ga \* 100

{-0.780782, -0.496686, -0.327154, -0.0959374, -1.94491, -0.909483, -0.538645,  
-0.222846, 0.344165, -0.377545, -0.372463, 0.0302535, 0.352802, 0.0251257}

```
Histogram[(ga - bh) / ga * 100, histen, AxesLabel -> {"%", "Number"},
  AxesStyle -> {{Arrowheads[Automatic], AbsoluteThickness[0.8]},
    {Arrowheads[Automatic], AbsoluteThickness[0.8]}},
  LabelStyle -> {FontFamily -> "Helvetica", FontSize -> 14}]
```

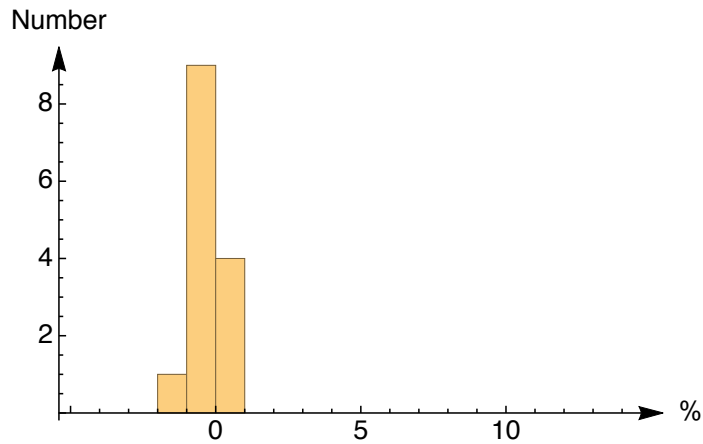

```
Mean[(ga - bh) / ga * 100]
```

```
-0.379579
```

```
StandardDeviation[(ga - bh) / ga * 100]
```

```
0.583806
```

## 2s-2p decay of single core holes

```
bhenA215v126 := 0.0 * eVToHartree
```

```
bhenA214v125 := -17.2 * eVToHartree
```

```
bhenA213v124 := -35.1 * eVToHartree
```

```
bhenA212v123 := -53.8 * eVToHartree
```

```
bhenA211v122 := -73.0 * eVToHartree
```

```
bhenA210v121 := -92.6 * eVToHartree
```

```
bhenA205v116 := -19.4 * eVToHartree
```

```
bhenA204v115 := -37.4 * eVToHartree
```

```
bhenA203v114 := -56.2 * eVToHartree
```

```
bhenA202v113 := -75.5 * eVToHartree
```

```
bhenA201v112 := -95.2 * eVToHartree
```

```
bhenA200v111 := -116.4 * eVToHartree
```

```
bh = {bhenA214v125, bhenA213v124, bhenA212v123,
```

```
  bhenA211v122, bhenA210v121, bhenA205v116, bhenA204v115,
```

```
  bhenA203v114, bhenA202v113, bhenA201v112, bhenA200v111}
```

```
{-0.632088, -1.2899, -1.97711, -2.6827, -3.40299,
```

```
-0.712937, -1.37442, -2.06531, -2.77457, -3.49854, -4.27762}
```

```
ga = {enA214v125, enA213v124, enA212v123, enA211v122, enA210v121, enA205v116,
      enA204v115, enA203v114, enA202v113, enA201v112, enA200v111} - enA215v126
{-0.625039, -1.27996, -1.96209, -2.67047, -3.40513,
 -0.703692, -1.3645, -2.05293, -2.76761, -3.50831, -4.27552}
```

```
(ga - bh) / ga * 100
{-1.12783, -0.776845, -0.765594, -0.458148, 0.0628331,
 -1.31377, -0.72728, -0.602993, -0.251553, 0.278519, -0.0491022}
```

```
Histogram[(ga - bh) / ga * 100, histen, AxesLabel → {"%", "Number"},
  AxesStyle → {{Arrowheads[Automatic], AbsoluteThickness[0.8]},
    {Arrowheads[Automatic], AbsoluteThickness[0.8]}},
  LabelStyle → {FontFamily → "Helvetica", FontSize → 14}]
```

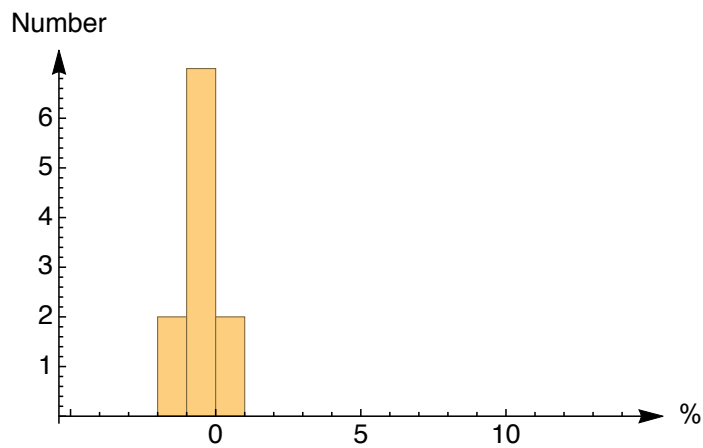

```
Mean[(ga - bh) / ga * 100]
```

```
-0.521069
```

```
StandardDeviation[(ga - bh) / ga * 100]
```

```
0.495037
```

## 2s–2s decay of single core holes

```
bhenA206v126 := 0.0 * eVToHartree
```

```
bhenA205v125 := -15.2 * eVToHartree
```

```
bhenA204v124 := -30.4 * eVToHartree
```

```
bhenA203v123 := -45.7 * eVToHartree
```

```
bhenA202v122 := -60.9 * eVToHartree
```

```
bhenA201v121 := -75.7 * eVToHartree
```

```
bh = {bhenA205v125, bhenA204v124, bhenA203v123, bhenA202v122, bhenA201v121}
```

```
{-0.55859, -1.11718, -1.67944, -2.23803, -2.78192}
```

```
ga = {enA205v125, enA204v124, enA203v123, enA202v122, enA201v121} - enA206v126
```

```
{-0.550454, -1.1063, -1.66409, -2.22231, -2.78067}
```

```
(ga - bh) / ga * 100
```

```
{-1.478, -0.983593, -0.922978, -0.707591, -0.0449843}
```

```
Histogram[(ga - bh) / ga * 100, histen, AxesLabel -> {"%", "Number"},
  AxesStyle -> {{Arrowheads[Automatic], AbsoluteThickness[0.8]},
    {Arrowheads[Automatic], AbsoluteThickness[0.8]}},
  LabelStyle -> {FontFamily -> "Helvetica", FontSize -> 14}]
```

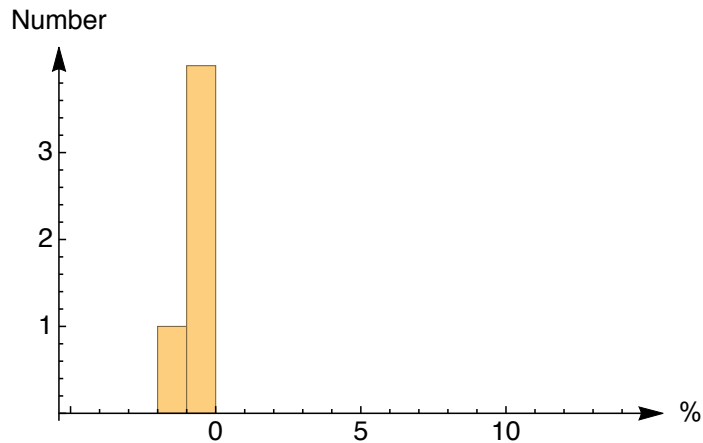

```
Mean[(ga - bh) / ga * 100]
```

```
-0.82743
```

```
StandardDeviation[(ga - bh) / ga * 100]
```

```
0.520419
```

## 2p-2p decay of double core holes

```
bhenA124v026 := 65.4 * eVToHartree
bhenA123v025 := 42.9 * eVToHartree
bhenA122v024 := 19.0 * eVToHartree
bhenA121v023 := -6.2 * eVToHartree
bhenA120v022 := -32.7 * eVToHartree
```

```
bhenA114v016 := 46.5 * eVToHartree
bhenA113v015 := 22.8 * eVToHartree
bhenA112v014 := -2.3 * eVToHartree
bhenA111v013 := -28.6 * eVToHartree
bhenA110v012 := -56.2 * eVToHartree
```

```
bhenA104v006 := 26.5 * eVToHartree
bhenA103v005 := 1.7 * eVToHartree
bhenA102v004 := -24.4 * eVToHartree
bhenA101v003 := -51.7 * eVToHartree
bhenA100v002 := -80.5 * eVToHartree
```

```

bh = {bhenA124v026, bhenA123v025, bhenA122v024, bhenA121v023, bhenA120v022,
      bhenA114v016, bhenA113v015, bhenA112v014, bhenA111v013, bhenA110v012,
      bhenA104v006, bhenA103v005, bhenA102v004, bhenA101v003, bhenA100v002}
{2.40341, 1.57655, 0.698237, -0.227846, -1.2017, 1.70884, 0.837885, -0.0845234,
 -1.05103, -2.06531, 0.973857, 0.0624739, -0.896684, -1.89994, -2.95832}

```

```

ga = {enA124v026, enA123v025, enA122v024, enA121v023, enA120v022,
      enA114v016, enA113v015, enA112v014, enA111v013, enA110v012, enA104v006,
      enA103v005, enA102v004, enA101v003, enA100v002} - enA224v126
{2.41357, 1.58919, 0.711532, -0.218342, -1.20026, 1.71918, 0.853547, -0.064291,
 -1.03406, -2.05611, 0.997332, 0.087193, -0.874572, -1.88821, -2.95441}

```

```

(ga - bh) / ga * 100
{0.421209, 0.795811, 1.86848, -4.35272, -0.120217, 0.60153, 1.83498, -31.4701,
 -1.64068, -0.447595, 2.35377, 28.3499, -2.52827, -0.620961, -0.132366}

```

```

Histogram[(ga - bh) / ga * 100, {-32, 30, 1}, AxesLabel -> {"%", "Number"},
  AxesStyle -> {{Arrowheads[Automatic], AbsoluteThickness[0.8]},
    {Arrowheads[Automatic], AbsoluteThickness[0.8]}},
  LabelStyle -> {FontFamily -> "Helvetica", FontSize -> 14}]

```

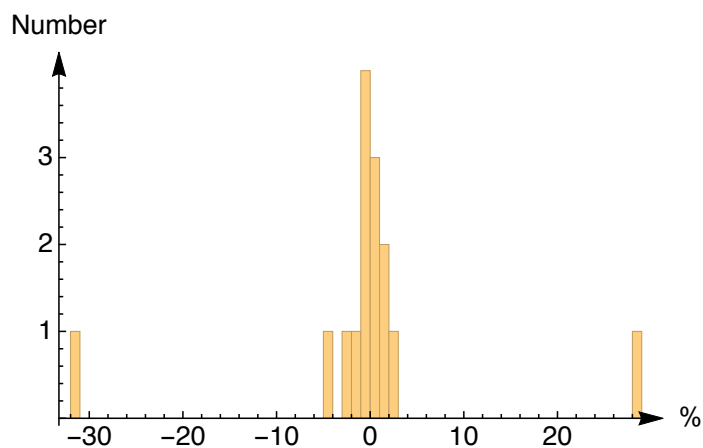

```
Mean[(ga - bh) / ga * 100]
```

```
-0.339147
```

```
StandardDeviation[(ga - bh) / ga * 100]
```

```
11.4473
```

## 2s–2p decay of double core holes

```
bhenA115v026 := 67.3 * eVToHartree
bhenA114v025 := 48.3 * eVToHartree
bhenA113v024 := 28.5 * eVToHartree
bhenA112v023 := 8.1 * eVToHartree
bhenA111v022 := -12.9 * eVToHartree
bhenA110v021 := -34.5 * eVToHartree
```

```
bhenA105v016 := 45.8 * eVToHartree
bhenA104v015 := 25.9 * eVToHartree
bhenA103v014 := 5.3 * eVToHartree
bhenA102v013 := -15.8 * eVToHartree
bhenA101v012 := -37.4 * eVToHartree
bhenA100v011 := -59.8 * eVToHartree
```

```
bh = {bhenA115v026, bhenA114v025, bhenA113v024, bhenA112v023,
      bhenA111v022, bhenA110v021, bhenA105v016, bhenA104v015,
      bhenA103v014, bhenA102v013, bhenA101v012, bhenA100v011}
{2.47323, 1.77499, 1.04736, 0.29767, -0.474066, -1.26785,
 1.68312, 0.951808, 0.194771, -0.580639, -1.37442, -2.19761}
```

```
ga = {enA115v026, enA114v025, enA113v024,
      enA112v023, enA111v022, enA110v021, enA105v016, enA104v015,
      enA103v014, enA102v013, enA101v012, enA100v011} - enA215v126
{2.48108, 1.78735, 1.06614, 0.318602, -0.455098, -1.2554,
 1.69827, 0.971631, 0.218607, -0.56038, -1.36561, -2.19783}
```

```
(ga - bh) / ga * 100
{0.316574, 0.691394, 1.76226, 6.5701, -4.16796, -0.991931,
 0.892198, 2.04023, 10.9034, -3.61528, -0.64548, 0.00998225}
```

```
Histogram[(ga - bh) / ga * 100, histen, AxesLabel -> {"%", "Number"},
  AxesStyle -> {{Arrowheads[Automatic], AbsoluteThickness[0.8]},
    {Arrowheads[Automatic], AbsoluteThickness[0.8]}},
  LabelStyle -> {FontFamily -> "Helvetica", FontSize -> 14}]
```

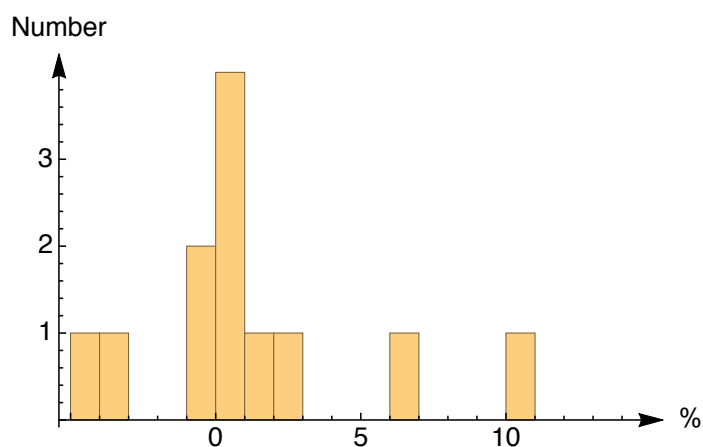

```
Mean[(ga - bh) / ga * 100]
```

```
1.14712
```

```
StandardDeviation[(ga - bh) / ga * 100]
```

```
4.12029
```

## 2s–2s decay of double core holes

```
bhenA106v026 := 68.6 * eVToHartree
```

```
bhenA105v025 := 52.6 * eVToHartree
```

```
bhenA104v024 := 36.7 * eVToHartree
```

```
bhenA103v023 := 20.8 * eVToHartree
```

```
bhenA102v022 := 5.0 * eVToHartree
```

```
bhenA101v021 := -10.6 * eVToHartree
```

```
bh = {bhenA106v026, bhenA105v025,
  bhenA104v024, bhenA103v023, bhenA102v022, bhenA101v021}
{2.521, 1.93301, 1.3487, 0.764386, 0.183747, -0.389543}
```

```
ga = {enA106v026, enA105v025, enA104v024,
  enA103v023, enA102v022, enA101v021} - enA206v126
{2.53741, 1.95713, 1.37492, 0.792191, 0.209277, -0.374209}
```

```
(ga - bh) / ga * 100
{0.646461, 1.23209, 1.90686, 3.50989, 12.1993, -4.09767}
```



```
Histogram[(ga - bh) / ga * 100, histen, AxesLabel -> {"%", "Number"},
  AxesStyle -> {{Arrowheads[Automatic], AbsoluteThickness[0.8]},
    {Arrowheads[Automatic], AbsoluteThickness[0.8]}},
  LabelStyle -> {FontFamily -> "Helvetica", FontSize -> 14}]
```

Number

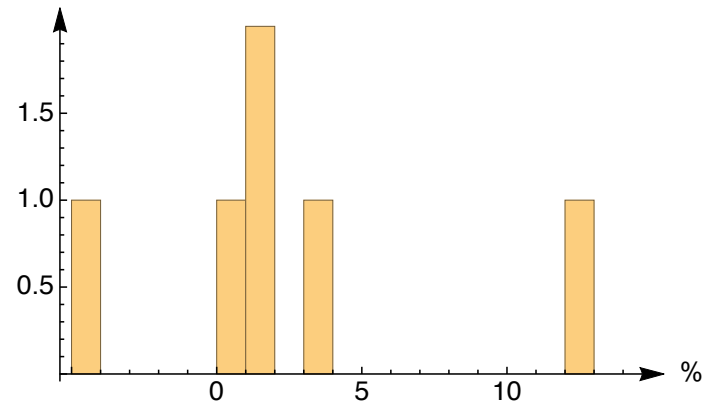

```
Mean[(ga - bh) / ga * 100]
```

2.56616

```
StandardDeviation[(ga - bh) / ga * 100]
```

5.36646

## Bhalla's radiative transition energy shifts

### Single core holes

```

bhenR225v126 := 0.0 * eVToHartree
bhenR224v125 := 5.2 * eVToHartree
bhenR223v124 := 12.2 * eVToHartree
bhenR222v123 := 20.5 * eVToHartree
bhenR221v122 := 30.5 * eVToHartree
bhenR220v121 := 42.2 * eVToHartree

bhenR215v116 := 6.1 * eVToHartree
bhenR214v115 := 12.4 * eVToHartree
bhenR213v114 := 20.4 * eVToHartree
bhenR212v113 := 30.0 * eVToHartree
bhenR211v112 := 41.2 * eVToHartree
bhenR210v111 := 54.1 * eVToHartree

bhenR205v106 := 13.2 * eVToHartree
bhenR204v105 := 20.7 * eVToHartree
bhenR203v104 := 29.8 * eVToHartree
bhenR202v103 := 40.5 * eVToHartree
bhenR201v102 := 53.1 * eVToHartree
bhenR200v101 := 65.9 * eVToHartree

bh = {bhenR224v125, bhenR223v124, bhenR222v123, bhenR221v122,
      bhenR220v121, bhenR215v116, bhenR214v115, bhenR213v114,
      bhenR212v113, bhenR211v112, bhenR210v111, bhenR205v106,
      bhenR204v105, bhenR203v104, bhenR202v103, bhenR201v102, bhenR200v101}
{0.191096, 0.448342, 0.753361, 1.12085, 1.55082,
 0.224171, 0.455692, 0.749686, 1.10248, 1.51407, 1.98814,
 0.485091, 0.760711, 1.09513, 1.48835, 1.95139, 2.42178}

ga = {enR224v125, enR223v124, enR222v123, enR221v122, enR220v121, enR215v116,
      enR214v115, enR213v114, enR212v113, enR211v112, enR210v111, enR205v106,
      enR204v105, enR203v104, enR202v103, enR201v102, enR200v101} - enR225v126
{0.191065, 0.443229, 0.754901, 1.12435, 1.5497, 0.228518, 0.461737, 0.754121,
 1.10431, 1.51071, 1.97154, 0.479999, 0.758004, 1.09355, 1.48528, 1.93162, 2.4308}

(ga - bh) / ga * 100
{-0.01648, -1.15353, 0.20398, 0.310811, -0.0726268,
 1.90231, 1.30927, 0.588073, 0.16619, -0.222357, -0.842005,
 -1.06085, -0.357124, -0.144747, -0.206469, -1.02361, 0.371215}

```

```
Histogram[(ga - bh) / ga * 100, histrad, AxesLabel -> {"%", "Number"},
  AxesStyle -> {{Arrowheads[Automatic], AbsoluteThickness[0.8]},
    {Arrowheads[Automatic], AbsoluteThickness[0.8]}},
  LabelStyle -> {FontFamily -> "Helvetica", FontSize -> 14}]
```

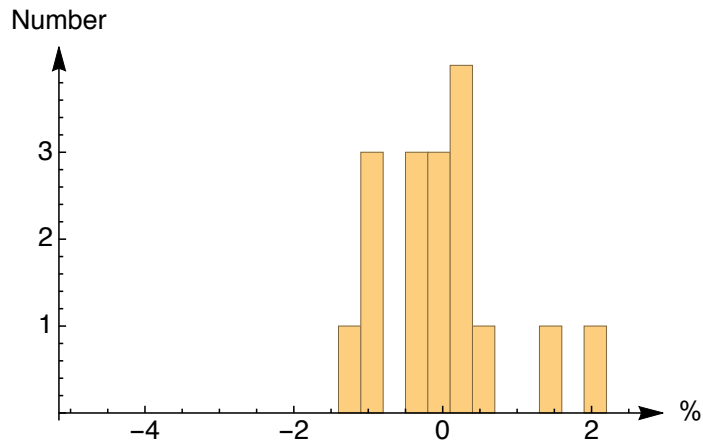

```
Mean[(ga - bh) / ga * 100]
```

```
-0.014585
```

```
StandardDeviation[(ga - bh) / ga * 100]
```

```
0.807685
```

## Double core holes

```
bhenR125v026 := 96.9 * eVToHartree
bhenR124v025 := 103.8 * eVToHartree
bhenR123v024 := 112.2 * eVToHartree
bhenR122v023 := 122.2 * eVToHartree
bhenR121v022 := 133.8 * eVToHartree
bhenR120v021 := 146.8 * eVToHartree
```

```
bhenR115v016 := 103.9 * eVToHartree
bhenR114v015 := 111.9 * eVToHartree
bhenR113v014 := 121.4 * eVToHartree
bhenR112v013 := 132.4 * eVToHartree
bhenR111v012 := 145.0 * eVToHartree
bhenR110v011 := 159.1 * eVToHartree
```

```
bhenR105v006 := 111.8 * eVToHartree
bhenR104v005 := 120.8 * eVToHartree
bhenR103v004 := 131.4 * eVToHartree
bhenR102v003 := 143.5 * eVToHartree
bhenR101v002 := 164.0 * eVToHartree
```

```

bh = {bhenR125v026, bhenR124v025, bhenR123v024, bhenR122v023,
      bhenR121v022, bhenR120v021, bhenR115v016, bhenR114v015,
      bhenR113v014, bhenR112v013, bhenR111v012, bhenR110v011,
      bhenR105v006, bhenR104v005, bhenR103v004, bhenR102v003, bhenR101v002}
{3.56101, 3.81458, 4.12327, 4.49077, 4.91706, 5.3948, 3.81825, 4.11225, 4.46137,
  4.86561, 5.32865, 5.84682, 4.10857, 4.43932, 4.82886, 5.27353, 6.02689}

```

```

ga = {enR125v026, enR124v025, enR123v024, enR122v023, enR121v022, enR120v021,
      enR115v016, enR114v015, enR113v014, enR112v013, enR111v012, enR110v011,
      enR105v006, enR104v005, enR103v004, enR102v003, enR101v002} - enR225v126
{3.56786, 3.82143, 4.13255, 4.49978, 4.92157, 5.39626, 3.82078, 4.11811,
  4.4715, 4.87954, 5.34071, 5.8534, 4.1229, 4.45817, 4.84825, 5.2918, 5.78732}

```

```

(ga - bh) / ga * 100
{0.192033, 0.179255, 0.224457, 0.200311, 0.0915842,
 0.0271143, 0.0659861, 0.142337, 0.226591, 0.285548, 0.225868,
 0.112524, 0.347438, 0.422833, 0.399912, 0.345212, -4.13952}

```

```

Histogram[(ga - bh) / ga * 100, histrad, AxesLabel -> {"%", "Number"},
  AxesStyle -> {{Arrowheads[Automatic], AbsoluteThickness[0.8]},
    {Arrowheads[Automatic], AbsoluteThickness[0.8]}},
  LabelStyle -> {FontFamily -> "Helvetica", FontSize -> 14}]

```

Number

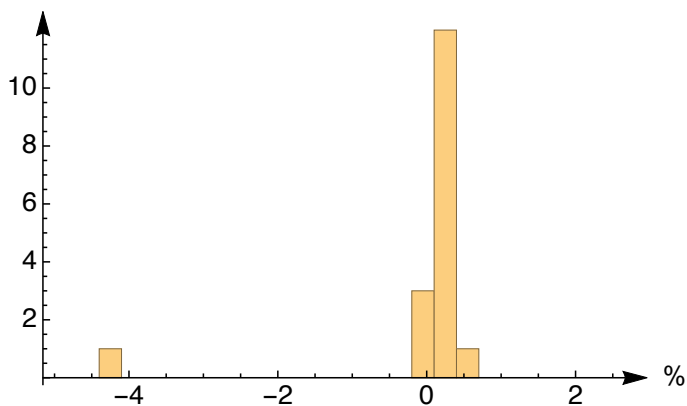

```
Mean[(ga - bh) / ga * 100]
```

```
-0.0382657
```

```
StandardDeviation[(ga - bh) / ga * 100]
```

```
1.06299
```

## Bhalla's Auger widths

### Total width of single core holes

```

bhGA126 := 88.066*^-4
bhGA125 := 78.753*^-4
bhGA124 := 66.278*^-4
bhGA123 := 51.633*^-4
bhGA122 := 36.687*^-4
bhGA121 := 23.994*^-4

bhGA116 := 80.428*^-4
bhGA115 := 67.321*^-4
bhGA114 := 51.162*^-4
bhGA113 := 33.624*^-4
bhGA112 := 17.113*^-4
bhGA111 := 4.716*^-4

bhGA106 := 77.901*^-4
bhGA105 := 61.854*^-4
bhGA104 := 43.571*^-4
bhGA103 := 25.306*^-4
bhGA102 := 9.682*^-4

bh = {bhGA126, bhGA125, bhGA124, bhGA123, bhGA122, bhGA121,
      bhGA116, bhGA115, bhGA114, bhGA113, bhGA112, bhGA111,
      bhGA106, bhGA105, bhGA104, bhGA103, bhGA102}

{0.0088066, 0.0078753, 0.0066278, 0.0051633, 0.0036687,
 0.0023994, 0.0080428, 0.0067321, 0.0051162, 0.0033624, 0.0017113,
 0.0004716, 0.0077901, 0.0061854, 0.0043571, 0.0025306, 0.0009682}

ga = {GamATot126, GamATot125, GamATot124, GamATot123, GamATot122, GamATot121,
      GamATot116, GamATot115, GamATot114, GamATot113, GamATot112, GamATot111,
      GamATot106, GamATot105, GamATot104, GamATot103, GamATot102}

{0.0101443, 0.00908152, 0.00769013, 0.00606984, 0.00439693,
 0.00295665, 0.00851707, 0.00718982, 0.0055801, 0.0037615, 0.00198967,
 0.000580309, 0.00876923, 0.00701997, 0.00502591, 0.00297236, 0.00113472}

(ga - bh) / ga * 100

{13.1869, 13.2821, 13.8142, 14.9352, 16.5623, 18.8473, 5.56846, 6.36622, 8.31347,
 10.6101, 13.9906, 18.733, 11.1655, 11.8885, 13.3072, 14.8623, 14.675}

```

```
Histogram[(ga - bh) / ga * 100, histrange, AxesLabel -> {"%", "Number"},
  AxesStyle -> {{Arrowheads[Automatic], AbsoluteThickness[0.8]},
    {Arrowheads[Automatic], AbsoluteThickness[0.8]}},
  LabelStyle -> {FontFamily -> "Helvetica", FontSize -> 14}]
```

Number

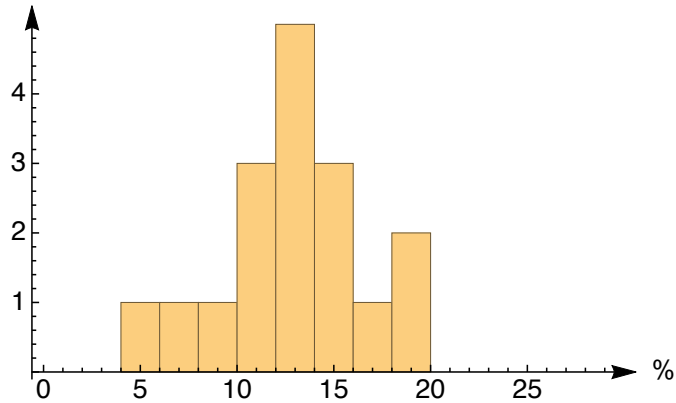

```
Mean[(ga - bh) / ga * 100]
```

12.9476

```
StandardDeviation[(ga - bh) / ga * 100]
```

3.73399

## 2p–2p decay of single core holes

```
bhGA224v126 := 55.284*^-4
```

```
bhGA223v125 := 45.358*^-4
```

```
bhGA222v124 := 33.070*^-4
```

```
bhGA221v123 := 19.731*^-4
```

```
bhGA220v122 := 7.698*^-4
```

```
bhGA214v116 := 66.278*^-4
```

```
bhGA213v115 := 53.548*^-4
```

```
bhGA212v114 := 38.330*^-4
```

```
bhGA211v113 := 22.495*^-4
```

```
bhGA210v112 := 8.670*^-4
```

```
bhGA204v106 := 77.901*^-4
```

```
bhGA203v105 := 61.854*^-4
```

```
bhGA202v104 := 43.571*^-4
```

```
bhGA201v103 := 25.306*^-4
```

```
bhGA200v102 := 9.682*^-4
```

```

bh = {bhGA224v126, bhGA223v125, bhGA222v124, bhGA221v123, bhGA220v122,
      bhGA214v116, bhGA213v115, bhGA212v114, bhGA211v113, bhGA210v112,
      bhGA204v106, bhGA203v105, bhGA202v104, bhGA201v103, bhGA200v102}

```

```

{0.0055284, 0.0045358, 0.003307, 0.0019731, 0.0007698,
 0.0066278, 0.0053548, 0.003833, 0.0022495, 0.000867,
 0.0077901, 0.0061854, 0.0043571, 0.0025306, 0.0009682}

```

```

ga = {GamA224v126, GamA223v125, GamA222v124, GamA221v123, GamA220v122,
      GamA214v116, GamA213v115, GamA212v114, GamA211v113, GamA210v112,
      GamA204v106, GamA203v105, GamA202v104, GamA201v103, GamA200v102}

```

```

{0.0061335, 0.0049967, 0.00363281, 0.00218344, 0.000863991,
 0.0067137, 0.00548109, 0.00399234, 0.00239789, 0.000950047,
 0.00876923, 0.00701997, 0.00502591, 0.00297236, 0.00113472}

```

```

(ga - bh) / ga * 100
{9.86549, 9.22409, 8.96854, 9.63342, 10.9018, 1.27947, 2.3041,
 3.99114, 6.18836, 8.74136, 11.1655, 11.8885, 13.3072, 14.8623, 14.675}

```

```

Histogram[(ga - bh) / ga * 100, histrange, AxesLabel -> {"%", "Number"},
  AxesStyle -> {{Arrowheads[Automatic], AbsoluteThickness[0.8]},
    {Arrowheads[Automatic], AbsoluteThickness[0.8]}},
  LabelStyle -> {FontFamily -> "Helvetica", FontSize -> 14}]

```

Number

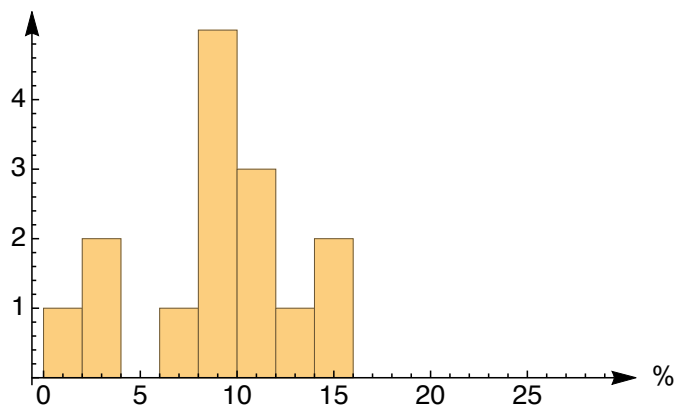

```

Mean[(ga - bh) / ga * 100]

```

9.13309

```

StandardDeviation[(ga - bh) / ga * 100]

```

4.14222

## 2s–2p decay of single core holes

```

bhGA215v126 := 24.448*^-4
bhGA214v125 := 24.002*^-4
bhGA213v124 := 22.507*^-4
bhGA212v123 := 19.682*^-4
bhGA211v122 := 15.163*^-4
bhGA210v121 := 8.606*^-4

bhGA205v116 := 14.150*^-4
bhGA204v115 := 13.773*^-4
bhGA203v114 := 12.832*^-4
bhGA202v113 := 11.129*^-4
bhGA201v112 := 8.442*^-4
bhGA200v111 := 4.716*^-4

bh = {bhGA215v126, bhGA214v125, bhGA213v124,
      bhGA212v123, bhGA211v122, bhGA210v121, bhGA205v116,
      bhGA204v115, bhGA203v114, bhGA202v113, bhGA201v112, bhGA200v111}
{0.0024448, 0.0024002, 0.0022507, 0.0019682, 0.0015163, 0.0008606,
 0.001415, 0.0013773, 0.0012832, 0.0011129, 0.0008442, 0.0004716}

ga = {GamA215v126, GamA214v125, GamA213v124,
      GamA212v123, GamA211v122, GamA210v121, GamA205v116,
      GamA204v115, GamA203v114, GamA202v113, GamA201v112, GamA200v111}
{0.00294607, 0.00288634, 0.00270171, 0.00235955, 0.00181318, 0.0010322,
 0.00180337, 0.00170873, 0.00158776, 0.00136361, 0.00103962, 0.000580309}

(ga - bh) / ga * 100
{17.0149, 16.8428, 16.6935, 16.5858, 16.3734,
 16.6247, 21.5358, 19.3963, 19.1817, 18.3858, 18.7973, 18.733}

```



```
Histogram[(ga - bh) / ga * 100, histrange, AxesLabel -> {"%", "Number"},
  AxesStyle -> {{Arrowheads[Automatic], AbsoluteThickness[0.8]},
    {Arrowheads[Automatic], AbsoluteThickness[0.8]}},
  LabelStyle -> {FontFamily -> "Helvetica", FontSize -> 14}]
```

Number

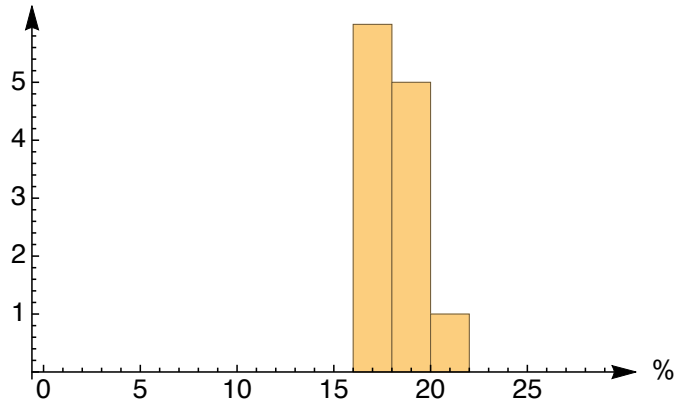

```
Mean[(ga - bh) / ga * 100]
```

18.0137

```
StandardDeviation[(ga - bh) / ga * 100]
```

1.58748

## 2s-2s decay of single core holes

```
bhGA206v126 := 8.334*^-4
```

```
bhGA205v125 := 9.393*^-4
```

```
bhGA204v124 := 10.701*^-4
```

```
bhGA203v123 := 12.220*^-4
```

```
bhGA202v122 := 13.827*^-4
```

```
bhGA201v121 := 15.388*^-4
```

```
bh = {bhGA206v126, bhGA205v125,
  bhGA204v124, bhGA203v123, bhGA202v122, bhGA201v121}
```

```
{0.0008334, 0.0009393, 0.0010701, 0.001222, 0.0013827, 0.0015388}
```

```
ga = {GamA206v126, GamA205v125,
  GamA204v124, GamA203v123, GamA202v122, GamA201v121}
```

```
{0.00106475, 0.00119848, 0.00135561, 0.00152685, 0.00171976, 0.00192445}
```

```
(ga - bh) / ga * 100
```

```
{21.7281, 21.6257, 21.0614, 19.9659, 19.5992, 20.0395}
```

```
Histogram[(ga - bh) / ga * 100, histrange, AxesLabel -> {"%", "Number"},
  AxesStyle -> {{Arrowheads[Automatic], AbsoluteThickness[0.8]},
    {Arrowheads[Automatic], AbsoluteThickness[0.8]}},
  LabelStyle -> {FontFamily -> "Helvetica", FontSize -> 14}]
```

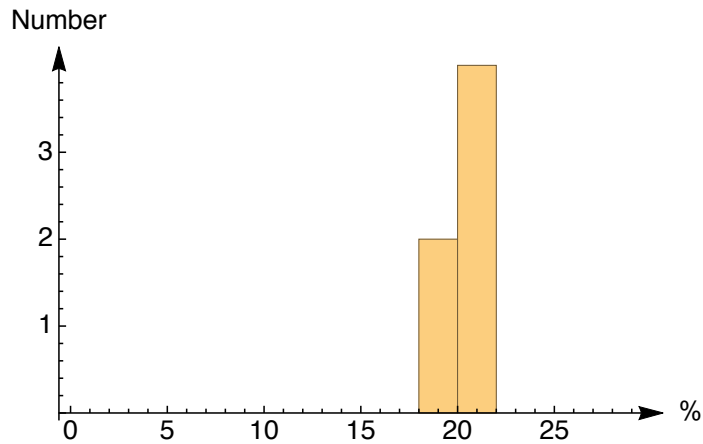

```
Mean[(ga - bh) / ga * 100]
```

```
20.67
```

```
StandardDeviation[(ga - bh) / ga * 100]
```

```
0.919339
```

## Total width of double core holes

```
bhGA026 := 129.860 * 2^-4
```

```
bhGA025 := 112.160 * 2^-4
```

```
bhGA024 := 91.009 * 2^-4
```

```
bhGA023 := 68.309 * 2^-4
```

```
bhGA022 := 46.790 * 2^-4
```

```
bhGA021 := 29.702 * 2^-4
```

```
bhGA016 := 119.128 * 2^-4
```

```
bhGA015 := 96.478 * 2^-4
```

```
bhGA014 := 70.982 * 2^-4
```

```
bhGA013 := 45.172 * 2^-4
```

```
bhGA012 := 22.201 * 2^-4
```

```
bhGA011 := 5.872 * 2^-4
```

```
bhGA006 := 116.220 * 2^-4
```

```
bhGA005 := 89.805 * 2^-4
```

```
bhGA004 := 61.849 * 2^-4
```

```
bhGA003 := 35.184 * 2^-4
```

```
bhGA002 := 13.161 * 2^-4
```

```

bh = {bhGA026, bhGA025, bhGA024, bhGA023, bhGA022, bhGA021,
      bhGA016, bhGA015, bhGA014, bhGA013, bhGA012, bhGA011,
      bhGA006, bhGA005, bhGA004, bhGA003, bhGA002}

{0.025972, 0.022432, 0.0182018, 0.0136618, 0.009358,
 0.0059404, 0.0238256, 0.0192956, 0.0141964, 0.0090344, 0.0044402,
 0.0011744, 0.023244, 0.017961, 0.0123698, 0.0070368, 0.0026322}

ga = {GamATot026, GamATot025, GamATot024, GamATot023, GamATot022, GamATot021,
      GamATot016, GamATot015, GamATot014, GamATot013, GamATot012, GamATot011,
      GamATot006, GamATot005, GamATot004, GamATot003, GamATot002}

{0.0282568, 0.0243976, 0.0199244, 0.0150109, 0.0102734,
 0.0064139, 0.025379, 0.0206334, 0.0153577, 0.00991768, 0.00495902,
 0.00129078, 0.0239298, 0.018492, 0.0129503, 0.0074571, 0.00278219}

(ga - bh) / ga * 100
{8.08594, 8.05645, 8.64554, 8.98723, 8.91066, 7.3824, 6.12077, 6.48353, 7.5618,
 8.90612, 10.4621, 9.01625, 2.86588, 2.87151, 4.48252, 5.63624, 5.39108}

```

```

Histogram[(ga - bh) / ga * 100, histrange, AxesLabel -> {"%", "Number"},
  AxesStyle -> {{Arrowheads[Automatic], AbsoluteThickness[0.8]},
    {Arrowheads[Automatic], AbsoluteThickness[0.8]}},
  LabelStyle -> {FontFamily -> "Helvetica", FontSize -> 14}]

```

Number

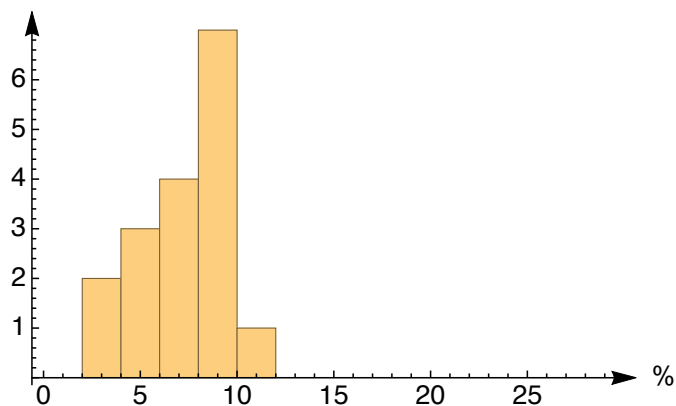

```
Mean[(ga - bh) / ga * 100]
```

7.05095

```
StandardDeviation[(ga - bh) / ga * 100]
```

2.21736

## 2p–2p decay of double core holes

```

bhGA124v026 := 85.925 * 2*^-4
bhGA123v025 := 67.900 * 2*^-4
bhGA122v024 := 47.598 * 2*^-4
bhGA121v023 := 27.310 * 2*^-4
bhGA120v022 := 10.233 * 2*^-4

bhGA114v016 := 99.936 * 2*^-4
bhGA113v015 := 78.032 * 2*^-4
bhGA112v014 := 54.054 * 2*^-4
bhGA111v013 := 30.757 * 2*^-4
bhGA110v012 := 11.475 * 2*^-4

bhGA104v006 := 116.220 * 2*^-4
bhGA103v005 := 89.805 * 2*^-4
bhGA102v004 := 61.849 * 2*^-4
bhGA101v003 := 35.184 * 2*^-4
bhGA100v002 := 13.161 * 2*^-4

bh = {bhGA124v026, bhGA123v025, bhGA122v024, bhGA121v023, bhGA120v022,
      bhGA114v016, bhGA113v015, bhGA112v014, bhGA111v013, bhGA110v012,
      bhGA104v006, bhGA103v005, bhGA102v004, bhGA101v003, bhGA100v002}
{0.017185, 0.01358, 0.0095196, 0.005462, 0.0020466,
 0.0199872, 0.0156064, 0.0108108, 0.0061514, 0.002295,
 0.023244, 0.017961, 0.0123698, 0.0070368, 0.0026322}

ga = {GamA124v026, GamA123v025, GamA122v024, GamA121v023, GamA120v022,
      GamA114v016, GamA113v015, GamA112v014, GamA111v013, GamA110v012,
      GamA104v006, GamA103v005, GamA102v004, GamA101v003, GamA100v002}
{0.0185137, 0.0146864, 0.0104446, 0.00611762, 0.002377,
 0.0210425, 0.0165259, 0.0116148, 0.00676088, 0.00260136,
 0.0239298, 0.018492, 0.0129503, 0.0074571, 0.00278219}

(ga - bh) / ga * 100
{7.17685, 7.5335, 8.85625, 10.7169, 13.8999, 5.01509, 5.56399,
 6.9222, 9.0148, 11.7769, 2.86588, 2.87151, 4.48252, 5.63624, 5.39108}

```

```
Histogram[(ga - bh) / ga * 100, histrange, AxesLabel -> {"%", "Number"},
  AxesStyle -> {{Arrowheads[Automatic], AbsoluteThickness[0.8]},
    {Arrowheads[Automatic], AbsoluteThickness[0.8]}},
  LabelStyle -> {FontFamily -> "Helvetica", FontSize -> 14}]
```

Number

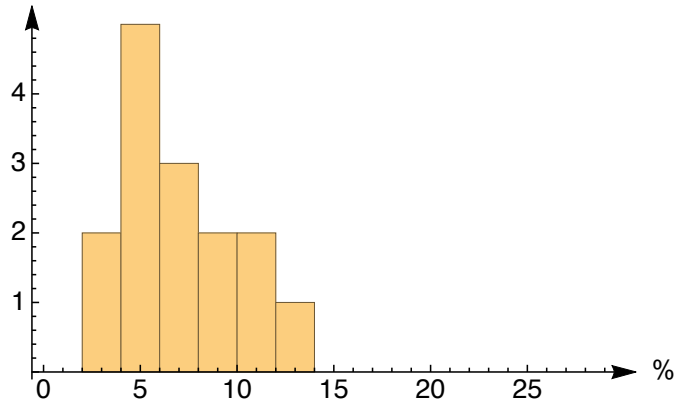

```
Mean[(ga - bh) / ga * 100]
```

7.18157

```
StandardDeviation[(ga - bh) / ga * 100]
```

3.19037

## 2s–2p decay of double core holes

```
bhGA115v026 := 33.699 * 2^-4
```

```
bhGA114v025 := 32.558 * 2^-4
```

```
bhGA113v024 := 30.020 * 2^-4
```

```
bhGA112v023 := 25.753 * 2^-4
```

```
bhGA111v022 := 19.398 * 2^-4
```

```
bhGA110v021 := 10.772 * 2^-4
```

```
bhGA105v016 := 19.192 * 2^-4
```

```
bhGA104v015 := 18.446 * 2^-4
```

```
bhGA103v014 := 16.928 * 2^-4
```

```
bhGA102v013 := 14.415 * 2^-4
```

```
bhGA101v012 := 10.726 * 2^-4
```

```
bhGA100v011 := 5.872 * 2^-4
```

```
bh = {bhGA115v026, bhGA114v025, bhGA113v024,
  bhGA112v023, bhGA111v022, bhGA110v021, bhGA105v016,
  bhGA104v015, bhGA103v014, bhGA102v013, bhGA101v012, bhGA100v011}
{0.0067398, 0.0065116, 0.006004, 0.0051506, 0.0038796, 0.0021544,
  0.0038384, 0.0036892, 0.0033856, 0.002883, 0.0021452, 0.0011744}
```

```
ga = {GamA115v026, GamA114v025, GamA113v024,
      GamA112v023, GamA111v022, GamA110v021, GamA105v016,
      GamA104v015, GamA103v014, GamA102v013, GamA101v012, GamA100v011}
{0.00738408, 0.0070738, 0.00652319, 0.00559174, 0.00421077, 0.00234648,
 0.00433649, 0.00410747, 0.00374292, 0.0031568, 0.00235766, 0.00129078}
```

```
(ga - bh) / ga * 100
{8.72526, 7.94764, 7.95914, 7.88914, 7.86483,
 8.18588, 11.486, 10.1832, 9.54656, 8.67334, 9.01148, 9.01625}

Histogram[(ga - bh) / ga * 100, histrange, AxesLabel -> {"%", "Number"},
  AxesStyle -> {{Arrowheads[Automatic], AbsoluteThickness[0.8]},
    {Arrowheads[Automatic], AbsoluteThickness[0.8]}},
  LabelStyle -> {FontFamily -> "Helvetica", FontSize -> 14}]
```

Number

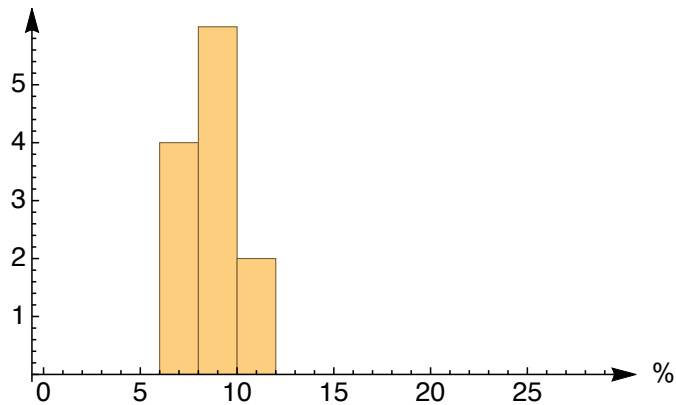

```
Mean[(ga - bh) / ga * 100]
```

8.87406

```
StandardDeviation[(ga - bh) / ga * 100]
```

1.09741

## 2s–2s decay of double core holes

```
bhGA106v026 := 10.239 * 2^-4
bhGA105v025 := 11.698 * 2^-4
bhGA104v024 := 13.390 * 2^-4
bhGA103v023 := 15.246 * 2^-4
bhGA102v022 := 17.160 * 2^-4
bhGA101v021 := 18.930 * 2^-4

bh = {bhGA106v026, bhGA105v025,
      bhGA104v024, bhGA103v023, bhGA102v022, bhGA101v021}
{0.0020478, 0.0023396, 0.002678, 0.0030492, 0.003432, 0.003786}
```

```
ga = {GamA106v026, GamA105v025,
      GamA104v024, GamA103v023, GamA102v022, GamA101v021}
{0.00235905, 0.00263738, 0.00295658, 0.0033015, 0.00368566, 0.00406742}
```

```
(ga - bh) / ga * 100
{13.1939, 11.2908, 9.42237, 7.64198, 6.88235, 6.91888}
```

```
Histogram[(ga - bh) / ga * 100, histrange, AxesLabel → {"%", "Number"},
  AxesStyle → {{Arrowheads[Automatic], AbsoluteThickness[0.8]},
    {Arrowheads[Automatic], AbsoluteThickness[0.8]}},
  LabelStyle → {FontFamily → "Helvetica", FontSize → 14}]
```

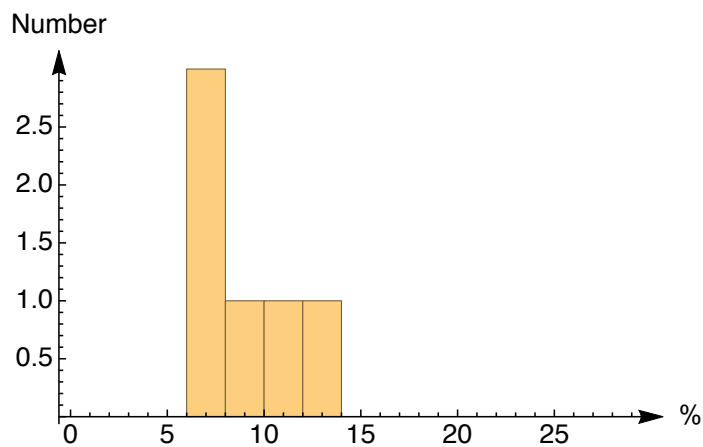

```
Mean[(ga - bh) / ga * 100]
```

```
9.22503
```

```
StandardDeviation[(ga - bh) / ga * 100]
```

```
2.58342
```

## Bhalla's radiative widths

### Single core holes

```

bhGR126 := 1.436*^-4
bhGR125 := 1.339*^-4
bhGR124 := 1.194*^-4
bhGR123 := 0.994*^-4
bhGR122 := 0.732*^-4
bhGR121 := 0.401*^-4

```

```

bhGR116 := 1.596*^-4
bhGR115 := 1.479*^-4
bhGR114 := 1.312*^-4
bhGR113 := 1.087*^-4
bhGR112 := 0.796*^-4
bhGR111 := 0.434*^-4

```

```

bhGR106 := 1.762*^-4
bhGR105 := 1.625*^-4
bhGR104 := 1.435*^-4
bhGR103 := 1.183*^-4
bhGR102 := 0.868*^-4
bhGR101 := 0.509*^-4

```

```

bh = {bhGR126, bhGR125, bhGR124, bhGR123, bhGR122, bhGR121,
      bhGR116, bhGR115, bhGR114, bhGR113, bhGR112, bhGR111,
      bhGR106, bhGR105, bhGR104, bhGR103, bhGR102, bhGR101}

```

```

{0.0001436, 0.0001339, 0.0001194, 0.0000994, 0.0000732, 0.0000401,
 0.0001596, 0.0001479, 0.0001312, 0.0001087, 0.0000796, 0.0000434,
 0.0001762, 0.0001625, 0.0001435, 0.0001183, 0.0000868, 0.0000509}

```

```

ga = {GamRTot126, GamRTot125, GamRTot124, GamRTot123, GamRTot122, GamRTot121,
      GamRTot116, GamRTot115, GamRTot114, GamRTot113, GamRTot112, GamRTot111,
      GamRTot106, GamRTot105, GamRTot104, GamRTot103, GamRTot102, GamRTot101}

```

```

{0.000171731, 0.000160333, 0.000143211, 0.000119525, 0.0000883876, 0.0000488718,
 0.000156805, 0.000147643, 0.000132924, 0.000111757, 0.0000832074, 0.0000462994,
 0.000200621, 0.00018672, 0.000166325, 0.00013847, 0.000102162, 0.0000563657}

```

```

(ga - bh) / ga * 100

```

```

{16.3809, 16.4864, 16.6266, 16.8375, 17.183, 17.9486, -1.7822, -0.174387, 1.29677,
 2.73498, 4.33541, 6.26238, 12.1725, 12.9711, 13.7231, 14.5665, 15.0367, 9.69688}

```



```
Histogram[(ga - bh) / ga * 100, histex, AxesLabel -> {"%", "Number"},
  AxesStyle -> {{Arrowheads[Automatic], AbsoluteThickness[0.8]},
    {Arrowheads[Automatic], AbsoluteThickness[0.8]}},
  LabelStyle -> {FontFamily -> "Helvetica", FontSize -> 14}]
```

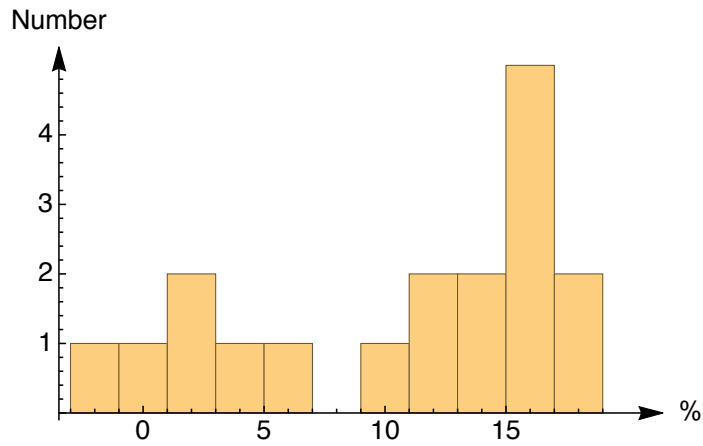

```
Mean[(ga - bh) / ga * 100]
```

```
10.6835
```

```
StandardDeviation[(ga - bh) / ga * 100]
```

```
6.73211
```

## Double core holes

```
bhGR026 := 2.363 * 2^-4
```

```
bhGR025 := 2.162 * 2^-4
```

```
bhGR024 := 1.893 * 2^-4
```

```
bhGR023 := 1.547 * 2^-4
```

```
bhGR022 := 1.117 * 2^-4
```

```
bhGR021 := 0.599 * 2^-4
```

```
bhGR016 := 2.611 * 2^-4
```

```
bhGR015 := 2.381 * 2^-4
```

```
bhGR014 := 2.078 * 2^-4
```

```
bhGR013 := 1.693 * 2^-4
```

```
bhGR012 := 1.219 * 2^-4
```

```
bhGR011 := 0.651 * 2^-4
```

```
bhGR006 := 2.936 * 2^-4
```

```
bhGR005 := 2.675 * 2^-4
```

```
bhGR004 := 2.336 * 2^-4
```

```
bhGR003 := 1.907 * 2^-4
```

```
bhGR002 := 1.415 * 2^-4
```

```
bhGR001 := 0.758 * 2^-4
```

```

bh = {bhGR026, bhGR025, bhGR024, bhGR023, bhGR022, bhGR021,
      bhGR016, bhGR015, bhGR014, bhGR013, bhGR012, bhGR011,
      bhGR006, bhGR005, bhGR004, bhGR003, bhGR002, bhGR001}

{0.0004726, 0.0004324, 0.0003786, 0.0003094, 0.0002234, 0.0001198,
 0.0005222, 0.0004762, 0.0004156, 0.0003386, 0.0002438, 0.0001302,
 0.0005872, 0.000535, 0.0004672, 0.0003814, 0.000283, 0.0001516}

ga = {GamRTot026, GamRTot025, GamRTot024, GamRTot023, GamRTot022, GamRTot021,
      GamRTot016, GamRTot015, GamRTot014, GamRTot013, GamRTot012, GamRTot011,
      GamRTot006, GamRTot005, GamRTot004, GamRTot003, GamRTot002, GamRTot001}

{0.000505777, 0.000463927, 0.000407528, 0.000334815, 0.000243958, 0.000133031,
 0.000520806, 0.000480957, 0.000424936, 0.000350832, 0.000256677, 0.000140442,
 0.000578887, 0.000530309, 0.000465267, 0.000381798, 0.000277857, 0.000151332}

(ga - bh) / ga * 100
{6.55961, 6.7957, 7.09843, 7.59077, 8.42686, 9.9458,
 -0.267678, 0.989101, 2.19704, 3.4865, 5.0169, 7.2925,
 -1.43611, -0.884564, -0.415422, 0.104336, -1.85096, -0.177094}

```

```

Histogram[(ga - bh) / ga * 100, histex, AxesLabel → {"%", "Number"},
  AxesStyle → {{Arrowheads[Automatic], AbsoluteThickness[0.8]},
    {Arrowheads[Automatic], AbsoluteThickness[0.8]}},
  LabelStyle → {FontFamily → "Helvetica", FontSize → 14}]

```

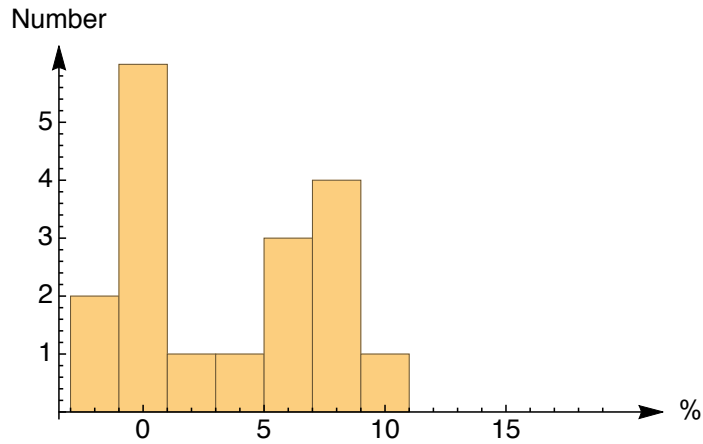

```
Mean[(ga - bh) / ga * 100]
```

```
3.35954
```

```
StandardDeviation[(ga - bh) / ga * 100]
```

```
3.96202
```

## Bhalla's fluorescence yields

The fluorescence yield is only approximately determined using Eq. (1) from Ref. [2]. See Ref. [2] for details on probabilistically averaging over fine-structure resolved fluorescence yields.

## Total fluorecence yield of single core holes

```

bhyi126 := 0.0160
bhyi125 := 0.0167
bhyi124 := 0.0177
bhyi123 := 0.0189
bhyi122 := 0.0196
bhyi121 := 0.0164

bhyi116 := 0.0195
bhyi115 := 0.0215
bhyi114 := 0.0250
bhyi113 := 0.0313
bhyi112 := 0.0445
bhyi111 := 0.0843

bhyi106 := 0.0221
bhyi105 := 0.0256
bhyi104 := 0.0319
bhyi103 := 0.0447
bhyi102 := 0.0823

bh = {{bhyi126, bhyi116, bhyi106}, {bhyi125, bhyi115, bhyi105},
      {bhyi124, bhyi114, bhyi104}, {bhyi123, bhyi113, bhyi103},
      {bhyi122, bhyi112, bhyi102}, {bhyi121, bhyi111, 1}}
{{0.016, 0.0195, 0.0221}, {0.0167, 0.0215, 0.0256}, {0.0177, 0.025, 0.0319},
 {0.0189, 0.0313, 0.0447}, {0.0196, 0.0445, 0.0823}, {0.0164, 0.0843, 1}}

ga = {{GamATot126, GamATot116, GamATot106},
      {GamATot125, GamATot115, GamATot105}, {GamATot124, GamATot114, GamATot104},
      {GamATot123, GamATot113, GamATot103}, {GamATot122, GamATot112, GamATot102},
      {GamATot121, GamATot111, 0}} * HartreeTomeV
{{276.041, 231.761, 238.623}, {247.121, 195.645, 191.023},
 {209.259, 151.842, 136.762}, {165.169, 102.356, 80.882},
 {119.647, 54.1416, 30.8773}, {80.4545, 15.791, 0.}}

gr = {{GamRTot126, GamRTot116, GamRTot106},
      {GamRTot125, GamRTot115, GamRTot105}, {GamRTot124, GamRTot114, GamRTot104},
      {GamRTot123, GamRTot113, GamRTot103}, {GamRTot122, GamRTot112, GamRTot102},
      {GamRTot121, GamRTot111, GamRTot101}} * HartreeTomeV
{{4.67304, 4.26689, 5.45916}, {4.36289, 4.01756, 5.0809},
 {3.89697, 3.61704, 4.52593}, {3.25244, 3.04105, 3.76797},
 {2.40515, 2.26419, 2.77996}, {1.32987, 1.25987, 1.53379}}

```

```

relerr = (gr / (ga + gr) - bh) / (gr / (ga + gr)) * 100
{{3.88642, -7.86654, 1.18976}, {3.73856, -6.84959, 1.19339},
 {3.18478, -7.44929, 0.416478}, {2.13015, -8.47951, -0.421659},
 {0.537841, -10.8591, 0.358638}, {-0.856829, -14.0901, -1.11022 × 10-14}}

```

```

BarChart[relerr, PlotRange → All,
 ChartLabels → {{6, 5, 4, 3, 2, 1}, None}, AxesLabel → {"2p^n", "ω"},
 AxesStyle → {{Arrowheads[Automatic], AbsoluteThickness[0.6]},
 {Arrowheads[Automatic], AbsoluteThickness[0.6]}},
 LabelStyle → {FontFamily → "Helvetica"}]

```

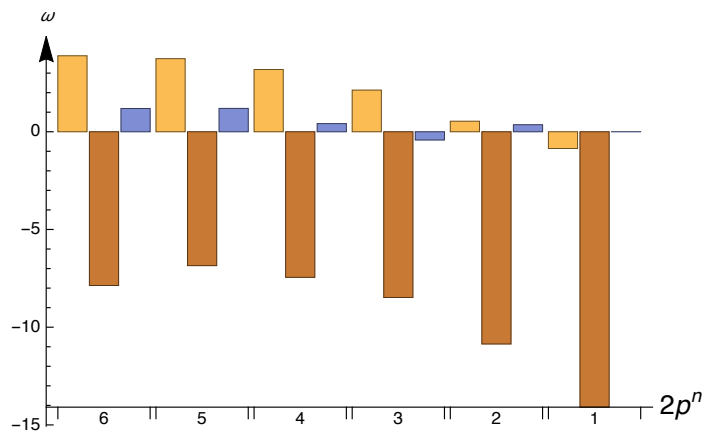

```
Mean[Flatten[relerr]]
```

```
-2.23537
```

```
StandardDeviation[Flatten[relerr]]
```

```
5.48154
```

## Total fluorescence yield of double core holes

```

bhyi026 := 0.0179
bhyi025 := 0.0189
bhyi024 := 0.0204
bhyi023 := 0.0221
bhyi022 := 0.0233
bhyi021 := 0.0198

bhyi016 := 0.0214
bhyi015 := 0.0241
bhyi014 := 0.0284
bhyi013 := 0.0361
bhyi012 := 0.0520
bhyi011 := 0.0998

bhyi006 := 0.0246
bhyi005 := 0.0289
bhyi004 := 0.0364
bhyi003 := 0.0514
bhyi002 := 0.0971

bh = {{bhyi026, bhyi016, bhyi006}, {bhyi025, bhyi015, bhyi005},
      {bhyi024, bhyi014, bhyi004}, {bhyi023, bhyi013, bhyi003},
      {bhyi022, bhyi012, bhyi002}, {bhyi021, bhyi011, 1}}
{{0.0179, 0.0214, 0.0246}, {0.0189, 0.0241, 0.0289}, {0.0204, 0.0284, 0.0364},
 {0.0221, 0.0361, 0.0514}, {0.0233, 0.052, 0.0971}, {0.0198, 0.0998, 1}}

ga = {{GamATot026, GamATot016, GamATot006},
      {GamATot025, GamATot015, GamATot005}, {GamATot024, GamATot014, GamATot004},
      {GamATot023, GamATot013, GamATot003}, {GamATot022, GamATot012, GamATot002},
      {GamATot021, GamATot011, 0}} * HartreeTomeV
{{768.907, 690.597, 651.163}, {663.892, 561.463, 503.193},
 {542.17, 417.905, 352.396}, {408.466, 269.874, 202.918},
 {279.554, 134.942, 75.7072}, {174.531, 35.1239, 0.}}

gr = {{GamRTot026, GamRTot016, GamRTot006},
      {GamRTot025, GamRTot015, GamRTot005}, {GamRTot024, GamRTot014, GamRTot004},
      {GamRTot023, GamRTot013, GamRTot003}, {GamRTot022, GamRTot012, GamRTot002},
      {GamRTot021, GamRTot011, GamRTot001}} * HartreeTomeV
{{13.7629, 14.1719, 15.7523}, {12.6241, 13.0875, 14.4304},
 {11.0894, 11.5631, 12.6606}, {9.11078, 9.54662, 10.3893},
 {6.63844, 6.98454, 7.56087}, {3.61996, 3.82161, 4.11795}}

```

```

relerr = (gr / (ga + gr) - bh) / (gr / (ga + gr)) * 100
{{{-1.79401, -6.42268, -4.15057}}, {-1.28369, -5.80054, -3.66497}},
{{{-1.77721, -5.48116, -4.95618}}, {-1.29157, -5.66127, -5.53198}},
{{{-0.44972, -5.66432, -6.93652}}, {2.55712, -1.70477, 0.}}}

```

```

BarChart[relerr, PlotRange → All,
  ChartLabels → {{6, 5, 4, 3, 2, 1}, None}, AxesLabel → {"2p^n", "ω"},
  AxesStyle → {{Arrowheads[Automatic], AbsoluteThickness[0.6]},
    {Arrowheads[Automatic], AbsoluteThickness[0.6]}},
  LabelStyle → {FontFamily → "Helvetica"}]

```

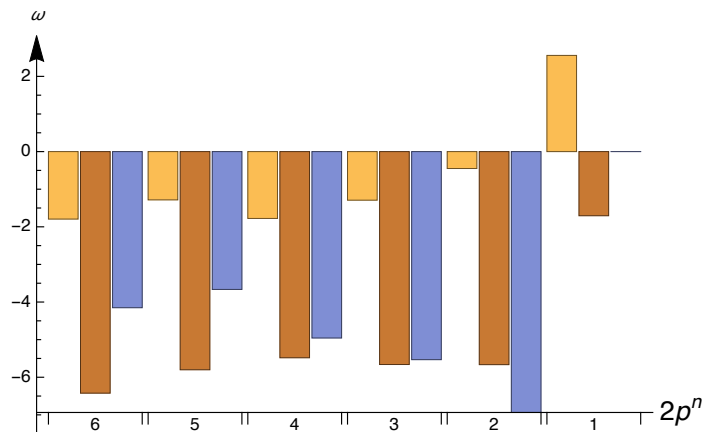

```
Mean[Flatten[relerr]]
```

```
-3.33411
```

```
StandardDeviation[Flatten[relerr]]
```

```
2.68177
```

## References

- [1] C. P. Bhalla, N. O. Folland, M. A. Hein, *Theoretical K-shell Auger rates, transition energies, and fluorescence yields for multiply ionized neon*, Phys. Rev. A **8**, 649 (1973), <http://doi.org/10.1103/PhysRevA.8.649>.
- [2] C. P. Bhalla, *Theoretical fluorescence yields for neon*, Phys. Rev. A **12**, 122 (1975), <http://doi.org/10.1103/PhysRevA.12.122>.
