# Supplementary material for: Neon in ultrashort and intense x rays from free electron lasers
Source: arXiv:1705.07521 ancillary file (2022-11-07)
Supplement: Supplementary file 2 [file neon_fluorescence.pdf]

```
In[54]:= Get["NeonRateEquations.m", Path -> NotebookDirectory[]]
```

```
In[55]:= HartreeToeV := 27.2113845  
eVToHartree := 1/HartreeToeV  
JouleToHartree := 2.29371269*^17  
MilliJouleToHartree := 1*^-3 * JouleToHartree  
BohrToAngstroem := 0.5291772083  
AngstroemToBohr := 1/BohrToAngstroem  
MicrometerToBohr := 1*^4 * AngstroemToBohr  
BohrToMicrometer := 1/MicrometerToBohr  
t0ToSecond := 24.18884326505*^-18  
t0ToFemtoSecond := 24.18884326505*^-3  
FemtoSecondTot0 := 1/t0ToFemtoSecond  
crossSectionAUtoBarn := 1*^8 * BohrToAngstroem^2  
crossSectionAUtocm2 := crossSectionAUtoBarn * 1*^-24  
crossSectioncm2toAU := 1/crossSectionAUtocm2
```

```
In[69]:= neginfinity := -10 000 / t0ToFemtoSecond  
posinfinity := 10 000 / t0ToFemtoSecond
```

# Fluorescence from a neon atom in LCLS radiation

Christian Buth, 11 May 2017

Theoretische Chemie, Physikalisch-Chemisches Institut, Ruprecht-Karls-Universität Heidelberg, Im Neuenheimer Feld 229, 69120 Heidelberg, Germany

---

## LCLS x-ray pulse

### Temporal profile

LCLS x-ray transmission:

```
In[71]:= optdamp := 0.5
```

LCLS pulse energy:

```
In[72]:= pulseenergy := optdamp * 1.2 * MilliJouleToHartree
```

LCLS x-ray energy:

```
In[73]:= omegaX := 1200 * eVToHartree
```

LCLS FWHM pulse duration:

```
In[74]:= tauX := 100 * FemtoSecondTot0
```

LCLS peak a fluence:

```
In[75]:= J0X := 2 * Sqrt[Log[2] / Pi] * 8 * 10^11 / (1 * 10^4 / BohrToAngstroem)^2 / tauX
```

Gaussian x-ray flux pulse shape (See Eq. (7) in Ref. [1]):

```
In[76]:= jxgaussian[J0Xj_, tX_, t_] :=
  J0Xj * Exp[-4 * Log[2] * (t/tX)^2] * UnitStep[t + 2 * tX] * UnitStep[2 * tX - t]
flux[t_] := jxgaussian[J0X, tauX, t]
```

```
In[78]:= Plot[{flux[t/t0ToFemtoSecond], 1/2 * flux[0] *
  UnitStep[t/t0ToFemtoSecond + tauX/2] * UnitStep[tauX/2 - t/t0ToFemtoSecond]},
  {t, -200, 200}, PlotStyle -> {{Red, Thick}, {Green, Thick}}, PlotRange -> All]
```

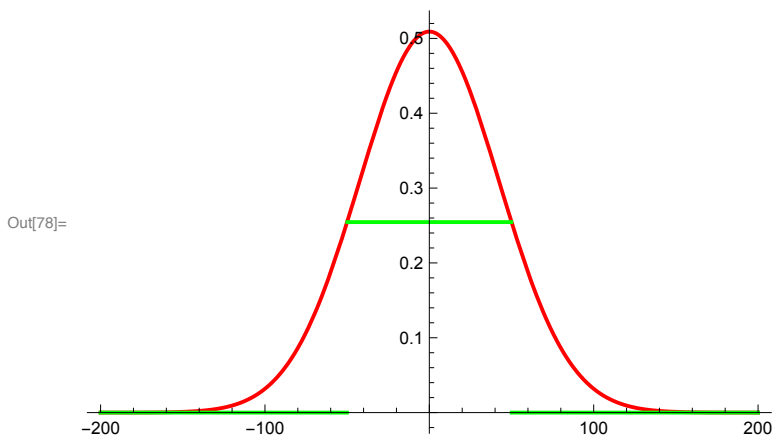

## Crater profile

FWHM of the crater profile:

```
In[79]:= rhoXx:=2*MicrometerToBohr
rhoYy:=1*MicrometerToBohr
```

The crater is normalized to unity with respect to an integration over the whole xy plane:

```
In[81]:= craterX[rx_] := 1/rhoXx/Sqrt[Pi/Log[16]] * Exp[-4*Log[2] * (rx/rhoXx)^2]
craterY[ry_] := 1/rhoYy/Sqrt[Pi/Log[16]] * Exp[-4*Log[2] * (ry/rhoYy)^2]
crater[rx_, ry_] := craterX[rx] * craterY[ry]
```

Number of radial integration points for the crater integration:

```
In[84]:= nintdata:=100
```

## Fluence profile

Number of x-ray photons for “monochromatic” light pulses:

```
In[85]:= numXRays[pulseenergy_,photonenergy_]:=pulseenergy/photonenergy
```

X-ray fluence, i.e., the number of photos per squaremeter:

```
In[86]:= fluence[pulseenergy_,photonenergy_,rx_,ry_]:=numXRays[pulseenergy,photonenergy]*crater
```

```
In[87]:= peakfluence[pulseenergy_,photonenergy_]:=fluence[pulseenergy,photonenergy,0,0]
```

The peak x-ray flux at a point in the beam area:

```
In[88]:= J0Xfun[pulseenergy_,photonenergy_,tauX_,rx_,ry_]:=2*Sqrt[Log[2]/Pi]/tauX*fluence[pulse
```

Gaussian x-ray flux pluse shape:

```
In[89]:= jxgaussian[J0Xj_,tX_,t_]:=J0Xj*Exp[-4*Log[2]*(t/tX)^2]*UnitStep[t+2*tX]*UnitStep[2*tX-
```

## Radiative decay of certain configurations

```
In[90]:= idxconfig = <|Table[configurations[[i]] → i, {i, 1, Length[configurations]}]|>
```

```
Out[90]= <| 226 → 1, 225 → 2, 216 → 3, 126 → 4, 224 → 5, 215 → 6, 206 → 7, 125 → 8,
116 → 9, 026 → 10, 223 → 11, 214 → 12, 205 → 13, 124 → 14, 115 → 15, 106 → 16,
025 → 17, 016 → 18, 222 → 19, 213 → 20, 204 → 21, 123 → 22, 114 → 23, 105 → 24,
024 → 25, 015 → 26, 006 → 27, 221 → 28, 212 → 29, 203 → 30, 122 → 31, 113 → 32,
104 → 33, 023 → 34, 014 → 35, 005 → 36, 220 → 37, 211 → 38, 202 → 39, 121 → 40,
112 → 41, 103 → 42, 022 → 43, 013 → 44, 004 → 45, 210 → 46, 201 → 47, 120 → 48,
111 → 49, 102 → 50, 021 → 51, 012 → 52, 003 → 53, 200 → 54, 110 → 55, 101 → 56,
020 → 57, 011 → 58, 002 → 59, 100 → 60, 010 → 61, 001 → 62, 000 → 63 |>
```

```
In[91]:= terminalcfg = Map[idxconfig,
{"226", "225", "224", "223", "222", "221", "220", "210", "200", "100", "000"}]
```

```
Out[91]= {1, 2, 5, 11, 19, 28, 37, 46, 54, 60, 63}
```

## Configurations which decay exclusively radiatively

```
In[92]:= Table[If[!existsGamAtot[[i]] && existsGamRtot[[i]], configurations[[i]], ""],
{i, 1, Length[existsGamAtot]}]
```

```
Out[92]= {, , 216, , , 215, 206, , , , 214, 205, , , , , 213, 204, , , , , , 212, 203, ,
, , , , , 211, 202, , , , , , 201, , , , , , 110, 101, , , , 010, 001, }
```

```
In[93]:= {GamRTot216, GamRTot215, GamRTot206, GamRTot214, GamRTot205, GamRTot213,
          GamRTot204, GamRTot212, GamRTot203, GamRTot211, GamRTot202, GamRTot201,
          GamRTot110, GamRTot101, GamRTot010, GamRTot001} * posinfinity
```

```
Out[93]= {0.201701, 0.161539, 0.191075, 0.115628, 0.147279,
          0.071781, 0.0989526, 0.0360639, 0.0556178, 0.0119578, 0.0237782,
          0.00585518, 7.44227 × 10-8, 23.3024, 2.51004 × 10-7, 62.5627}
```

```
In[94]:= 1 / GamRTot110 * t0ToSecond * 1*^6
```

```
Out[94]= 134.368
```

```
In[95]:= {GamATot126, GamATot125, GamATot124, GamATot123, GamATot122, GamATot121,
          GamATot116, GamATot115, GamATot114, GamATot113, GamATot112, GamATot111,
          GamATot106, GamATot105, GamATot104, GamATot103, GamATot102} * posinfinity
```

```
Out[95]= {4193.8, 3754.43, 3179.21, 2509.36, 1817.75, 1222.32, 3521.07, 2972.37, 2306.89,
          1555.06, 822.556, 239.908, 3625.32, 2902.15, 2077.78, 1228.81, 469.109}
```

```
In[96]:= 1 / GamATot111 * t0ToFemtoSecond
```

```
Out[96]= 41.6827
```

## Decay matrix with exclusively radiative decay widths

```
In[97]:= matRad:=SparseArray[{
  (* No core holes *)
  {idxconfig["216"],idxconfig["216"]}→-GamRTot216,{idxconfig["225"],idxconfig["216"]}→Ga
  {idxconfig["215"],idxconfig["215"]}→-GamRTot215,{idxconfig["224"],idxconfig["215"]}→Ga
  {idxconfig["206"],idxconfig["206"]}→-GamRTot206,{idxconfig["215"],idxconfig["206"]}→Ga
  {idxconfig["214"],idxconfig["214"]}→-GamRTot214,{idxconfig["223"],idxconfig["214"]}→Ga
  {idxconfig["205"],idxconfig["205"]}→-GamRTot205,{idxconfig["214"],idxconfig["205"]}→Ga
  {idxconfig["213"],idxconfig["213"]}→-GamRTot213,{idxconfig["222"],idxconfig["213"]}→Ga
  {idxconfig["204"],idxconfig["204"]}→-GamRTot204,{idxconfig["213"],idxconfig["204"]}→Ga
  {idxconfig["212"],idxconfig["212"]}→-GamRTot212,{idxconfig["221"],idxconfig["212"]}→Ga
  {idxconfig["203"],idxconfig["203"]}→-GamRTot203,{idxconfig["212"],idxconfig["203"]}→Ga
  {idxconfig["211"],idxconfig["211"]}→-GamRTot211,{idxconfig["220"],idxconfig["211"]}→Ga
  {idxconfig["202"],idxconfig["202"]}→-GamRTot202,{idxconfig["211"],idxconfig["202"]}→Ga
  {idxconfig["201"],idxconfig["201"]}→-GamRTot201,{idxconfig["210"],idxconfig["201"]}→Ga

  (* Single core holes *)
  {idxconfig["110"],idxconfig["110"]}→-GamRTot110,{idxconfig["200"],idxconfig["110"]}→Ga
  {idxconfig["101"],idxconfig["101"]}→-GamRTot101,{idxconfig["200"],idxconfig["101"]}→Ga
  {idxconfig["110"],idxconfig["101"]}→GamR110v101,

  (* Double core holes *)
  {idxconfig["010"],idxconfig["010"]}→-GamRTot010,{idxconfig["100"],idxconfig["010"]}→Ga
  {idxconfig["001"],idxconfig["001"]}→-GamRTot001,{idxconfig["100"],idxconfig["001"]}→Ga
  {idxconfig["010"],idxconfig["001"]}→GamR010v001,
  {Length[configurations],Length[configurations]}]}
```

```
In[98]:= Chop[Transpose[Eigenvectors[matRad]].DiagonalMatrix[Eigenvalues[matRad]].  
Inverse[Transpose[Eigenvectors[matRad]]] - matRad] == SparseArray[{},  
{Length[configurations], Length[configurations]}]  
Out[98]:= True
```

## Probabilities at infinite time

```
In[99]:= eigval = Eigenvalues[matRad]
```

```
Out[99]= { -0.000151332, -0.0000563657, -4.87891 × 10-7, -4.62189 × 10-7,  
-3.90745 × 10-7, -3.56251 × 10-7, -2.7969 × 10-7, -2.39355 × 10-7, -1.7363 × 10-7,  
-1.34533 × 10-7, -8.72344 × 10-8, -5.75167 × 10-8, -2.89245 × 10-8, -1.4163 × 10-8,  
-6.0715 × 10-13, -1.8002 × 10-13, 0., 0., 0., 0., 0., 0., 0., 0., 0., 0., 0.,  
0., 0., 0., 0., 0., 0., 0., 0., 0., 0., 0., 0., 0., 0., 0., 0.,  
0., 0., 0., 0., 0., 0., 0., 0., 0., 0., 0., 0., 0., 0., 0., 0. }
```

## Integral over the probabilities

[illegible]

```
In[106]:= posinfinityrad := 1*^10 * posinfinity
```

```
In[107]:= expIntGam = Transpose[Eigenvectors[matRad]].DiagonalMatrix[
  diagelemint[posinfinityrad]].Inverse[Transpose[Eigenvectors[matRad]]];
```

## Crater integration of fluorescence

All charge states:

```
In[108]:= probability[sol_] := expGamInf. (Values[sol[[1]]] /. t -> posinfinity)
```

```
In[109]:= probabilityaction[sol_] :=
  NIntegrate[Values[sol[[1]]], {t, neginfinity, posinfinity}, AccuracyGoal -> 10,
    MinRecursion -> 10, MaxRecursion -> 20, Method -> "LocalAdaptive"] +
  expIntGam. (Values[sol[[1]]] /. t -> posinfinity)
```

Compute fluorescence for a fraction of the peak x-ray fluences on the beam axis:

```
In[110]:= fluorescenceprofile[pulseenergy_, photonenergy_, tauX_, nintsteps_, nint_] := Module[{J0Xpea
  J0Xpeak = 2*Sqrt[Log[2]/Pi]/tauX*peakfluence[pulseenergy, photonenergy];
  J0Xcur = J0Xpeak/nintsteps*nint;
  jxcrater[t_] := jxgaussian[J0Xcur, tauX, t];
  sol = solveRateEquations[photonenergy, jxcrater, neginfinity, posinfinity, 1/10000];
  Join[{J0Xcur}, probability[sol], probabilityaction[sol]]
  ]
```

```
In[111]:= tabfluorescenceprof[pulseenergy_, photonenergy_, tauX_, nintsteps_] := Module[{nint},
  Table[fluorescenceprofile[pulseenergy, photonenergy, tauX, nintsteps, nint],
    {nint, nintsteps, 0, -1}]
  ]
```

Create interpolation functions for all charge states:

```
In[112]:= interpolfluorescence[tabdata_] := Module[{nint},
  Table[
    ListInterpolation[tabdata[[All, nint]], {tabdata[[All, 1]]}],
    {nint, 2, Length[tabdata[[1]]]}]
  ]
```

Evaluate all fluorescence at a specific spatial point:

```
In[113]:= fluorescenceint[funyields_, pulseenergy_, photonenergy_, tauX_, rx_, ry_] := Module[{jj0x, nin
  jj0x = J0Xfun[pulseenergy, photonenergy, tauX, rx, ry];
  Table[funyields[[nint]][jj0x], {nint, 1, Length[funyields]}]
  ]
```

Integration of the fluorescence of the beam area. The integral needs to be normalized to the integration area:

```

In[114]:= fluorescencebeam[funyields_, pulseenergy_, photonenergy_, tauX_] :=
  1 / ((2 * 5 * MicrometerToBohr) ^ 2) * NIntegrate[
    fluorescenceint[funyields, pulseenergy, photonenergy, tauX, rx, ry],
    {rx, -5 * MicrometerToBohr, 5 * MicrometerToBohr},
    {ry, -5 * MicrometerToBohr, 5 * MicrometerToBohr},
    MaxRecursion -> 20, Method -> "LocalAdaptive", AccuracyGoal -> 10]

In[115]:= fluorescencecrateranalysis[pulseenergy_, photoenergy_, pulseduration_, nint_] := Module[{ta
  tabionyi = tabfluorescenceprof[pulseenergy, photoenergy, pulseduration, nint];
  funionyi = interpolfluorescence[tabionyi];
  fluorescencebeam[funionyi, pulseenergy, photoenergy, pulseduration]
}]

```

## Fluorescence spectrum from the plain rate equations

```
In[116]:= crava = fluorescencecrateranalysis[pulseenergy, omegaX, tauX, nintdata];
```

First Length[configurations] elements are the probability:

```
In[117]:= prob = crava[[1 ;; 63]]
```

```
Out[117]:= {0.913102, 0.00207947, 0., 0., 0.0235917, 0., 0., 0., 0., 0., 0.00212353, 0., 0., 0.,
  0., 0., 0., 0., 0.0114965, 0., 0., 0., 0., 0., 0., 0., 0.00192679, 0., 0.,
  0., 0., 0., 0., 0., 0.00700726, 0., 0., 0., 0., 0., 0., 0.00206717,
  0., 5.06534 × 10-120, 7.20358 × 10-115, 1.95879 × 10-222, 0., 0., 0., 0.0151453,
  0., 0., 2.40062 × 10-265, 4.31818 × 10-259, 0., 0.02146, 0., 0., 1.36836 × 10-7}
```

```
In[118]:= Partition[Riffle[configurations, prob], 2][[terminalcfg]] // TableForm
```

```
Out[118]//TableForm=
```

```

226    0.913102
225    0.00207947
224    0.0235917
223    0.00212353
222    0.0114965
221    0.00192679
220    0.00700726
210    0.00206717
200    0.0151453
100    0.02146
000    1.36836 × 10-7

```

Second Length[configurations] elements are the probability action:

```
In[119]:= probaction = crava[[64 ;; 126]]
```

```
Out[119]= {3.77489 × 1015, 8.59682 × 1012, 2507.95, 7.58632, 9.75311 × 1013, 23005., 4908.41,  
0.215309, 0.375452, 0.0681753, 8.77895 × 1012, 5921.12, 1016.62, 3.74038,  
1.98766, 0.621736, 0.00386759, 0.00863313, 4.75282 × 1013, 48881.3, 14230.5,  
0.243278, 0.712251, 0.181303, 0.0668832, 0.043467, 0.0140638, 7.96559 × 1012,  
20485., 6094.18, 2.08743, 3.67347, 1.94242, 0.00802599, 0.0282549, 0.00655152,  
2.8969 × 1013, 232456., 72225.2, 0.217947, 1.65863, 1.00171, 0.0917775, 0.202574,  
0.0829681, 8.54598 × 1012, 104476., 0.719339, 16.6836, 13.144, 0.00675621,  
0.139245, 0.0519821, 6.2601 × 1013, 1.16331 × 1010, 129.916, 0.000031956,  
0.00478224, 0.005479, 8.87188 × 1013, 162672., 0.00601039, 5.65698 × 108}
```

```
In[120]:= fluorescence = fluorencematrix.probaction;
```

```
In[121]:= spectrumFluorescence =  
Table[{fluorencenergy[[i]] * HartreeToeV, fluorescence[[i]]},  
{i, 1, Length[fluorescence]}];
```

```
In[122]:= spectrumFluorescenceNorm =  
Table[{spectrumFluorescence[[i, 1]], 1/Total[spectrumFluorescence[[ ; ; , 2]]] *  
spectrumFluorescence[[i, 2]]}, {i, 1, Length[spectrumFluorescence]}];
```

```
In[123]:= ListPlot[spectrumFluorescenceNorm, PlotRange → {{10, 40}, {0, 0.2}},  
Filling → Bottom, FillingStyle → Thick, PlotMarkers → {Automatic, Small},  
PlotStyle → {Red, Thick}, AxesLabel → {"", "y(ω)"},  
LabelStyle → {FontFamily → "Helvetica", FontSize → 14},  
AxesStyle → {Medium, Arrowheads[Automatic]}]
```

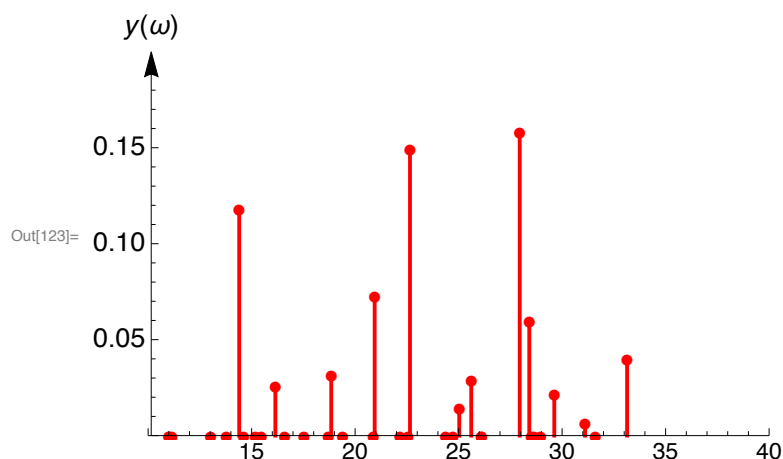



```

In[124]:= ListPlot[spectrumFluorescenceNorm, PlotRange → {{840, 930}, {0, 0.2}},
  Filling → Bottom, FillingStyle → Thick, PlotMarkers → {Automatic, Small},
  PlotStyle → {Red, Thick}, Axes → {True, False}, AxesLabel → {" $\omega$  [eV]", ""},
  LabelStyle → {FontFamily → "Helvetica", FontSize → 14},
  AxesStyle → Arrowheads[Automatic]]

```

Out[124]=

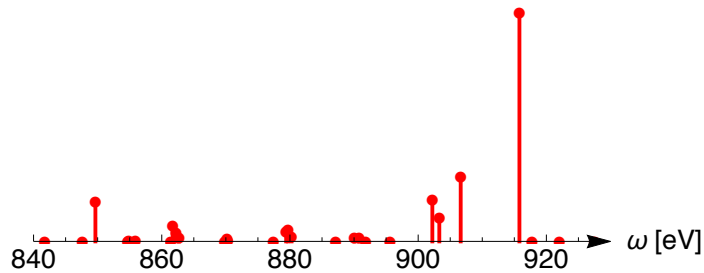

```

In[125]:= ListLogPlot[spectrumFluorescenceNorm, PlotRange → {{800, 1050}, {0.00001, 1}},
  Filling → Bottom, FillingStyle → Thick, PlotMarkers → {Automatic, Small},
  PlotStyle → {Red, Thick}, AxesLabel → {" $\omega$  [eV]", ""},
  LabelStyle → {FontFamily → "Helvetica", FontSize → 14},
  AxesStyle → Arrowheads[Automatic]]

```

Out[125]=

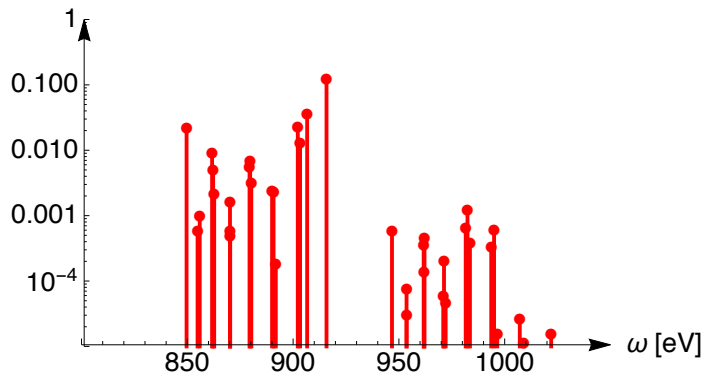

```

In[126]:= spectrumFluorescenceStates =
  Table[{i, fluorescencetransitions[[i]], fluorecenceenergy[[i]] * HartreeToeV,
    spectrumFluorescenceNorm[[i, 2]]}, {i, 1, 100}];

```

```
In[127]:= Sort[spectrumFluorescenceStates, #1[[4]] > #2[[4]] &][[1 ;; 20]] // TableForm
Out[127]//TableForm=
```

|    |       |       |       |       |       |       |       |         |            |
|----|-------|-------|-------|-------|-------|-------|-------|---------|------------|
| 4  | 1s(2) | 2s(1) | 2p(5) | ----> | 1s(2) | 2s(2) | 2p(4) | 27.9511 | 0.157954   |
| 27 | 1s(2) | 2s(1) | 2p(3) | ----> | 1s(2) | 2s(2) | 2p(2) | 22.6515 | 0.149136   |
| 90 | 1s(1) | 2s(0) | 2p(1) | ----> | 1s(2) | 2s(0) | 2p(0) | 915.795 | 0.128669   |
| 59 | 1s(2) | 2s(1) | 2p(1) | ----> | 1s(2) | 2s(2) | 2p(0) | 14.4009 | 0.118146   |
| 60 | 1s(2) | 2s(0) | 2p(2) | ----> | 1s(2) | 2s(1) | 2p(1) | 20.9451 | 0.0729956  |
| 28 | 1s(2) | 2s(0) | 2p(4) | ----> | 1s(2) | 2s(1) | 2p(3) | 28.4145 | 0.0598517  |
| 5  | 1s(2) | 2s(0) | 2p(6) | ----> | 1s(2) | 2s(1) | 2p(5) | 33.1401 | 0.0398634  |
| 89 | 1s(1) | 2s(1) | 2p(0) | ----> | 1s(2) | 2s(0) | 2p(0) | 906.634 | 0.0367986  |
| 43 | 1s(2) | 2s(1) | 2p(2) | ----> | 1s(2) | 2s(2) | 2p(1) | 18.8468 | 0.0314005  |
| 13 | 1s(2) | 2s(1) | 2p(4) | ----> | 1s(2) | 2s(2) | 2p(3) | 25.6103 | 0.0291001  |
| 75 | 1s(2) | 2s(0) | 2p(1) | ----> | 1s(2) | 2s(1) | 2p(0) | 16.1478 | 0.0260008  |
| 80 | 1s(1) | 2s(0) | 2p(2) | ----> | 1s(2) | 2s(0) | 2p(1) | 902.212 | 0.0235913  |
| 2  | 1s(1) | 2s(2) | 2p(6) | ----> | 1s(2) | 2s(2) | 2p(5) | 849.65  | 0.0228925  |
| 1  | 1s(2) | 2s(1) | 2p(6) | ----> | 1s(2) | 2s(2) | 2p(5) | 29.6225 | 0.0215008  |
| 44 | 1s(2) | 2s(0) | 2p(3) | ----> | 1s(2) | 2s(1) | 2p(2) | 25.0309 | 0.0144065  |
| 77 | 1s(1) | 2s(1) | 2p(1) | ----> | 1s(2) | 2s(1) | 2p(0) | 903.298 | 0.0135697  |
| 15 | 1s(1) | 2s(2) | 2p(4) | ----> | 1s(2) | 2s(2) | 2p(3) | 861.711 | 0.0094125  |
| 47 | 1s(1) | 2s(1) | 2p(3) | ----> | 1s(2) | 2s(1) | 2p(2) | 879.7   | 0.00720743 |
| 14 | 1s(2) | 2s(0) | 2p(5) | ----> | 1s(2) | 2s(1) | 2p(4) | 31.1105 | 0.00636397 |
| 50 | 1s(1) | 2s(0) | 2p(4) | ----> | 1s(2) | 2s(0) | 2p(3) | 879.407 | 0.00567299 |

## Modified rate equations

```
In[128]:= Solve[a / (1 - a) == shake, a]
```

```
Out[128]= {{a ->  $\frac{\text{shake}}{1 + \text{shake}}$ }}
```

Photoionization shake off from Table I of Ref. [3]:

```
In[129]:= valshakeoff :=  $\frac{0.16}{1 + 0.16}$ 
```

Photoionization shake off from Table III of Ref. [3]:

```
In[130]:= coresshakeoff :=  $\frac{0.23}{1 + 0.23}$ 
```

Double Auger decay partial probabilities from Table I of Ref. [2]:

```
In[131]:= p2pm3 := 2.5 / 100
p2sm12pm2 := 2.9 / 100
p2sm22pm1 := 0.5 / 100
pNem3 := p2pm3 + p2sm12pm2 + p2sm22pm1
```

Probabilities from Table I of Ref. [4]:

```
In[135]:= daNe2p := 0.9267
daNe3p := 0.0597
```

```
In[137]:= d = daNe3p / (daNe2p + daNe3p)
```

```
Out[137]= 0.0605231
```

```
In[138]:= 1 - d
```

```
Out[138]= 0.939477
```

Double Auger decay fractions:

```

In[139]:= da223v126 = p2pm3 / pNem3 * d
Out[139]= 0.0256454

In[140]:= da214v126 = p2sm12pm2 / pNem3 * d
Out[140]= 0.0297486

In[141]:= da205v126 = p2sm22pm1 / pNem3 * d
Out[141]= 0.00512908

In[142]:= daTot126 := da223v126 + da214v126 + da205v126

```

## Multiple photoionization of the valence electrons

```

In[143]:= req225[en_, jx_] := P225'[t] == (1 - valshakeoff) * xsc225v226[en] * jx[t] * P226[t] -
          xscTot225[en] * jx[t] * P225[t] + GamR225v216 * P216[t] + GamR225v126 * P126[t]

In[144]:= req216[en_, jx_] := P216'[t] == (1 - valshakeoff) * xsc216v226[en] * jx[t] * P226[t] -
          xscTot216[en] * jx[t] * P216[t] + GamR216v126 * P126[t] - GamRTot216 * P216[t]

```

## Multiple photoionization of core and valence electrons

```

In[145]:= req126[en_, jx_] := P126'[t] == (1 - coreshakeoff) * xsc126v226[en] * jx[t] * P226[t] -
          xscTot126[en] * jx[t] * P126[t] - GamATot126 * P126[t] - GamRTot126 * P126[t]

In[146]:= req125[en_, jx_] := P125'[t] == coreshakeoff * xsc126v226[en] * jx[t] * P226[t] +
          xsc125v225[en] * jx[t] * P225[t] + xsc125v126[en] * jx[t] * P126[t] -
          xscTot125[en] * jx[t] * P125[t] - GamATot125 * P125[t] +
          GamR125v116 * P116[t] + GamR125v026 * P026[t] - GamRTot125 * P125[t]

```

## Double Auger decay

```

In[147]:= req224[en_, jx_] := P224'[t] ==
          valshakeoff * xsc225v226[en] * jx[t] * P226[t] + xsc224v225[en] * jx[t] * P225[t] -
          xscTot224[en] * jx[t] * P224[t] + (1 - daTot126) * GamA224v126 * P126[t] +
          GamR224v215 * P215[t] + GamR224v125 * P125[t]

In[148]:= req215[en_, jx_] := P215'[t] ==
          valshakeoff * xsc216v226[en] * jx[t] * P226[t] + xsc215v225[en] * jx[t] * P225[t] +
          xsc215v216[en] * jx[t] * P216[t] - xscTot215[en] * jx[t] * P215[t] +
          (1 - daTot126) * GamA215v126 * P126[t] + GamR215v206 * P206[t] +
          GamR215v125 * P125[t] + GamR215v116 * P116[t] - GamRTot215 * P215[t]

In[149]:= req206[en_, jx_] :=
          P206'[t] == xsc206v216[en] * jx[t] * P216[t] - xscTot206[en] * jx[t] * P206[t] +
          (1 - daTot126) * GamA206v126 * P126[t] + GamR206v116 * P116[t] - GamRTot206 * P206[t]

In[150]:= req223[en_, jx_] := P223'[t] == xsc223v224[en] * jx[t] * P224[t] -
          xscTot223[en] * jx[t] * P223[t] + da223v126 * GamATot126 * P126[t] +
          GamA223v125 * P125[t] + GamR223v214 * P214[t] + GamR223v124 * P124[t]

```

```

In[151]:= req214[en_, jx_] :=
  P214'[t] == xsc214v224[en] * jx[t] * P224[t] + xsc214v215[en] * jx[t] * P215[t] -
    xscTot214[en] * jx[t] * P214[t] + da214v126 * GamATot126 * P126[t] +
    GamA214v125 * P125[t] + GamA214v116 * P116[t] + GamR214v205 * P205[t] +
    GamR214v124 * P124[t] + GamR214v115 * P115[t] - GamRTot214 * P214[t]

In[152]:= req205[en_, jx_] :=
  P205'[t] == xsc205v215[en] * jx[t] * P215[t] + xsc205v206[en] * jx[t] * P206[t] -
    xscTot205[en] * jx[t] * P205[t] + da205v126 * GamATot126 * P126[t] +
    GamA205v125 * P125[t] + GamA205v116 * P116[t] +
    GamR205v115 * P115[t] + GamR205v106 * P106[t] - GamRTot205 * P205[t]

```

## Convergence of the calculation

### Temporal integration: Probabilities

```

In[153]:= probabilitytime[sol_, t1_] := expGamInf. (Values[sol[[1]]] /. t -> t1)

In[154]:= absdiff[pinf_, maxfrac_] := Module[{sol},
  sol = solveRateEquations[omegaX, flux, neginfinity, pinf, maxfrac];
  Total[Abs[probabilitytime[sol, pinf] - probabilitytime[sol, pinf/10]]]
]

In[155]:= absdiff[10 * posinfinity, 1/10000] - absdiff[10 * posinfinity, 1/3000]

Out[155]:= 3.4181 × 10-14

In[156]:= tababsdiff = Table[{10^i, absdiff[10^i * FemtoSecondTot0, 1/10000]}, {i, 2, 9}]

Out[156]:= {{100, 0.65692}, {1000, 0.0283216}, {10000, 1.85304 × 10-12},
  {100000, 8.28865 × 10-14}, {1000000, 3.62978 × 10-13}, {10000000, 9.58051 × 10-14},
  {100000000, 3.02869 × 10-14}, {1000000000, 5.55112 × 10-16}}

In[157]:= ListLogLogPlot[tababsdiff, Joined -> True]

```

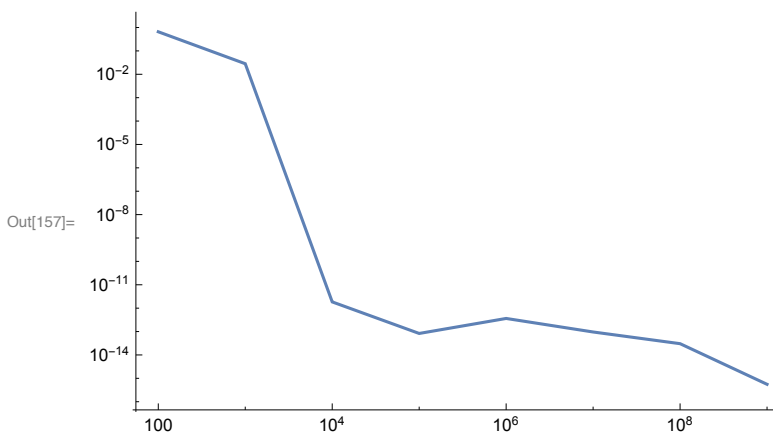

```
In[158]:= absdifftwo[pinf_, maxfrac_] := Module[{sol1, sol2},
  sol1 = solveRateEquations[omegaX, flux, neginfinity, pinf, maxfrac];
  sol2 = solveRateEquations[omegaX, flux, neginfinity, pinf/10, maxfrac];
  Total[Abs[probabilitytime[sol1, pinf] - probabilitytime[sol2, pinf/10]]]
]
```

```
In[159]:= absdifftwo[10 * posinfinity, 1/10000] - absdifftwo[10 * posinfinity, 1/3000]
```

```
Out[159]:=  $8.108 \times 10^{-7}$ 
```

```
In[160]:= tababsdifftwo =
  Table[{10^i, absdifftwo[10^i * FemtoSecondTot0, 1/10000]}, {i, 2, 9}]
```

```
Out[160]:= {{100, 0.65692}, {1000, 0.0283217}, {10000,  $2.72827 \times 10^{-7}$ },
  {100000,  $1.05377 \times 10^{-6}$ }, {1000000,  $7.65119 \times 10^{-7}$ }, {10000000,  $7.40005 \times 10^{-7}$ },
  {100000000,  $1.17127 \times 10^{-13}$ }, {1000000000,  $3.48521 \times 10^{-14}$ }}
```

```
In[161]:= ListLogLogPlot[tababsdifftwo, Joined -> True]
```

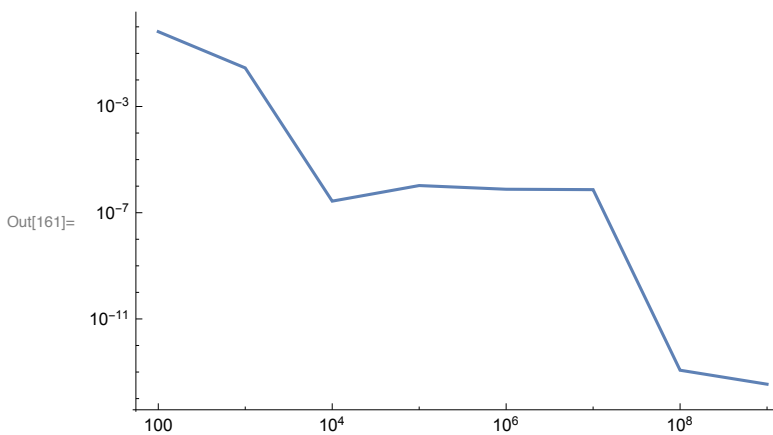

## Temporal integration: Probability action

```
In[162]:= diagelemintdelta[dt_] :=
  Table[If[eigval[[i]] != 0,  $\frac{-1}{\text{eigval}[[i]]}$ , dt], {i, 1, Length[eigval]}]
```

```
In[163]:= expIntGamDt[dt_] := Transpose[Eigenvectors[matRad]].
  DiagonalMatrix[diagelemintdelta[dt]].Inverse[Transpose[Eigenvectors[matRad]]]
```

```
In[164]:= probabilityactiontime[sol_, t1_] :=
  NIntegrate[Values[sol[[1]]], {t, neginfinity, t1}, AccuracyGoal -> 10,
    MinRecursion -> 10, MaxRecursion -> 20, Method -> "LocalAdaptive"] +
  expIntGamDt[posinfinityrad - t1].(Values[sol[[1]]] /. t -> t1)
```

```
In[165]:= safeErr[x_] := If[x == 0, 1, x]
```

```
In[166]:= absdiffaction[pinf_, maxfrac_] := Module[{sol, pa, pa10, relerr, i},
  sol = solveRateEquations[omegaX, flux, neginfinity, pinf, maxfrac];
  pa = probabilityactiontime[sol, pinf];
  pa10 = probabilityactiontime[sol, pinf/10];
  relerr = Table[(pa[[i]] - pa10[[i]])/safeErr[pa10[[i]]], {i, 1, Length[pa]}];
  Total[Abs[relerr]]
]
```

```
In[167]:= absdiffaction[10 * posinfinity, 1/10 000] - absdiffaction[10 * posinfinity, 1/3000]
```

```
Out[167]= 9.40761 × 10-6
```

```
In[168]:= tababsdiffaction =
  Table[{10^i, absdiffaction[10^i * FemtoSecondTot0, 1/10 000]}, {i, 2, 9}]
```

```
Out[168]= {{100, 59.3475}, {1000, 37.3063}, {10 000, 0.912569},
  {100 000, 0.0000163118}, {1 000 000, 3.01474 × 10-6},
  {10 000 000, 4.39231 × 10-6}, {100 000 000, 15.}, {1 000 000 000, 35.}}
```

```
In[169]:= ListLogLogPlot[tababsdiffaction, Joined -> True]
```

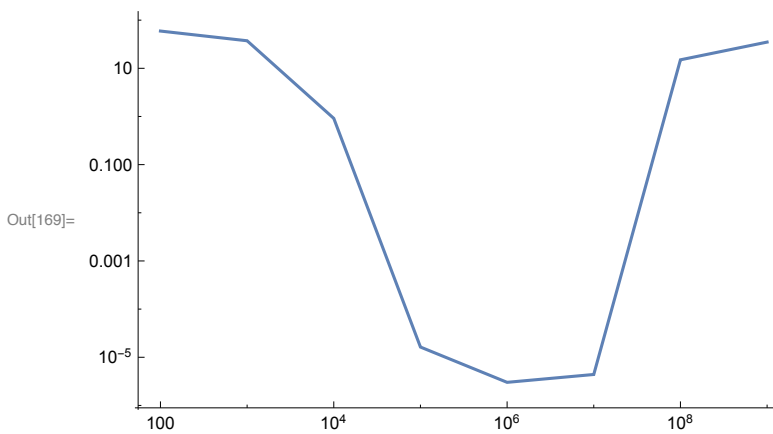

```
In[170]:= absdiffactiontwo[pinf_, maxfrac_] := Module[{sol1, sol2, pa, pa10, relerr, i},
  sol1 = solveRateEquations[omegaX, flux, neginfinity, pinf, maxfrac];
  sol2 = solveRateEquations[omegaX, flux, neginfinity, pinf/10, maxfrac];
  pa = probabilityactiontime[sol1, pinf];
  pa10 = probabilityactiontime[sol2, pinf/10];
  relerr = Table[(pa[[i]] - pa10[[i]])/safeErr[pa10[[i]]], {i, 1, Length[pa]}];
  Total[Abs[relerr]]
]
```

```
In[171]:= absdiffactiontwo[10 * posinfinity, 1/10 000] -
  absdiffactiontwo[10 * posinfinity, 1/3000]
```

```
Out[171]= 0.00163418
```

```
In[172]:= tababsdifttwo =
  Table[{10^i, absdiftactiontwo[10^i * FemtoSecondTot0, 1/10 000]}, {i, 2, 9}]
```

```
Out[172]= {{100, 59.3475}, {1000, 37.3064}, {10 000, 0.913479},
  {100 000, 0.00191773}, {1 000 000, 0.00280948},
  {10 000 000, 0.00389573}, {100 000 000, 15.0001}, {1 000 000 000, 35.002}}
```

```
In[173]:= ListLogLogPlot[tababsdifttwo, Joined -> True]
```

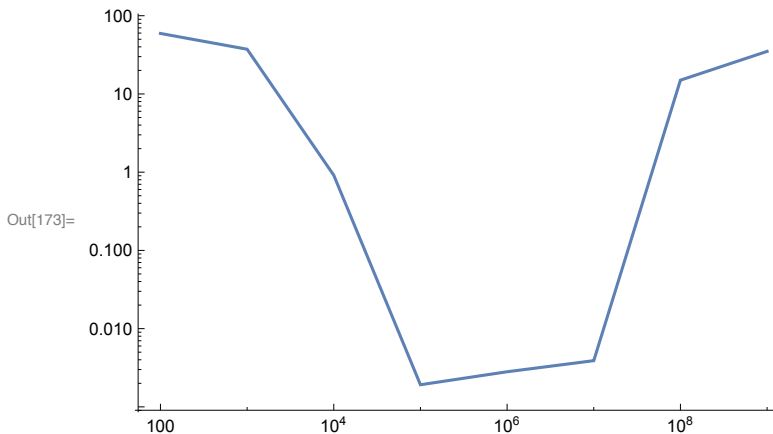

## Spatial integration: Probabilities

```
In[174]:= probabilitybeamdist[funyields_, pulseenergy_, photonenergy_, tauX_, dist_] :=
  Module[{cratint},
    cratint = 1 / ((2 * dist)^2) * NIntegrate[
      fluorescenceint[funyields, pulseenergy, photonenergy, tauX, rx, ry],
      {rx, -dist, dist}, {ry, -dist, dist}, MaxRecursion -> 20,
      Method -> "LocalAdaptive", AccuracyGoal -> 10];
    1 / Total[cratint[[2 ;; Length[configurations]]]] *
    cratint[[2 ;; Length[configurations]]]
  ]
```

```
In[175]:= tabionyi=tabfluorescenceprof[pulseenergy,omegaX,tauX,nintdata];
  funionyi=interpolfluorescence[tabionyi];
  ionyi=probabilitybeamdist[funionyi,pulseenergy,omegaX,tauX,10*MicrometerToBohr];
```

```
In[178]:= diffdist[dist_] := Total[
  Abs[probabilitybeamdist[funionyi, pulseenergy, omegaX, tauX, dist] - ionyi]]
```

```
In[179]:= tabdiffdist = Table[{i, diffdist[i * MicrometerToBohr]}, {i, 1, 9}]
```

```
Out[179]= {{1, 0.573791}, {2, 0.110226}, {3, 0.00371548},
  {4, 0.0000226151}, {5, 5.49434 × 10^-7}, {6, 4.96268 × 10^-7},
  {7, 9.25404 × 10^-7}, {8, 2.30832 × 10^-7}, {9, 1.43082 × 10^-7}}
```

```
In[180]:= ListLogPlot[tabdiffdist, Joined -> True, PlotRange -> All]
```

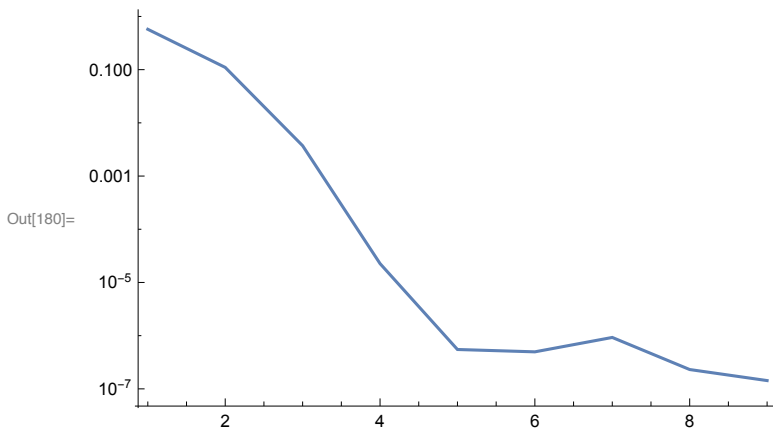

## Spatial integration: Probability action

```
In[181]:= probabilityactionbeamdistr[funyield_, pulseenergy_,
    photonenergy_, tauX_, dist_] := Module[{cratint},
    cratint = 1 / ((2 * dist) ^ 2) * NIntegrate[
        fluorescenceint[funyield_, pulseenergy_, photonenergy_, tauX_, rx, ry],
        {rx, -dist, dist}, {ry, -dist, dist}, MinRecursion -> 10, MaxRecursion -> 20,
        Method -> "LocalAdaptive", AccuracyGoal -> 10];
    cratint[[Length[configurations] + 1 ;; 2 * Length[configurations]]]
]

In[182]:= tabionyi=tabfluorescenceprof[pulseenergy,omegaX,tauX,nintdata];
funionyi=interpolfluorescence[tabionyi];
ionyi=probabilityactionbeamdistr[funionyi,pulseenergy,omegaX,tauX,10*MicrometerToBohr];

In[185]:= diffdist[dist_] := Module[{sf, sf10, nsf, nsf10, relerr, i},
    sf = fluorecencematrix.
    probabilityactionbeamdistr[funionyi, pulseenergy, omegaX, tauX, dist];
    sf10 = fluorecencematrix.ionyi;
    nsf = sf * 1 / Total[sf];
    nsf10 = sf10 * 1 / Total[sf10];
    relerr =
    Table[(nsf[[i]] - nsf10[[i]]) / safeErr[nsf10[[i]]], {i, 1, Length[nsf]};
    Total[Abs[relerr]]
]

In[186]:= diffdist[5 * MicrometerToBohr]

Out[186]= 0.0000111626

In[187]:= tabdiffdist = Table[{i, diffdist[i * MicrometerToBohr]}, {i, 1, 9}]

Out[187]= {{1, 68.6371}, {2, 8.78747}, {3, 0.231487}, {4, 0.00140491}, {5, 0.0000111626},
    {6, 0.0000271685}, {7, 0.0000460785}, {8, 0.0000217345}, {9, 0.000021235}}
```



```
In[188]:= ListLogPlot[tabdiffdist, Joined -> True, PlotRange -> All]
```

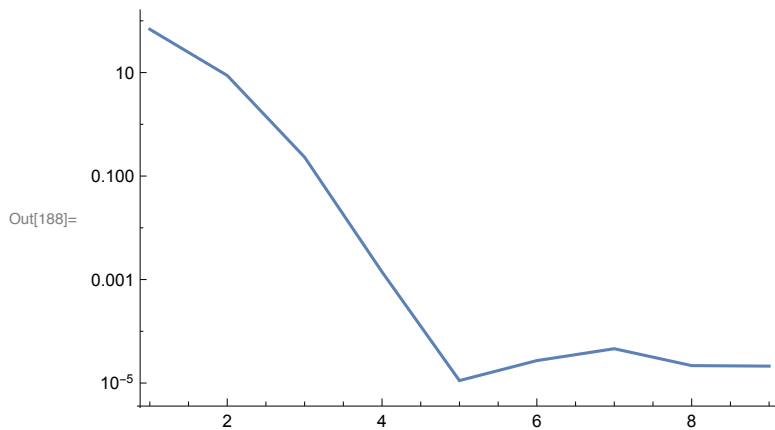

## Interpolation of the fluence

```
In[189]:= tabionyi=tabfluorescenceprof[pulseenergy,omegaX,tauX,nintdata];
funionyi=interpolfluorescence[tabionyi];

In[191]:= plotIonyi[idx_] := Module[{lp1, lp2},
  lp1 = ListPlot[tabionyi[[All, {1, idx+1}]],
    PlotRange -> All, PlotMarkers -> {Automatic, 10}, PlotStyle -> Black];
  lp2 = Plot[funionyi[[idx]][x], {x, 0, tabionyi[[1, 1]]},
    PlotRange -> All, PlotStyle -> Red];
  Show[lp1, lp2]
]

In[192]:= Manipulate[plotIonyi[idx], {idx, 1, Length[tabionyi[[1]]] - 1, 1}]
```

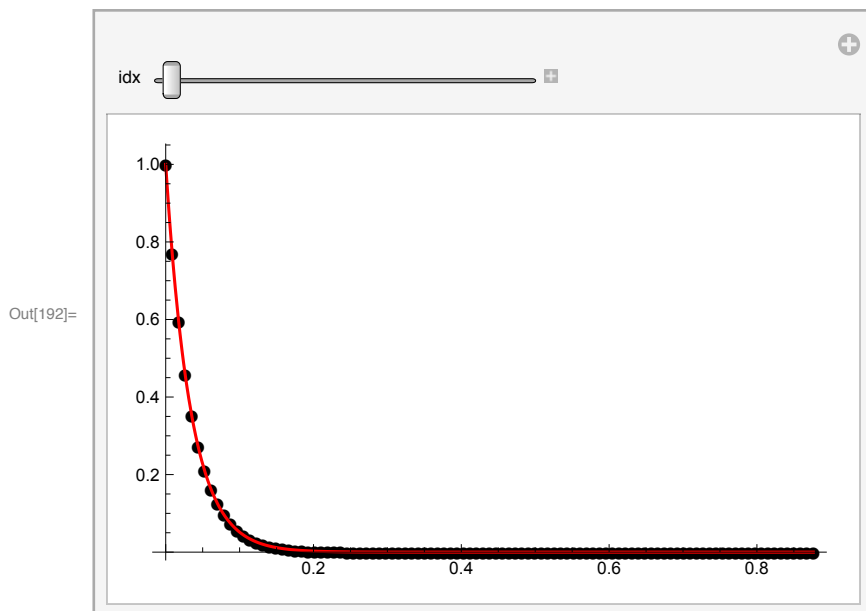

## Fluorescence spectrum from the modified rate equations

```
In[193]:= crava = fluorescencecrateranalysis[pulseenergy, omegaX, tauX, nintdata];
```

First Length[configurations] elements are the probability:

```
In[194]:= prob = crava[[1 ;; 63]]
Out[194]= {0.913102, 0.00177374, 0., 0., 0.0183612, 0., 0., 0., 0., 0., 0.0075726, 0., 0., 0.,
0., 0., 0., 0., 0.00919243, 0., 0., 0., 0., 0., 0., 0., 0.00418371, 0., 0.,
0., 0., 0., 0., 0., 0.0057461, 0., 0., 0., 0., 0., 0., 0., 0.00324725,
0.,  $4.14393 \times 10^{-120}$ ,  $5.89321 \times 10^{-115}$ ,  $1.27496 \times 10^{-222}$ , 0., 0., 0., 0.0177446,
0., 0.,  $2.1982 \times 10^{-265}$ ,  $3.95408 \times 10^{-259}$ , 0., 0.019076, 0., 0.,  $2.20563 \times 10^{-7}$ }
```

```
In[195]:= Partition[Riffle[configurations, prob], 2][[terminalcfg]] // TableForm
Out[195]//TableForm=
226    0.913102
225    0.00177374
224    0.0183612
223    0.0075726
222    0.00919243
221    0.00418371
220    0.0057461
210    0.00324725
200    0.0177446
100    0.019076
000     $2.20563 \times 10^{-7}$ 
```

Second Length[configurations] elements are the probability action:

```
In[196]:= probaction = crava[[64 ;; 126]]
Out[196]= { $3.77489 \times 10^{15}$ ,  $7.3329 \times 10^{12}$ , 2162.02, 6.16774,  $7.59078 \times 10^{13}$ , 18062.4, 3752.9,
1.76818, 0.322441, 0.0554262,  $3.13062 \times 10^{13}$ , 14816.8, 2750.96, 2.9052,
1.58467, 0.476617, 0.0166045, 0.00740167,  $3.80028 \times 10^{13}$ , 39259.6, 11260.6,
1.13359, 1.26336, 0.348924, 0.0519812, 0.0347167, 0.0107931,  $1.7296 \times 10^{13}$ ,
41811.4, 12316., 1.65417, 3.00489, 1.54628, 0.0279784, 0.0423565, 0.0104281,
 $2.37552 \times 10^{13}$ , 190731., 58880.7, 0.672863, 2.89911, 1.71632, 0.0728434, 0.166246,
0.0662602,  $1.34246 \times 10^{13}$ , 167994., 0.583999, 13.9969, 10.837, 0.0171811,
0.218594, 0.0791925,  $7.33411 \times 10^{13}$ ,  $1.73945 \times 10^{10}$ , 185.464, 0.0000742362,
0.00791845, 0.00809896,  $7.88626 \times 10^{13}$ , 266019., 0.00932176,  $9.11836 \times 10^8$ }
```

```
In[197]:= fluorescence = fluorencematrix.probaction;
In[198]:= spectrumFluorescence =
Table[{fluorencenergy[[i]] * HartreeToeV, fluorescence[[i]]},
{i, 1, Length[fluorescence]}];
In[199]:= spectrumFluorescenceNorm =
Table[{spectrumFluorescence[[i, 1]], 1/Total[spectrumFluorescence[[ ;; , 2]]] *
spectrumFluorescence[[i, 2]]}, {i, 1, Length[spectrumFluorescence]}];
```

```

In[200]:= ListPlot[spectrumFluorescenceNorm, PlotRange → {{10, 40}, {0, 0.2}},
  Filling → Bottom, FillingStyle → Thick, PlotMarkers → {Automatic, Small},
  PlotStyle → {Red, Thick}, AxesLabel → {"", "y(ω)"},
  LabelStyle → {FontFamily → "Helvetica", FontSize → 14},
  AxesStyle → {Medium, Arrowheads[Automatic]}]

```

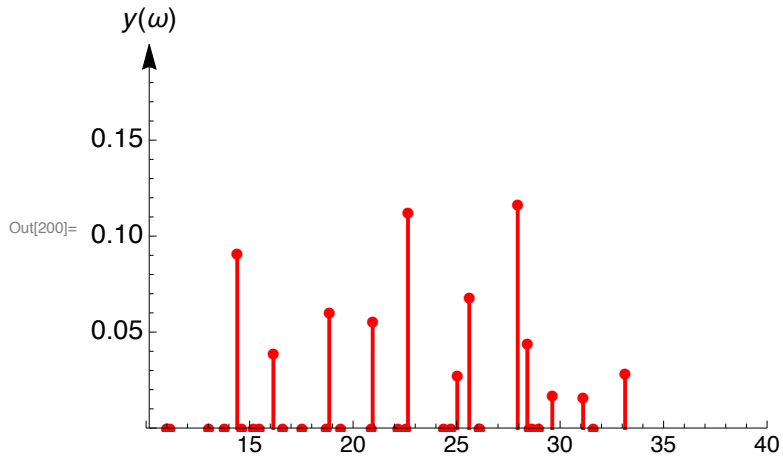

```

In[201]:= ListPlot[spectrumFluorescenceNorm, PlotRange → {{10, 40}, {0, 0.2}},
  Filling → Bottom, FillingStyle → Thick, PlotMarkers → {Automatic, Small},
  PlotStyle → {Red, Thick}, AxesLabel → {"", "y(ω)"},
  LabelStyle → {FontFamily → "Helvetica", FontSize → 14},
  AxesStyle → {Medium, Arrowheads[Automatic]},
  ImagePadding → {{All, All}, {40, All}}, Axes → False,
  LabelStyle → {FontFamily → "Helvetica", FontSize → 14}, Frame → True,
  FrameStyle → Thick, FrameTicks → True, FrameTicksStyle → Thick,
  FrameLabel → {"Photon energy ω [eV]", "Photon yield y(ω)"}]

```

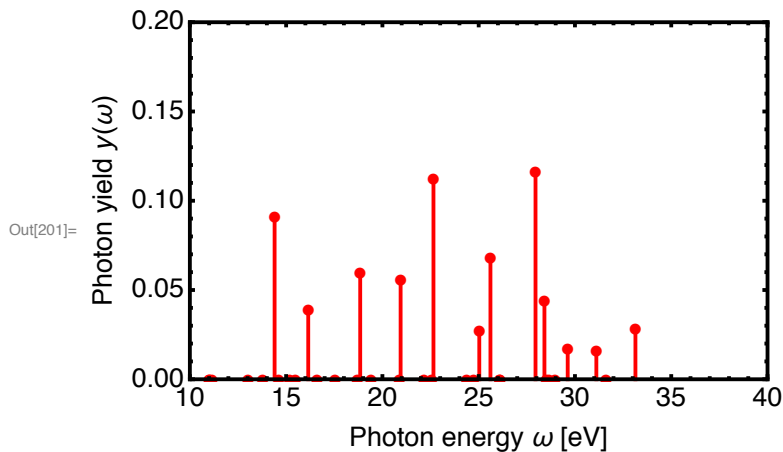

```

In[202]:= ListPlot[spectrumFluorescenceNorm, PlotRange → {{840, 930}, {0, 0.2}},
  Filling → Bottom, FillingStyle → Thick, PlotMarkers → {Automatic, Small},
  PlotStyle → {Red, Thick}, Axes → {True, False}, AxesLabel → {" $\omega$  [eV]", ""},
  LabelStyle → {FontFamily → "Helvetica", FontSize → 14},
  AxesStyle → Arrowheads[Automatic]]

```

Out[202]=

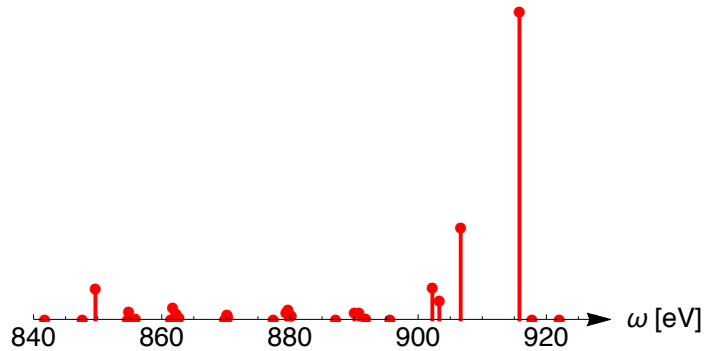

```

In[203]:= ListPlot[spectrumFluorescenceNorm, PlotRange → {{840, 930}, {0, 0.2}},
  Filling → Bottom, FillingStyle → Thick, PlotMarkers → {Automatic, Small},
  PlotStyle → {Red, Thick}, AxesLabel → {"", " $y(\omega)$ "},
  LabelStyle → {FontFamily → "Helvetica", FontSize → 14},
  AxesStyle → {Medium, Arrowheads[Automatic]},
  ImagePadding → {{All, All}, {40, All}}, Axes → False,
  LabelStyle → {FontFamily → "Helvetica", FontSize → 14}, Frame → True,
  FrameStyle → Thick, FrameTicks → True, FrameTicksStyle → Thick,
  FrameLabel → {"Photon energy  $\omega$  [eV]", "Photon yield  $y(\omega)$ "}]

```

Out[203]=

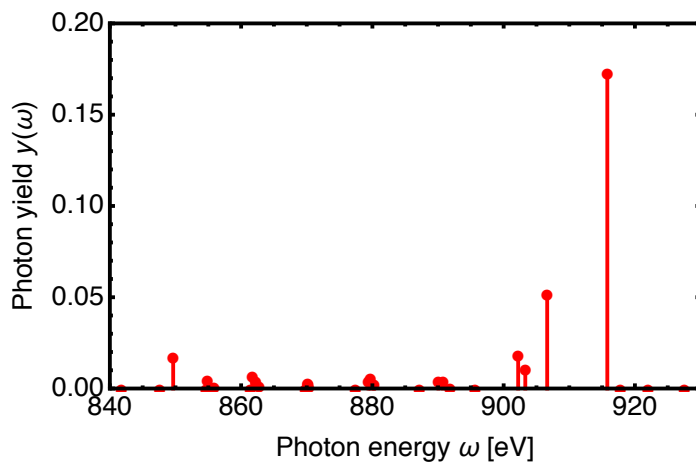

```
In[204]:= ListLogPlot[spectrumFluorescenceNorm, PlotRange → {{800, 1050}, {0.00001, 1}},
  Filling → Bottom, FillingStyle → Thick, PlotMarkers → {Automatic, Small},
  PlotStyle → {Red, Thick}, AxesLabel → {" $\omega$  [eV]", ""},
  LabelStyle → {FontFamily → "Helvetica", FontSize → 14},
  AxesStyle → Arrowheads[Automatic]]
```

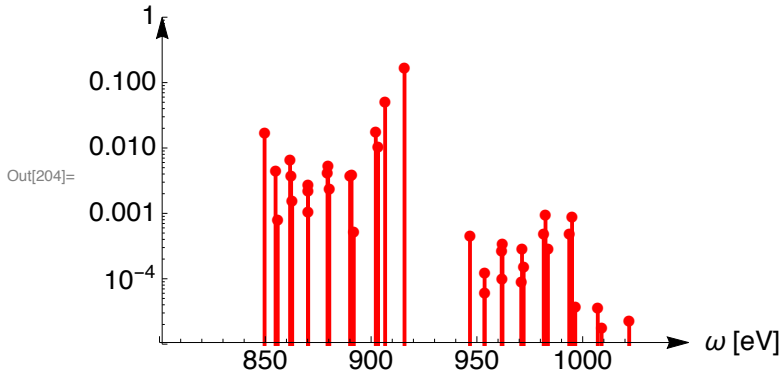

```
In[205]:= spectrumFluorescenceStates =
  Table[{i, fluorescencetransitions[[i]], fluorecenceenergy[[i]] * HartreeToEV,
    spectrumFluorescenceNorm[[i, 2]]}, {i, 1, 100}];
```

```
In[206]:= Sort[spectrumFluorescenceStates, #1[[4]] > #2[[4]] &][[1 ;; 20]] // TableForm
```

Out[206]//TableForm=

|    |       |       |       |       |       |       |       |         |            |
|----|-------|-------|-------|-------|-------|-------|-------|---------|------------|
| 90 | 1s(1) | 2s(0) | 2p(1) | ----> | 1s(2) | 2s(0) | 2p(0) | 915.795 | 0.172823   |
| 4  | 1s(2) | 2s(1) | 2p(5) | ----> | 1s(2) | 2s(2) | 2p(4) | 27.9511 | 0.116684   |
| 27 | 1s(2) | 2s(1) | 2p(3) | ----> | 1s(2) | 2s(2) | 2p(2) | 22.6515 | 0.112698   |
| 59 | 1s(2) | 2s(1) | 2p(1) | ----> | 1s(2) | 2s(2) | 2p(0) | 14.4009 | 0.0912076  |
| 13 | 1s(2) | 2s(1) | 2p(4) | ----> | 1s(2) | 2s(2) | 2p(3) | 25.6103 | 0.0685135  |
| 43 | 1s(2) | 2s(1) | 2p(2) | ----> | 1s(2) | 2s(2) | 2p(1) | 18.8468 | 0.0603013  |
| 60 | 1s(2) | 2s(0) | 2p(2) | ----> | 1s(2) | 2s(1) | 2p(1) | 20.9451 | 0.0559901  |
| 89 | 1s(1) | 2s(1) | 2p(0) | ----> | 1s(2) | 2s(0) | 2p(0) | 906.634 | 0.0517697  |
| 28 | 1s(2) | 2s(0) | 2p(4) | ----> | 1s(2) | 2s(1) | 2p(3) | 28.4145 | 0.0445603  |
| 75 | 1s(2) | 2s(0) | 2p(1) | ----> | 1s(2) | 2s(1) | 2p(0) | 16.1478 | 0.0393364  |
| 5  | 1s(2) | 2s(0) | 2p(6) | ----> | 1s(2) | 2s(1) | 2p(5) | 33.1401 | 0.0286768  |
| 44 | 1s(2) | 2s(0) | 2p(3) | ----> | 1s(2) | 2s(1) | 2p(2) | 25.0309 | 0.0273932  |
| 80 | 1s(1) | 2s(0) | 2p(2) | ----> | 1s(2) | 2s(0) | 2p(1) | 902.212 | 0.0183007  |
| 2  | 1s(1) | 2s(2) | 2p(6) | ----> | 1s(2) | 2s(2) | 2p(5) | 849.65  | 0.0175113  |
| 1  | 1s(2) | 2s(1) | 2p(6) | ----> | 1s(2) | 2s(2) | 2p(5) | 29.6225 | 0.0174392  |
| 14 | 1s(2) | 2s(0) | 2p(5) | ----> | 1s(2) | 2s(1) | 2p(4) | 31.1105 | 0.0162026  |
| 77 | 1s(1) | 2s(1) | 2p(1) | ----> | 1s(2) | 2s(1) | 2p(0) | 903.298 | 0.0107113  |
| 15 | 1s(1) | 2s(2) | 2p(4) | ----> | 1s(2) | 2s(2) | 2p(3) | 861.711 | 0.00687855 |
| 47 | 1s(1) | 2s(1) | 2p(3) | ----> | 1s(2) | 2s(1) | 2p(2) | 879.7   | 0.00554705 |
| 6  | 1s(1) | 2s(2) | 2p(5) | ----> | 1s(2) | 2s(2) | 2p(4) | 854.849 | 0.00468699 |

## Fluorescence with Bhalla's Auger decay widths

### Bhalla's data

#### Total width of single core holes

```
In[207]:= bhGA126 := 88.066*^-4
bhGA125 := 78.753*^-4
bhGA124 := 66.278*^-4
bhGA123 := 51.633*^-4
bhGA122 := 36.687*^-4
bhGA121 := 23.994*^-4

bhGA116 := 80.428*^-4
bhGA115 := 67.321*^-4
bhGA114 := 51.162*^-4
bhGA113 := 33.624*^-4
bhGA112 := 17.113*^-4
bhGA111 := 4.716*^-4

bhGA106 := 77.901*^-4
bhGA105 := 61.854*^-4
bhGA104 := 43.571*^-4
bhGA103 := 25.306*^-4
bhGA102 := 9.682*^-4
```

```
In[224]:= GamATot126 := bhGA126
GamATot125 := bhGA125
GamATot124 := bhGA124
GamATot123 := bhGA123
GamATot122 := bhGA122
GamATot121 := bhGA121
GamATot116 := bhGA116
GamATot115 := bhGA115
GamATot114 := bhGA114
GamATot113 := bhGA113
GamATot112 := bhGA112
GamATot111 := bhGA111
GamATot106 := bhGA106
GamATot105 := bhGA105
GamATot104 := bhGA104
GamATot103 := bhGA103
GamATot102 := bhGA102
```

## 2p–2p decay of single core holes

```
In[241]:= bhGA224v126 := 55.284*^-4
          bhGA223v125 := 45.358*^-4
          bhGA222v124 := 33.070*^-4
          bhGA221v123 := 19.731*^-4
          bhGA220v122 := 7.698*^-4
```

```
          bhGA214v116 := 66.278*^-4
          bhGA213v115 := 53.548*^-4
          bhGA212v114 := 38.330*^-4
          bhGA211v113 := 22.495*^-4
          bhGA210v112 := 8.670*^-4
```

```
          bhGA204v106 := 77.901*^-4
          bhGA203v105 := 61.854*^-4
          bhGA202v104 := 43.571*^-4
          bhG201v103 := 25.306*^-4
          bhGA200v102 := 9.682*^-4
```

```
In[256]:= GamA224v126 := bhGA224v126
          GamA223v125 := bhGA223v125
          GamA222v124 := bhGA222v124
          GamA221v123 := bhGA221v123
          GamA220v122 := bhGA220v122
          GamA214v116 := bhGA214v116
          GamA213v115 := bhGA213v115
          GamA212v114 := bhGA212v114
          GamA211v113 := bhGA211v113
          GamA210v112 := bhGA210v112
          GamA204v106 := bhGA204v106
          GamA203v105 := bhGA203v105
          GamA202v104 := bhGA202v104
          GamA201v103 := bhG201v103
          GamA200v102 := bhGA200v102
```

## 2s–2p decay of single core holes

```
In[271]:= bhGA215v126 := 24.448*^-4
          bhGA214v125 := 24.002*^-4
          bhGA213v124 := 22.507*^-4
          bhGA212v123 := 19.682*^-4
          bhGA211v122 := 15.163*^-4
          bhGA210v121 := 8.606*^-4
```

```
          bhGA205v116 := 14.150*^-4
          bhGA204v115 := 13.773*^-4
          bhGA203v114 := 12.832*^-4
          bhGA202v113 := 11.129*^-4
          bhGA201v112 := 8.442*^-4
          bhGA200v111 := 4.716*^-4
```

```
In[283]:= GamA215v126 := bhGA215v126
          GamA214v125 := bhGA214v125
          GamA213v124 := bhGA213v124
          GamA212v123 := bhGA212v123
          GamA211v122 := bhGA211v122
          GamA210v121 := bhGA210v121
          GamA205v116 := bhGA205v116
          GamA204v115 := bhGA204v115
          GamA203v114 := bhGA203v114
          GamA202v113 := bhGA202v113
          GamA201v112 := bhGA201v112
          GamA200v111 := bhGA200v111
```

## 2s–2s decay of single core holes

```
In[295]:= bhGA206v126 := 8.334*^-4
          bhGA205v125 := 9.393*^-4
          bhGA204v124 := 10.701*^-4
          bhGA203v123 := 12.220*^-4
          bhGA202v122 := 13.827*^-4
          bhGA201v121 := 15.388*^-4
```

```
In[301]:= GamA206v126 := bhGA206v126
          GamA205v125 := bhGA205v125
          GamA204v124 := bhGA204v124
          GamA203v123 := bhGA203v123
          GamA202v122 := bhGA202v122
          GamA201v121 := bhGA201v121
```



## Total width of double core holes

```
In[307]:= bhGA026 := 129.860 * 2*^-4
          bhGA025 := 112.160 * 2*^-4
          bhGA024 := 91.009 * 2*^-4
          bhGA023 := 68.309 * 2*^-4
          bhGA022 := 46.790 * 2*^-4
          bhGA021 := 29.702 * 2*^-4
```

```
          bhGA016 := 119.128 * 2*^-4
          bhGA015 := 96.478 * 2*^-4
          bhGA014 := 70.982 * 2*^-4
          bhGA013 := 45.172 * 2*^-4
          bhGA012 := 22.201 * 2*^-4
          bhGA011 := 5.872 * 2*^-4
```

```
          bhGA006 := 116.220 * 2*^-4
          bhGA005 := 89.805 * 2*^-4
          bhGA004 := 61.849 * 2*^-4
          bhGA003 := 35.184 * 2*^-4
          bhGA002 := 13.161 * 2*^-4
```

```
In[324]:= GamATot026 := bhGA026
          GamATot025 := bhGA025
          GamATot024 := bhGA024
          GamATot023 := bhGA023
          GamATot022 := bhGA022
          GamATot021 := bhGA021
          GamATot016 := bhGA016
          GamATot015 := bhGA015
          GamATot014 := bhGA014
          GamATot013 := bhGA013
          GamATot012 := bhGA012
          GamATot011 := bhGA011
          GamATot006 := bhGA006
          GamATot005 := bhGA005
          GamATot004 := bhGA004
          GamATot003 := bhGA003
          GamATot002 := bhGA002
```

## 2p–2p decay of double core holes

```

In[341]:= bhGA124v026 := 85.925 * 2*^-4
          bhGA123v025 := 67.900 * 2*^-4
          bhGA122v024 := 47.598 * 2*^-4
          bhGA121v023 := 27.310 * 2*^-4
          bhGA120v022 := 10.233 * 2*^-4

          bhGA114v016 := 99.936 * 2*^-4
          bhGA113v015 := 78.032 * 2*^-4
          bhGA112v014 := 54.054 * 2*^-4
          bhGA111v013 := 30.757 * 2*^-4
          bhGA110v012 := 11.475 * 2*^-4

          bhGA104v006 := 116.220 * 2*^-4
          bhGA103v005 := 89.805 * 2*^-4
          bhGA102v004 := 61.849 * 2*^-4
          bhGA101v003 := 35.184 * 2*^-4
          bhGA100v002 := 13.161 * 2*^-4

In[356]:= GamA124v026 := bhGA124v026
          GamA123v025 := bhGA123v025
          GamA122v024 := bhGA122v024
          GamA121v023 := bhGA121v023
          GamA120v022 := bhGA120v022
          GamA114v016 := bhGA114v016
          GamA113v015 := bhGA113v015
          GamA112v014 := bhGA112v014
          GamA111v013 := bhGA111v013
          GamA110v012 := bhGA110v012
          GamA104v006 := bhGA104v006
          GamA103v005 := bhGA103v005
          GamA102v004 := bhGA102v004
          GamA101v003 := bhGA101v003
          GamA100v002 := bhGA100v002

```

## 2s–2p decay of double core holes

```
In[371]:= bhGA115v026 := 33.699 * 2*^-4
          bhGA114v025 := 32.558 * 2*^-4
          bhGA113v024 := 30.020 * 2*^-4
          bhGA112v023 := 25.753 * 2*^-4
          bhGA111v022 := 19.398 * 2*^-4
          bhGA110v021 := 10.772 * 2*^-4
```

```
          bhGA105v016 := 19.192 * 2*^-4
          bhGA104v015 := 18.446 * 2*^-4
          bhGA103v014 := 16.928 * 2*^-4
          bhGA102v013 := 14.415 * 2*^-4
          bhGA101v012 := 10.726 * 2*^-4
          bhGA100v011 := 5.872 * 2*^-4
```

```
In[383]:= GamA115v026 := bhGA115v026
          GamA114v025 := bhGA114v025
          GamA113v024 := bhGA113v024
          GamA112v023 := bhGA112v023
          GamA111v022 := bhGA111v022
          GamA110v021 := bhGA110v021
          GamA105v016 := bhGA105v016
          GamA104v015 := bhGA104v015
          GamA103v014 := bhGA103v014
          GamA102v013 := bhGA102v013
          GamA101v012 := bhGA101v012
          GamA100v011 := bhGA100v011
```

## 2s–2s decay of double core holes

```
In[395]:= bhGA106v026 := 10.239 * 2*^-4
          bhGA105v025 := 11.698 * 2*^-4
          bhGA104v024 := 13.390 * 2*^-4
          bhGA103v023 := 15.246 * 2*^-4
          bhGA102v022 := 17.160 * 2*^-4
          bhGA101v021 := 18.930 * 2*^-4
```

```
In[401]:= GamA106v026 := bhGA106v026
          GamA105v025 := bhGA105v025
          GamA104v024 := bhGA104v024
          GamA103v023 := bhGA103v023
          GamA102v022 := bhGA102v022
          GamA101v021 := bhGA101v021
```

## Fluorescence spectrum

```
In[407]:= cravaBhalla = fluorescencecrateranalysis[pulseenergy, omegaX, tauX, nintdata];
```

First Length[configurations] elements are the probability:

```
In[408]:= probBhalla = cravaBhalla[[1 ;; 63]]
Out[408]:= {0.913102, 0.00182067, 0., 0., 0.0183746, 0., 0., 0., 0., 0., 0.00761663, 0., 0., 0.,
  0., 0., 0., 0., 0.00915533, 0., 0., 0., 0., 0., 0., 0., 0.00421855, 0., 0.,
  0., 0., 0., 0., 0., 0.00573017, 0., 0., 0., 0., 0., 0., 0.00344751,
  0.,  $1.01351 \times 10^{-100}$ ,  $1.54507 \times 10^{-95}$ ,  $2.04334 \times 10^{-193}$ , 0., 0., 0., 0.0184594,
  0., 0.,  $5.95681 \times 10^{-245}$ ,  $1.11192 \times 10^{-238}$ , 0., 0.0180746, 0., 0.,  $3.0724 \times 10^{-7}$ }
```

```
In[409]:= Table[{configurations[[i]], prob[[i]], probBhalla[[i]]},
  {i, terminalcfg}] // TableForm
```

```
Out[409]//TableForm=
  226    0.913102    0.913102
  225    0.00177374  0.00182067
  224    0.0183612   0.0183746
  223    0.0075726   0.00761663
  222    0.00919243   0.00915533
  221    0.00418371   0.00421855
  220    0.0057461    0.00573017
  210    0.00324725   0.00344751
  200    0.0177446    0.0184594
  100    0.019076     0.0180746
  000     $2.20563 \times 10^{-7}$    $3.0724 \times 10^{-7}$ 
```

Second Length[configurations] elements are the probability action:

```
In[410]:= probactionBhalla = cravaBhalla[[64 ;; 126]]
Out[410]:= { $3.77489 \times 10^{15}$ ,  $7.52688 \times 10^{12}$ , 2162.02, 7.05584,  $7.59632 \times 10^{13}$ , 17030., 3381.56,
  2.03848, 0.342856, 0.0690174,  $3.14882 \times 10^{13}$ , 14409.4, 2509.98, 3.45023,
  1.61135, 0.478314, 0.0209712, 0.00841288,  $3.78494 \times 10^{13}$ , 37738.1, 10136.7,
  1.37526, 1.36516, 0.356944, 0.0675405, 0.0377667, 0.01117,  $1.74401 \times 10^{13}$ ,
  41446.8, 11448.1, 2.09933, 3.29661, 1.57687, 0.0374056, 0.0497647, 0.0109968,
   $2.36893 \times 10^{13}$ , 188732., 55256.6, 0.899642, 3.40904, 1.83774, 0.100856, 0.199114,
  0.0706843,  $1.42525 \times 10^{13}$ , 169299., 0.663721, 17.6204, 11.7088, 0.0247321,
  0.283423, 0.089778,  $7.62944 \times 10^{13}$ ,  $1.91988 \times 10^{10}$ , 183.789, 0.000107942,
  0.0114934, 0.0108049,  $7.47227 \times 10^{13}$ , 387307., 0.0131538,  $1.27017 \times 10^9$ }
```

```
In[411]:= fluorescenceBhalla = fluorecencematrix.probactionBhalla;
```

```
In[412]:= spectrumFluorescenceBhalla =
  Table[{fluorecenceenergy[[i]] * HartreeToeV, fluorescenceBhalla[[i]]},
    {i, 1, Length[fluorescenceBhalla]}];
```

```
In[413]:= spectrumFluorescenceBhallaNorm = Table[{spectrumFluorescenceBhalla[[i, 1]],
  1/Total[spectrumFluorescenceBhalla[[;;, 2]]] *
  spectrumFluorescenceBhalla[[i, 2]]},
  {i, 1, Length[spectrumFluorescenceBhalla]}];
```

```

In[414]:= ListPlot[{spectrumFluorescenceNorm, spectrumFluorescenceBhallaNorm},
  PlotRange → {{10, 40}, {0, 0.2}}, Filling → Bottom, FillingStyle → Thick,
  PlotMarkers → {Automatic, Small}, PlotStyle → {{Black, Thick}, {Red, Thick}},
  AxesLabel → {"", "y(ω)"}, LabelStyle → {FontFamily → "Helvetica", FontSize → 14},
  AxesStyle → {Medium, Arrowheads[Automatic]]]

```

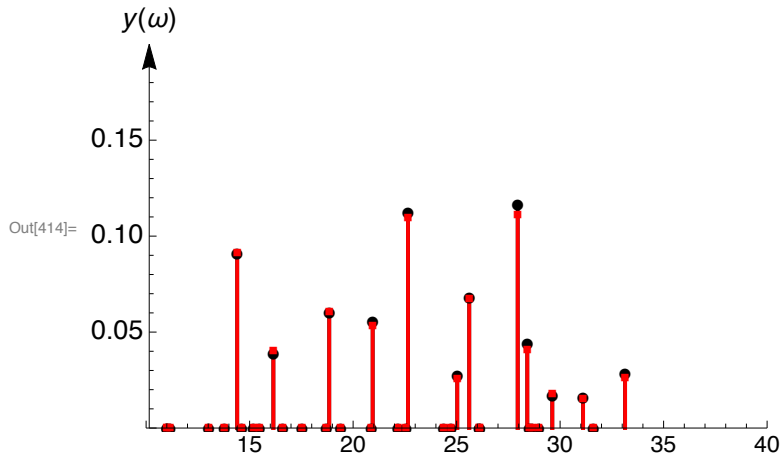

```

In[415]:= ListPlot[{spectrumFluorescenceNorm, spectrumFluorescenceBhallaNorm},
  PlotRange → {{840, 930}, {0, 0.2}}, Filling → Bottom, FillingStyle → Thick,
  PlotMarkers → {Automatic, Small}, PlotStyle → {{Black, Thick}, {Red, Thick}},
  Axes → {True, False}, AxesLabel → {"ω [eV]", ""},
  LabelStyle → {FontFamily → "Helvetica", FontSize → 14},
  AxesStyle → Arrowheads[Automatic]]]

```

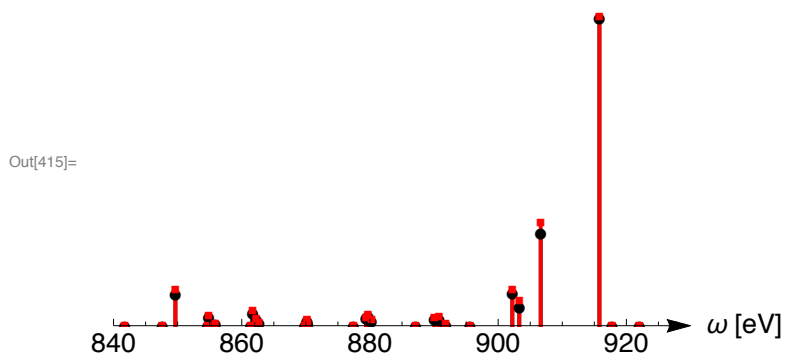

```
In[416]:= ListLogPlot[{spectrumFluorescenceNorm, spectrumFluorescenceBhallaNorm},
  PlotRange -> {{800, 1050}, {0.00001, 1}}, Filling -> Bottom,
  FillingStyle -> {{Thick}, {Thin}}, PlotMarkers -> {Automatic, Small},
  PlotStyle -> {{Black, Thick}, {Red, Thick}}, AxesLabel -> {" $\omega$  [eV]", ""},
  LabelStyle -> {FontFamily -> "Helvetica", FontSize -> 14},
  AxesStyle -> Arrowheads[Automatic]]
```

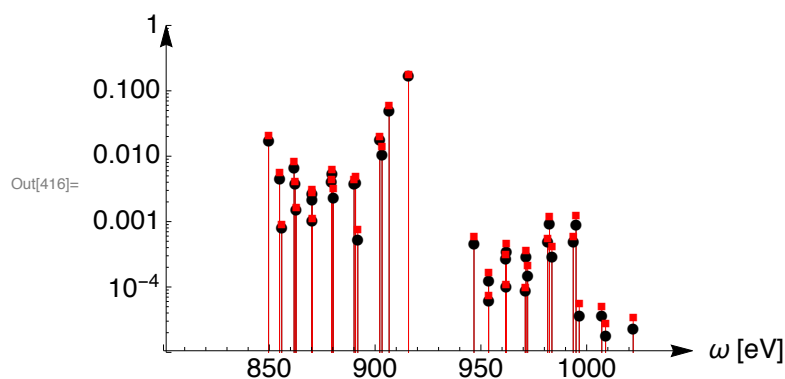

```
In[417]:= spectrumFluorescenceBhallaStates = Table[{i, fluorescencetransitions[[i]],
  fluorecenceenergy[[i]] * HartreeToeV, spectrumFluorescenceNorm[[i, 2]],
  spectrumFluorescenceBhallaNorm[[i, 2]]}, {i, 1, 100}];
```

```
In[418]:= Sort[spectrumFluorescenceBhallaStates, #1[[4]] > #2[[4]] &][[1 ;; 20]] // TableForm
```

Out[418]//TableForm=

|    |       |       |       |       |       |       |       |         |            |         |
|----|-------|-------|-------|-------|-------|-------|-------|---------|------------|---------|
| 90 | 1s(1) | 2s(0) | 2p(1) | ----> | 1s(2) | 2s(0) | 2p(0) | 915.795 | 0.172823   | 0.17319 |
| 4  | 1s(2) | 2s(1) | 2p(5) | ----> | 1s(2) | 2s(2) | 2p(4) | 27.9511 | 0.116684   | 0.11125 |
| 27 | 1s(2) | 2s(1) | 2p(3) | ----> | 1s(2) | 2s(2) | 2p(2) | 22.6515 | 0.112698   | 0.10955 |
| 59 | 1s(2) | 2s(1) | 2p(1) | ----> | 1s(2) | 2s(2) | 2p(0) | 14.4009 | 0.0912076  | 0.09127 |
| 13 | 1s(2) | 2s(1) | 2p(4) | ----> | 1s(2) | 2s(2) | 2p(3) | 25.6103 | 0.0685135  | 0.06738 |
| 43 | 1s(2) | 2s(1) | 2p(2) | ----> | 1s(2) | 2s(2) | 2p(1) | 18.8468 | 0.0603013  | 0.06045 |
| 60 | 1s(2) | 2s(0) | 2p(2) | ----> | 1s(2) | 2s(1) | 2p(1) | 20.9451 | 0.0559901  | 0.05313 |
| 89 | 1s(1) | 2s(1) | 2p(0) | ----> | 1s(2) | 2s(0) | 2p(0) | 906.634 | 0.0517697  | 0.05778 |
| 28 | 1s(2) | 2s(0) | 2p(4) | ----> | 1s(2) | 2s(1) | 2p(3) | 28.4145 | 0.0445603  | 0.04056 |
| 75 | 1s(2) | 2s(0) | 2p(1) | ----> | 1s(2) | 2s(1) | 2p(0) | 16.1478 | 0.0393364  | 0.04009 |
| 5  | 1s(2) | 2s(0) | 2p(6) | ----> | 1s(2) | 2s(1) | 2p(5) | 33.1401 | 0.0286768  | 0.02613 |
| 44 | 1s(2) | 2s(0) | 2p(3) | ----> | 1s(2) | 2s(1) | 2p(2) | 25.0309 | 0.0273932  | 0.02575 |
| 80 | 1s(1) | 2s(0) | 2p(2) | ----> | 1s(2) | 2s(0) | 2p(1) | 902.212 | 0.0183007  | 0.01999 |
| 2  | 1s(1) | 2s(2) | 2p(6) | ----> | 1s(2) | 2s(2) | 2p(5) | 849.65  | 0.0175113  | 0.02025 |
| 1  | 1s(2) | 2s(1) | 2p(6) | ----> | 1s(2) | 2s(2) | 2p(5) | 29.6225 | 0.0174392  | 0.01763 |
| 14 | 1s(2) | 2s(0) | 2p(5) | ----> | 1s(2) | 2s(1) | 2p(4) | 31.1105 | 0.0162026  | 0.01495 |
| 77 | 1s(1) | 2s(1) | 2p(1) | ----> | 1s(2) | 2s(1) | 2p(0) | 903.298 | 0.0107113  | 0.01363 |
| 15 | 1s(1) | 2s(2) | 2p(4) | ----> | 1s(2) | 2s(2) | 2p(3) | 861.711 | 0.00687855 | 0.00826 |
| 47 | 1s(1) | 2s(1) | 2p(3) | ----> | 1s(2) | 2s(1) | 2p(2) | 879.7   | 0.00554705 | 0.00615 |
| 6  | 1s(1) | 2s(2) | 2p(5) | ----> | 1s(2) | 2s(2) | 2p(4) | 854.849 | 0.00468699 | 0.00546 |

## References

- [1] Christian Buth, Ji-Cai Liu, Mau Hsiung Chen, James P. Cryan, Li Fang, James M. Glowina, Matthias Hoener, Ryan N. Coffee, Nora Berrah, *Ultrafast absorption of intense x rays by nitrogen molecules*, J. Chem. Phys. **136**, 214310 (2012), <http://dx.doi.org/10.1063/1.4722756>.
- [2] Y. Hikosaka, T. Kaneyasu, P. Lablanquie, F. Penent, E. Shigemasa, K. Ito, *Multiple Auger decay of the neon 1s-core-hole state studied by multielectron coincidence spectroscopy*, Phys. Rev. A **92**, 033413 (2015), <http://dx.doi.org/10.1103/PhysRevA.92.033413>.

- [3] N. Saito, I. H. Suzuki, *Shake-off processes in photoionization and Auger transition for rare gases irradiated by soft X-rays*, Phys. Scr. **49**, 80–85 (1994), <http://dx.doi.org/10.1088/0031-8949/49/1/011>.
- [4] B. Kanngießer, M. Jainz, S. Brünken, W. Benten, C. Gerth, K. Godehusen, K. Tiedtke, P. van Kampen, A. Tutay, P. Zimmermann, V. F. Demekhin, A. G. Kochur, Phys. Rev. A **62**, 14702 (2000), <http://dx.doi.org/10.1103/PhysRevA.62.014702>.
