# Supplementary material for: Neon in ultrashort and intense x rays from free electron lasers
Source: arXiv:1705.07521 ancillary file (2022-11-07)
Supplement: Supplementary file 3 [file neon_ion_yields.pdf]

```
In[1]:= Get["NeonRateEquations.m", Path -> NotebookDirectory[]]
```

```
In[2]:= HartreeToeV := 27.2113845
eVToHartree := 1/HartreeToeV
JouleToHartree := 2.29371269*^17
MilliJouleToHartree := 1*^-3 * JouleToHartree
BohrToAngstroem := 0.5291772083
AngstroemToBohr := 1/BohrToAngstroem
MicrometerToBohr := 1*^4 * AngstroemToBohr
BohrToMicrometer := 1/MicrometerToBohr
t0ToSecond := 24.18884326505*^-18
t0ToFemtoSecond := 24.18884326505*^-3
FemtoSecondTot0 := 1/t0ToFemtoSecond
crossSectionAUtoBarn := 1*^8 * BohrToAngstroem^2
crossSectionAUtocm2 := crossSectionAUtoBarn * 1*^-24
crossSectioncm2toAU := 1/crossSectionAUtocm2
intensityAUtoSI := 6.436409085121321*^15
intensitySItoAU := 1/intensityAUtoSI
```

```
In[18]:= neginfinity := -10 000 * FemtoSecondTot0
posinfinity := 10 000 * FemtoSecondTot0
```

# Ion yields from a neon atom in LCLS radiation

Christian Buth, 10 May 2017

Theoretische Chemie, Physikalisch-Chemisches Institut, Ruprecht-Karls-Universität Heidelberg, Im  
Neuenheimer Feld 229, 69120 Heidelberg, Germany

---

## Experimental ion yields

Figure 2b of Ref. [4]:

```
In[20]:= doumyexpt1110eV := {0.01877, 0.2267, 0.09675,
    0.1184, 0.06643, 0.09820, 0.1444, 0.2267, 0.04910, 0.0}
doumytheoryplain1110eV := {0.02744, 0.3033, 0.02455, 0.1430,
    0.02455, 0.09242, 0.1083, 0.2801, 0.007220, 0.0}
doumytheoryshake1110eV := {0.02744, 0.2440, 0.07798, 0.1227,
    0.04621, 0.07942, 0.1603, 0.2455, 0.005776, 0.0}
```

Figure 2a of Ref. [4]:

```
In[23]:= doumyexpt1225eV := {0.03321, 0.2614, 0.1011,
  0.1300, 0.06787, 0.07942, 0.07365, 0.1747, 0.08087, 0}
doumytheoryplain1225eV := {0.02888, 0.3264, 0.02599,
  0.1516, 0.02455, 0.09820, 0.03033, 0.1776, 0.1343, 0}
doumytheoryshake1225eV := {0.02744, 0.2643, 0.08231,
  0.1300, 0.04910, 0.08376, 0.04477, 0.1950, 0.1227, 0}
```

Figure 2b, upper panel, of Ref. [5]:

```
In[26]:= youngexpt800eV := {0.4880, 0.2483, 0.1455,
  0.07604, 0.03461, 0.01252, 0.006198, 0, 0.007596, 0.008302}
youngtheory800eV := {0.4777, 0.2486, 0.1493, 0.08152,
  0.03839, 0.01450, 0.006458, 0, 0.007831, 0.008525}
```

Figure 2b, middle panel, of Ref. [5]:

```
In[28]:= youngexpt1050eV := {0.04235, 0.2378, 0.08235,
  0.08480, 0.04340, 0.1108, 0.2448, 0.1490, 0.01636, 0.008289}
youngtheory1050eV := {0.01629, 0.2205, 0.01768, 0.1061,
  0.02433, 0.4198, 0.1801, 0.02642, 0.006065, 0.008512}
```

Figure 2b, lower panel, of Ref. [5]:

```
In[30]:= youngexpt2000eV := {0.04542, 0.3144, 0.1170, 0.1205,
  0.06288, 0.07162, 0.05590, 0.09432, 0.07162, 0.03144}
youngtheory2000eV := {0.03180, 0.3890, 0.02970, 0.1852,
  0.02761, 0.1153, 0.02899, 0.1097, 0.08082, 0.04148}
```

## LCLS x-ray pulse

### Temporal profile

LCLS FWHM pulse duration:

```
In[32]:= tauX := 100 * FemtoSecondTot0
```

Gaussian x-ray flux pulse shape (See Eq. (7) in Ref. [1]):

```
In[33]:= jxgaussian[J0Xj_, tX_, t_] :=
  J0Xj * Exp[-4 * Log[2] * (t/tX)^2] * UnitStep[t + 2 * tX] * UnitStep[2 * tX - t]
```

### Crater profile

FWHM of the crater profile:

```
In[34]:= rhoXx:=2*MicrometerToBohr
rhoYy:=1*MicrometerToBohr
```

The crater is normalized to unity with respect to an integration over the whole xy plane:

```
In[36]:= craterX[rx_] := 1/rhoXx/Sqrt[Pi/Log[16]] * Exp[-4*Log[2] * (rx/rhoXx)^2]
craterY[ry_] := 1/rhoYy/Sqrt[Pi/Log[16]] * Exp[-4*Log[2] * (ry/rhoYy)^2]
crater[rx_,ry_] := craterX[rx]*craterY[ry]
```

Number of radial integration points for the crater integration:

```
In[39]:= nintdata:=100
```

## Fluence profile

Number of x-ray photons for "monochromatic" light pulses:

```
In[40]:= numXRays[pulseenergy_,photonenergy_] := pulseenergy/photonenergy
```

X-ray fluence, i.e., the number of photos per squaremeter:

```
In[41]:= fluence[pulseenergy_,photonenergy_,rx_,ry_] := numXRays[pulseenergy,photonenergy]*crater
```

```
In[42]:= peakfluence[pulseenergy_,photonenergy_] := fluence[pulseenergy,photonenergy,0,0]
```

The peak x-ray flux at a point in the beam area:

```
In[43]:= J0Xfun[pulseenergy_,photonenergy_,tauX_,rx_,ry_] := 2*Sqrt[Log[2]/Pi]/tauX*fluence[pulse
```

Gaussian x-ray flux pluse shape:

```
In[44]:= jxgaussian[J0Xj_,tX_,t_] := J0Xj*Exp[-4*Log[2] * (t/tX)^2]*UnitStep[t+2*tX]*UnitStep[2*tX-
```

## Crater integration of ion yields from a single neon atom

All charge states:

```
In[45]:= ionyields[sol_] := {solNeutral[sol,posinfinity],solSingly[sol,posinfinity],solDoubly[sol,
solTriply[sol,posinfinity],solQuadruply[sol,posinfinity],solQuintuply[sol,posi
solSextuply[sol,posinfinity],solSeptuply[sol,posinfinity],solOctuply[sol,posin
solNonuply[sol,posinfinity],solDecuply[sol,posinfinity]}
```

Compute ion yields for a fraction of the peak x-ray fluences on the beam axis:

```
In[46]:= ionprofile[pulseenergy_,photonenergy_,tauX_,nintsteps_,nint_] := Module[{J0Xpeak,J0Xcur,
J0Xpeak=2*Sqrt[Log[2]/Pi]/tauX*peakfluence[pulseenergy,photonenergy];
J0Xcur=J0Xpeak/nintsteps*nint;
jxcrater[t_] := jxgaussian[J0Xcur,tauX,t];
sol=solveRateEquations[photonenergy,jxcrater,neginfinity,posinfinity,1/3000];
Join[{J0Xcur},ionyields[sol]]
]
```

```
In[47]:= tabionprof[pulseenergy_,photonenergy_,tauX_,nintsteps_]:=Module[{nint},
  Table[ionprofile[pulseenergy,photonenergy,tauX,nintsteps,nint],
    {nint,nintsteps,0,-1}]
]
```

Create interpolation functions for all charge states:

```
In[48]:= interpolYields[tabdata_]:=Module[{nint},
  Table[
    ListInterpolation[tabdata[[All,nint]],{tabdata[[All,1]]}],
    {nint,2,Length[tabdata[[1]]]}]
]
```

Evaluate all ion yields at a specific spatial point:

```
In[49]:= ionyieldint[funyields_,pulseenergy_,photonenergy_,tauX_,rx_,ry_]:=Module[{jj0x,nint},
  jj0x=J0Xfun[pulseenergy,photonenergy,tauX,rx,ry];
  Table[funyields[[nint]][jj0x],{nint,1,Length[funyields]}]
]
```

Integration of the ion yields of the beam area. The integral needs to be normalized to the integration area:

```
In[50]:= ionyieldbeam[funyields_, pulseenergy_, photonenergy_, tauX_] :=
  1 / ((2 * 5 * MicrometerToBohr) ^ 2) *
  NIntegrate[ionyieldint[funyields, pulseenergy, photonenergy, tauX, rx, ry],
    {rx, -5 * MicrometerToBohr, 5 * MicrometerToBohr}, {ry, -5 * MicrometerToBohr,
      5 * MicrometerToBohr}, MaxRecursion -> 20, Method -> "LocalAdaptive"]
```

```
In[51]:= ionyieldcrateranalysis[pulseenergy_,photoenergy_,pulseduration_,nint_]:=Module[{tabion},
  tabionyi=tabionprof[pulseenergy,photoenergy,pulseduration,nint];
  funionyi=interpolYields[tabionyi];
  ionyieldbeam[funionyi,pulseenergy,photoenergy,pulseduration]
]
```

## Ion yields from the plain rate equations

### Doumy data 1110 eV

Young data 1050 eV damping:  $0.699 / 3 = 0.233$

```
In[54]:= optdamp := 0.699 / 3
pulseenergy := optdamp * 1.27 * MilliJouleToHartree
omegaX := 1110 * eVToHartree
tauX := 100 * FemtoSecondTot0
rhoXx := 1 * MicrometerToBohr
rhoYy := 2 * MicrometerToBohr
```

```
In[60]:= ionyi = ionyieldcrateranalysis[pulseenergy, omegaX, tauX, nintdata];
ionyinorm = 1/Total[ionyi[[2 ;;]]] * ionyi[[2 ;;]]
```

```
Out[61]:= {0.0277336, 0.307386, 0.0285334, 0.150099, 0.0264165,
0.114911, 0.102137, 0.242226, 0.000557375, 7.16262 × 10-12}
```

```
In[52]:= theoryplain1110eV := {0.02773362066028239`,
0.3073855410174069`, 0.028533415145271204`, 0.15009900528630182`,
0.026416465072749782`, 0.11491137339204098`, 0.102137344156741`,
0.24222586075572966`, 0.000557374506313544`, 7.162618871618358`*-12}
```

```
In[63]:= tabionyi = Table[{doumyexpt1110eV[[i]],
doumytheoryplain1110eV[[i]], ionyinorm[[i]]}, {i, 1, 10}];
```

```
In[64]:= BarChart[tabionyi, PlotRange → All,
ChartLabels → {Placed[{"Ne+", "Ne2+", "Ne3+", "Ne4+", "Ne5+", "Ne6+",
"Ne7+", "Ne8+", "Ne9+", "Ne10+"}, Below], Placed[{}], Above]},
AxesLabel → {"", "Y"}, AxesStyle → {AbsoluteThickness[0.8],
{Arrowheads[Automatic], AbsoluteThickness[0.8]}},
LabelStyle → {FontFamily → "Helvetica", FontSize → 14},
ChartLegends → Placed[{"Experiment", "Theory Doumy", "Theory CAESR"}, Bottom]]
```

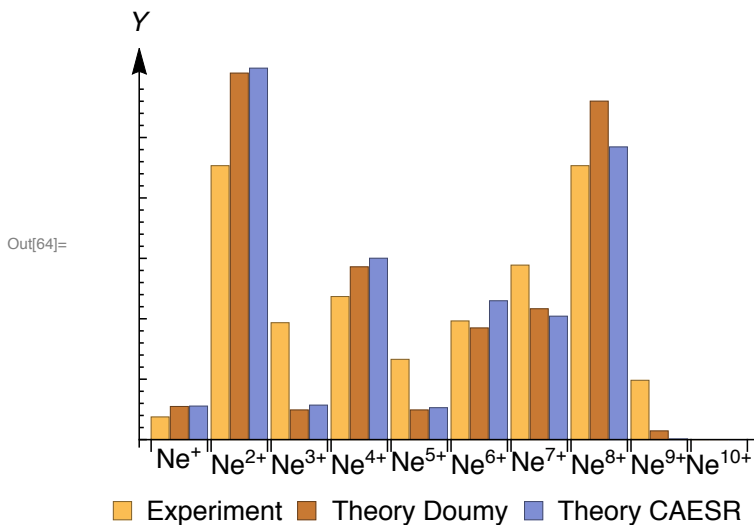

## Doumy data 1225 eV

Young data 1050 eV damping: 0.699 / 3 = 0.233

```
In[65]:= optdamp := 0.699 / 3
pulseenergy := optdamp * 1.45 * MilliJouleToHartree
omegaX := 1225 * eVToHartree
tauX := 100 * FemtoSecondTot0
rhoXx := 1 * MicrometerToBohr
rhoYy := 2 * MicrometerToBohr
```

```
In[71]:= ionyi = ionyieldcrateranalysis[pulseenergy, omegaX, tauX, nintdata];
ionyinorm = 1/Total[ionyi[[2 ;;]]] * ionyi[[2 ;;]]
```

```
Out[72]= {0.0286603, 0.326748, 0.0291796, 0.15873, 0.0264293,
0.0964488, 0.0267622, 0.153249, 0.153793, 2.30551 × 10-7}
```

```
In[53]:= theoryplain1225eV := {0.02866033964420429`,
0.32674760819974086`, 0.029179608660893374`, 0.1587299232256419`,
0.026429321303565748`, 0.09644884123093148`, 0.02676223122775317`,
0.15324865693646972`, 0.1537932390201907`, 2.3055060876278903`*^-7}
```

```
In[74]:= tabionyi = Table[{doumyexpt1225eV[[i]],
doumytheoryplain1225eV[[i]], ionyinorm[[i]]}, {i, 1, 10}];
```

```
In[75]:= BarChart[tabionyi, PlotRange → All,
ChartLabels → {Placed[{"Ne+", "Ne2+", "Ne3+", "Ne4+", "Ne5+", "Ne6+",
"Ne7+", "Ne8+", "Ne9+", "Ne10+"}, Below], Placed[{}], Above]},
AxesLabel → {"", "Y"}, AxesStyle → {AbsoluteThickness[0.8],
{Arrowheads[Automatic], AbsoluteThickness[0.8]}},
LabelStyle → {FontFamily → "Helvetica", FontSize → 14},
ChartLegends → Placed[{"Experiment", "Theory Doumy", "Theory CAESR"}, Bottom]]
```

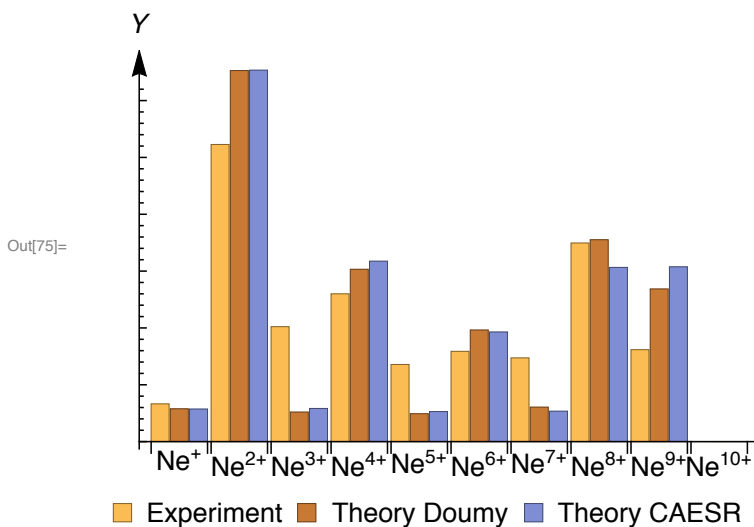

## Young data 800 eV

```
In[76]:= optdamp := 0.663/3
pulseenergy := optdamp * 2.4 * MilliJouleToHartree
omegaX := 800 * eVToHartree
tauX := 340 * FemtoSecondTot0
rhoXx := 1 * MicrometerToBohr
rhoYy := 2 * MicrometerToBohr
```

```
In[82]:= ionyi = ionyieldcrateranalysis[pulseenergy, omegaX, tauX, nintdata];
ionyinorm = 1/Total[ionyi[[2 ;;]]] * ionyi[[2 ;;]]
```

```
Out[83]= {0.435716, 0.255377, 0.171323, 0.0910379,
0.0351978, 0.00940381, 0.00177819, 0.000165801, 0., 0.}
```

```
In[54]:= theoryplain800eV :=
{0.43571632549838224`, 0.255377145799351`, 0.17132301747083567`,
0.09103788785724379`, 0.035197819154662885`, 0.009403814576120145`,
0.0017781886173969252`, 0.00016580102600747732`, 0., 0.}
```

```
In[85]:= tabionyi = Table[
{youngexpt800eV[[i]], youngtheory800eV[[i]], ionyinorm[[i]]}, {i, 1, 10}];
```

```
In[86]:= BarChart[tabionyi, PlotRange → All,
ChartLabels → {Placed[{"Ne+", "Ne2+", "Ne3+", "Ne4+", "Ne5+", "Ne6+", "Ne7+", "Ne8+",
"Ne9+", "Ne10+"}, Below], Placed[{}, Above]}, AxesLabel → {"", "Y"},
AxesStyle → {{Arrowheads[Automatic], AbsoluteThickness[0.6]},
{Arrowheads[Automatic], AbsoluteThickness[0.6]}},
LabelStyle → {FontFamily → "Helvetica", FontSize → 14}]
```

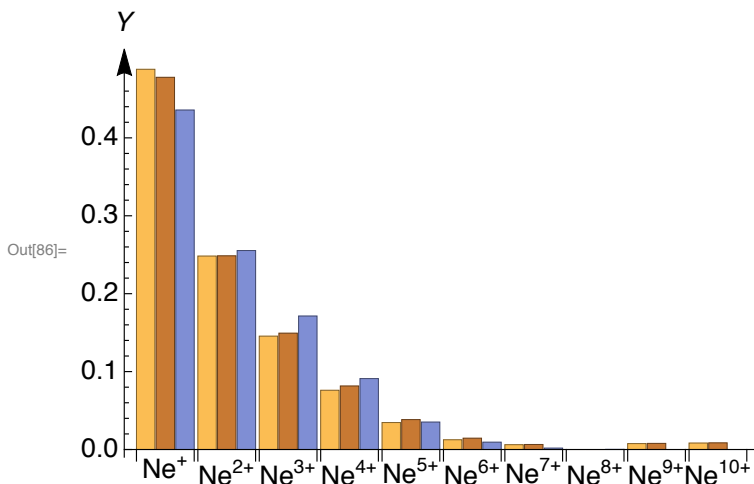

## Young data 1050 eV

```
In[87]:= optdamp := 0.699/3
pulseenergy := optdamp * 2.4 * MilliJouleToHartree
omegaX := 1050 * eVToHartree
tauX := 280 * FemtoSecondTot0
rhoXx := 1 * MicrometerToBohr
rhoYy := 2 * MicrometerToBohr
```

```
In[93]:= ionyi = ionyieldcrateranalysis[pulseenergy, omegaX, tauX, nintdata];
ionyinorm = 1/Total[ionyi[[2 ;;]]] * ionyi[[2 ;;]]
```

```
Out[94]= {0.0228886, 0.24715, 0.0236598, 0.121835, 0.0323053,
0.379241, 0.153796, 0.0191182, 6.37775 × 10-6, 2.55783 × 10-17}
```

```
In[55]:= theoryplain1050eV := {0.022888553304354253`, 0.24715002207907782`,
  0.023659803095957933`, 0.1218348890578218`, 0.0323052889558537`,
  0.3792411902043192`, 0.15379567180665624`, 0.01911820374218655`,
  6.377753772559972`*^-6, 2.5578272556430032`*^-17}
```

```
In[96]:= tabionyi = Table[
  {youngexpt1050eV[[i]], youngtheory1050eV[[i]], ionyinorm[[i]]}, {i, 1, 10}];
```

```
In[97]:= BarChart[tabionyi, PlotRange → All,
  ChartLabels → {Placed[{"Ne+", "Ne2+", "Ne3+", "Ne4+", "Ne5+", "Ne6+", "Ne7+", "Ne8+",
    "Ne9+", "Ne10+"}, Below], Placed[{}, Above]}, AxesLabel → {"", "Y"},
  AxesStyle → {{Arrowheads[Automatic], AbsoluteThickness[0.6]},
    {Arrowheads[Automatic], AbsoluteThickness[0.6]}},
  LabelStyle → {FontFamily → "Helvetica", FontSize → 14}]
```

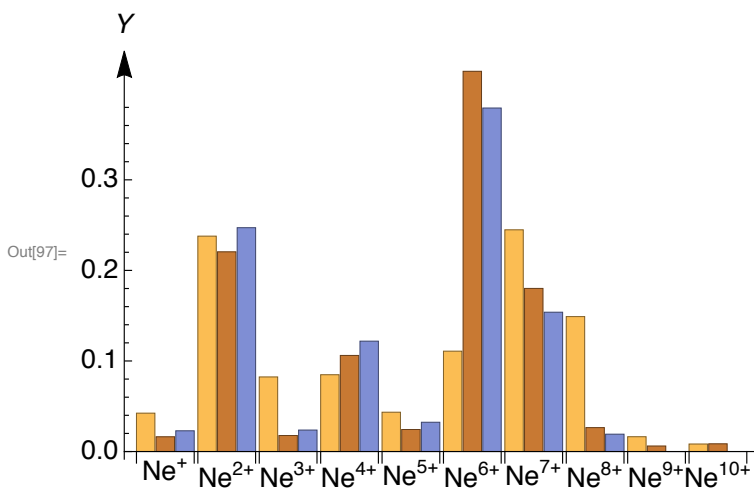

## Young data 2000 eV

### Original damping 0.584 / 3

```
In[98]:= optdamp := 0.584 / 3
pulseenergy := optdamp * 2.4 * MilliJouleToHartree
omegaX := 1999.999 * eVToHartree
tauX := 230 * FemtoSecondTot0
rhoXx := 1 * MicrometerToBohr
rhoYy := 2 * MicrometerToBohr
```

```
In[104]:= ionyi = ionyieldcrateranalysis[pulseenergy, omegaX, tauX, nintdata];
ionyinorm = 1 / Total[ionyi[[2 ;;]]] * ionyi[[2 ;;]]
```

```
Out[105]:= {0.0467493, 0.562197, 0.0369904, 0.208639, 0.0198109,
  0.0755012, 0.00903772, 0.0280486, 0.0107888, 0.00223687}
```



```
In[56]:= theoryplain2000eVo019 := {0.046749343487133777`,
  0.5621966441358869`, 0.03699039031953911`, 0.20863946217002846`,
  0.019810909991688434`, 0.07550121383278423`, 0.009037721209136824`,
  0.028048611945134926`, 0.01078883734872949`, 0.002236865559937846`}
```

```
In[107]:= tabionyi = Table[
  {youngexpt2000eV[[i]], youngtheory2000eV[[i]], ionyinorm[[i]]}, {i, 1, 10}];
```

```
In[108]:= BarChart[tabionyi, PlotRange → All,
  ChartLabels → {Placed[{"Ne+", "Ne2+", "Ne3+", "Ne4+", "Ne5+", "Ne6+", "Ne7+", "Ne8+",
    "Ne9+", "Ne10+"}, Below], Placed[{}, Above]}, AxesLabel → {"", "Y"},
  AxesStyle → {{Arrowheads[Automatic], AbsoluteThickness[0.6]},
    {Arrowheads[Automatic], AbsoluteThickness[0.6]}},
  LabelStyle → {FontFamily → "Helvetica", FontSize → 14}]
```

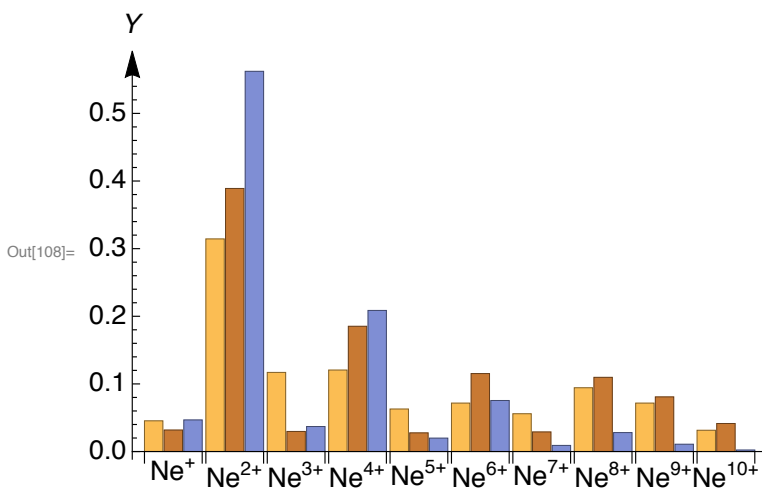

Adjusted damping 0.635, adjusted pulse duration 140 fs

```
In[109]:= optdamp := 0.635
pulseenergy := optdamp * 2.4 * MilliJouleToHartree
omegaX := 1999.999 * eVToHartree
tauX := 140 * FemtoSecondTot0
rhoXx := 1 * MicrometerToBohr
rhoYy := 2 * MicrometerToBohr
```

```
In[115]:= ionyi = ionyieldcrateranalysis[pulseenergy, omegaX, tauX, nintdata];
ionyinorm = 1 / Total[ionyi[[2 ;;]]] * ionyi[[2 ;;]]
```

```
Out[116]:= {0.0293679, 0.359196, 0.029966, 0.173315, 0.0263913,
  0.101803, 0.0235222, 0.0892322, 0.0939761, 0.0732303}
```

```
In[57]:= theoryplain2000eVo064 := {0.029367894211233307`,
  0.3591957086955541`, 0.029965973942764564`, 0.17331544215821076`,
  0.026391267577717686`, 0.10180282507831621`, 0.023522235126221695`,
  0.08923224643626439`, 0.09397607009999752`, 0.07323033667371982`}
```

```
In[118]:= tabionyi = Table[
  {youngexpt2000eV[[i]], youngtheory2000eV[[i]], ionyinorm[[i]]}, {i, 1, 10}];
In[119]:= BarChart[tabionyi, PlotRange → All,
  ChartLabels → {Placed[{"Ne+", "Ne2+", "Ne3+", "Ne4+", "Ne5+", "Ne6+", "Ne7+", "Ne8+",
    "Ne9+", "Ne10+"}, Below], Placed[{}, Above]}, AxesLabel → {"", "Y"},
  AxesStyle → {{Arrowheads[Automatic], AbsoluteThickness[0.6]},
    {Arrowheads[Automatic], AbsoluteThickness[0.6]}},
  LabelStyle → {FontFamily → "Helvetica", FontSize → 14}]
```

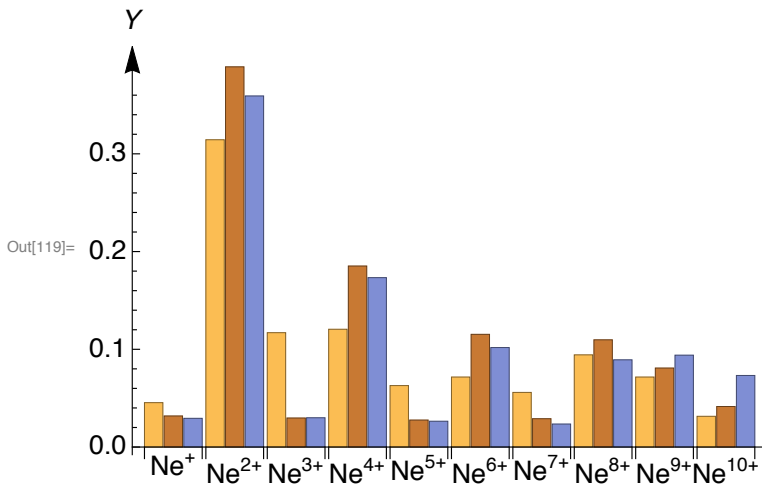

### Adjusted beam area, original damping 0.584 / 3

```
In[120]:= optdamp := 0.584 / 3
pulseenergy := optdamp * 2.4 * MilliJouleToHartree
omegaX := 1999.999 * eVToHartree
tauX := 230 * FemtoSecondTot0
rhoXx := 1 * MicrometerToBohr
rhoYy := rhoXx

In[126]:= ionyi = ionyildcrateranalysis[pulseenergy, omegaX, tauX, nintdata];
ionyinorm = 1 / Total[ionyi[[2 ;;]]] * ionyi[[2 ;;]]

Out[127]= {0.0352002, 0.429458, 0.0347199, 0.199912, 0.027551,
  0.105933, 0.0202564, 0.0699583, 0.0521829, 0.024828}
```

```
In[58]:= theoryplain2000eVo019beam := {0.03520016997678228`,
  0.4294578241598163`, 0.03471985075598394`, 0.19991235951940314`,
  0.02755102475468712`, 0.10593316813412958`, 0.02025636482959082`,
  0.0699583081307055`, 0.052182923985633234`, 0.02482800575326819`}
```

```
In[129]:= tabionyi = Table[
  {youngexpt2000eV[[i]], youngtheory2000eV[[i]], ionyinorm[[i]]}, {i, 1, 10}];
```

```
In[130]:= BarChart[tabionyi, PlotRange → All,
  ChartLabels → {Placed[{"Ne+", "Ne2+", "Ne3+", "Ne4+", "Ne5+", "Ne6+", "Ne7+", "Ne8+",
    "Ne9+", "Ne10+"}, Below], Placed[{}, Above]}, AxesLabel → {"", "Y"},
  AxesStyle → {{Arrowheads[Automatic], AbsoluteThickness[0.6]},
    {Arrowheads[Automatic], AbsoluteThickness[0.6]}},
  LabelStyle → {FontFamily → "Helvetica", FontSize → 14}]
```

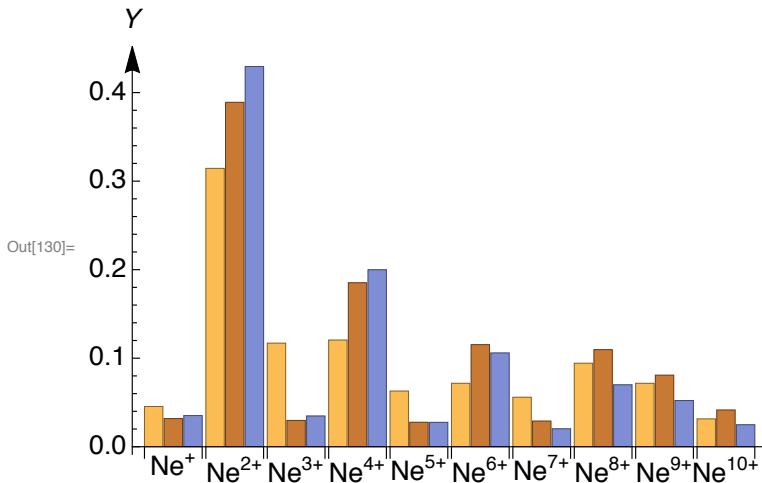

### Adjusted beam area, adjusted damping 0.25

```
In[131]:= optdamp := 0.25
pulseenergy := optdamp * 2.4 * MilliJouleToHartree
omegaX := 1999.999 * eVToHartree
tauX := 230 * FemtoSecondTot0
rhoXx := 1 * MicrometerToBohr
rhoYy := rhoXx

In[137]:= ionyi = ionyieldcrateranalysis[pulseenergy, omegaX, tauX, nintdata];
ionyinorm = 1/Total[ionyi[[2 ;;]]] * ionyi[[2 ;;]]

Out[138]= {0.0319735, 0.390634, 0.0322556, 0.186412, 0.0273603,
  0.10543, 0.0223464, 0.0805723, 0.0745614, 0.0484541}
```

```
In[59]:= theoryplain2000eVo025beam := {0.031973467506859025`,
  0.3906342744247116`, 0.032255594933307506`, 0.18641186310492208`,
  0.02736032486549449`, 0.10543030174976885`, 0.02234640124179485`,
  0.0805722684592051`, 0.07456137709147048`, 0.04845412662246604`}
```

```
In[140]:= tabionyi = Table[
  {youngexpt2000eV[[i]], youngtheory2000eV[[i]], ionyinorm[[i]]}, {i, 1, 10}];
```

```
In[141]:= BarChart[tabiony1, PlotRange → All,
  ChartLabels → {Placed[{"Ne+", "Ne2+", "Ne3+", "Ne4+", "Ne5+", "Ne6+", "Ne7+", "Ne8+",
    "Ne9+", "Ne10+"}, Below], Placed[{}, Above]}, AxesLabel → {"", "Y"},
  AxesStyle → {{Arrowheads[Automatic], AbsoluteThickness[0.6]},
    {Arrowheads[Automatic], AbsoluteThickness[0.6]}},
  LabelStyle → {FontFamily → "Helvetica", FontSize → 14}]
```

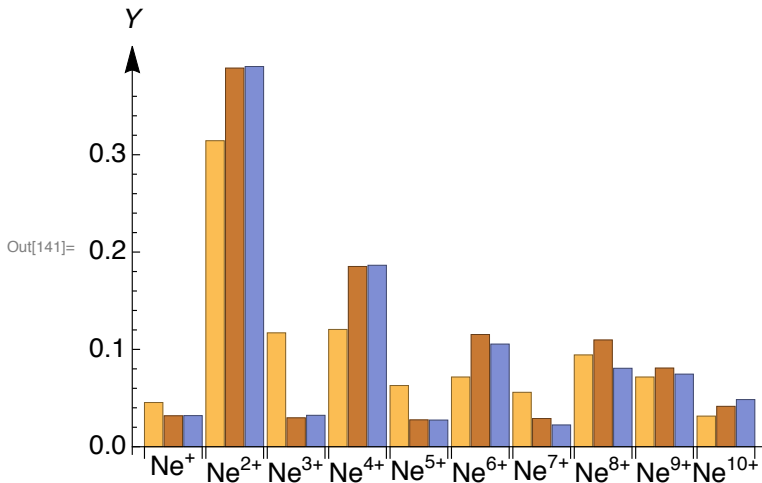

## Modified rate equations

```
In[72]:= Solve[a / (1 - a) == shake, a]
```

```
Out[72]= {{a →  $\frac{\text{shake}}{1 + \text{shake}}$ }}
```

Photoionization shake off from Table I of Ref. [3]:

```
In[73]:= valshakeoff :=  $\frac{0.16}{1 + 0.16}$ 
```

Photoionization shake off from Table III of Ref. [3]:

```
In[74]:= coresshakeoff :=  $\frac{0.23}{1 + 0.23}$ 
```

Double Auger decay partial probabilities from Table I of Ref. [2]:

```
In[75]:= p2pm3 := 2.5 / 100
p2sm12pm2 := 2.9 / 100
p2sm22pm1 := 0.5 / 100
pNem3 := p2pm3 + p2sm12pm2 + p2sm22pm1
```

Probabilities from Table I of Ref. [6]:

```
In[79]:= daNe2p := 0.9267
daNe3p := 0.0597
```

```
In[81]:= d = daNe3p / (daNe2p + daNe3p)
```

```
Out[81]= 0.0605231
```

In[82]:= 1 - d

Out[82]= 0.939477

Double Auger decay fractions:

In[83]:= da223v126 = p2pm3 / pNem3 \* d

Out[83]= 0.0256454

In[84]:= da214v126 = p2sm12pm2 / pNem3 \* d

Out[84]= 0.0297486

In[85]:= da205v126 = p2sm22pm1 / pNem3 \* d

Out[85]= 0.00512908

In[86]:= daTot126 := da223v126 + da214v126 + da205v126

## Multiple photoionization of the valence electrons

In[87]:= req225[en\_, jx\_] := P225'[t] == (1 - valshakeoff) \* xsc225v226[en] \* jx[t] \* P226[t] -  
xscTot225[en] \* jx[t] \* P225[t] + GamR225v216 \* P216[t] + GamR225v126 \* P126[t]

In[88]:= req216[en\_, jx\_] := P216'[t] == (1 - valshakeoff) \* xsc216v226[en] \* jx[t] \* P226[t] -  
xscTot216[en] \* jx[t] \* P216[t] + GamR216v126 \* P126[t] - GamRTot216 \* P216[t]

## Multiple photoionization of core and valence electrons

In[89]:= req126[en\_, jx\_] := P126'[t] == (1 - coreshakeoff) \* xsc126v226[en] \* jx[t] \* P226[t] -  
xscTot126[en] \* jx[t] \* P126[t] - GamATot126 \* P126[t] - GamRTot126 \* P126[t]

In[90]:= req125[en\_, jx\_] := P125'[t] == coreshakeoff \* xsc126v226[en] \* jx[t] \* P226[t] +  
xsc125v225[en] \* jx[t] \* P225[t] + xsc125v126[en] \* jx[t] \* P126[t] -  
xscTot125[en] \* jx[t] \* P125[t] - GamATot125 \* P125[t] +  
GamR125v116 \* P116[t] + GamR125v026 \* P026[t] - GamRTot125 \* P125[t]

## Double Auger decay

In[91]:= req224[en\_, jx\_] := P224'[t] ==  
valshakeoff \* xsc225v226[en] \* jx[t] \* P226[t] + xsc224v225[en] \* jx[t] \* P225[t] -  
xscTot224[en] \* jx[t] \* P224[t] + (1 - daTot126) \* GamA224v126 \* P126[t] +  
GamR224v215 \* P215[t] + GamR224v125 \* P125[t]

In[92]:= req215[en\_, jx\_] := P215'[t] ==  
valshakeoff \* xsc216v226[en] \* jx[t] \* P226[t] + xsc215v225[en] \* jx[t] \* P225[t] +  
xsc215v216[en] \* jx[t] \* P216[t] - xscTot215[en] \* jx[t] \* P215[t] +  
(1 - daTot126) \* GamA215v126 \* P126[t] + GamR215v206 \* P206[t] +  
GamR215v125 \* P125[t] + GamR215v116 \* P116[t] - GamRTot215 \* P215[t]

In[93]:= req206[en\_, jx\_] :=  
P206'[t] == xsc206v216[en] \* jx[t] \* P216[t] - xscTot206[en] \* jx[t] \* P206[t] +  
(1 - daTot126) \* GamA206v126 \* P126[t] + GamR206v116 \* P116[t] - GamRTot206 \* P206[t]

```

In[94]:= req223[en_, jx_] := P223'[t] == xsc223v224[en] * jx[t] * P224[t] -
      xscTot223[en] * jx[t] * P223[t] + da223v126 * GamATot126 * P126[t] +
      GamA223v125 * P125[t] + GamR223v214 * P214[t] + GamR223v124 * P124[t]

In[95]:= req214[en_, jx_] :=
      P214'[t] == xsc214v224[en] * jx[t] * P224[t] + xsc214v215[en] * jx[t] * P215[t] -
      xscTot214[en] * jx[t] * P214[t] + da214v126 * GamATot126 * P126[t] +
      GamA214v125 * P125[t] + GamA214v116 * P116[t] + GamR214v205 * P205[t] +
      GamR214v124 * P124[t] + GamR214v115 * P115[t] - GamRTot214 * P214[t]

In[96]:= req205[en_, jx_] :=
      P205'[t] == xsc205v215[en] * jx[t] * P215[t] + xsc205v206[en] * jx[t] * P206[t] -
      xscTot205[en] * jx[t] * P205[t] + da205v126 * GamATot126 * P126[t] +
      GamA205v125 * P125[t] + GamA205v116 * P116[t] +
      GamR205v115 * P115[t] + GamR205v106 * P106[t] - GamRTot205 * P205[t]

```

## Ion yields from the modified rate equations

### Doumy data 1110 eV

Young data 1050 eV damping:  $0.699 / 3 = 0.233$

```

In[167]:= optdamp := 0.699 / 3
pulseenergy := optdamp * 1.27 * MilliJouleToHartree
omegaX := 1110 * eVToHartree
tauX := 100 * FemtoSecondTot0
rhoXx := 1 * MicrometerToBohr
rhoYy := 2 * MicrometerToBohr

In[173]:= ionyi = ionyildcrateranalysis[pulseenergy, omegaX, tauX, nintdata];
ionyinorm = 1 / Total[ionyi[[2 ;;]]] * ionyi[[2 ;;]]

Out[174]:= {0.0236618, 0.239342, 0.099468, 0.120152, 0.0561308,
      0.0944512, 0.161036, 0.205293, 0.00046512, 1.3117 × 10-11}

In[60]:= theoryshake1110eV := {0.023661784312894934`, 0.2393417491540436`,
      0.09946800390982896`, 0.12015244846769116`, 0.05613081344654926`,
      0.09445116252851939`, 0.16103554310354887`, 0.2052933754006595`,
      0.00046511966314724307`, 1.311701151108976`*^-11}

In[176]:= Total[ionyi]

Out[176]:= 1.

In[177]:= tabionyi = Table[{doumyexpt1110eV[[i]],
      doumytheoryshake1110eV[[i]], ionyinorm[[i]]}, {i, 1, 10}];

```

```
In[178]:= BarChart[tabionyi, PlotRange → All,
  ChartLabels → {Placed[{"Ne+", "Ne2+", "Ne3+", "Ne4+", "Ne5+", "Ne6+",
    "Ne7+", "Ne8+", "Ne9+", "Ne10+"}, Below], Placed[{}, Above]},
  AxesLabel → {"", "Y"}, AxesStyle → {AbsoluteThickness[0.8],
    {Arrowheads[Automatic], AbsoluteThickness[0.8]}},
  LabelStyle → {FontFamily → "Helvetica", FontSize → 14},
  ChartLegends → Placed[{"Experiment", "Theory Doumy", "Theory CAESR"}, Bottom]]
```

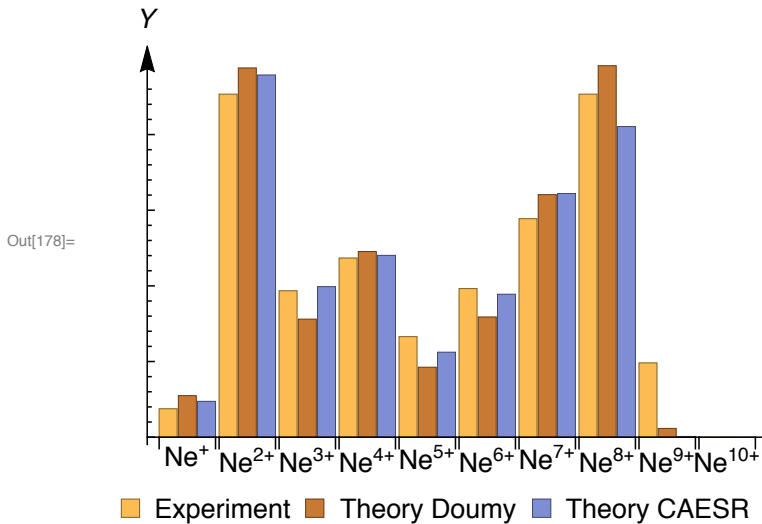

## Doumy data 1225 eV

Young data 1050 eV damping:  $0.699 / 3 = 0.233$

```
In[179]:= optdamp := 0.699 / 3
pulseenergy := optdamp * 1.45 * MilliJouleToHartree
omegaX := 1225 * eVToHartree
tauX := 100 * FemtoSecondTot0
rhoXx := 1 * MicrometerToBohr
rhoYy := 2 * MicrometerToBohr
```

```
In[185]:= ionyi = ionyieldcrateranalysis[pulseenergy, omegaX, tauX, nintdata];
ionyinorm = 1 / Total[ionyi[[2 ;;]]] * ionyi[[2 ;;]]
```

```
Out[186]= {0.0244456, 0.254286, 0.104633, 0.126883, 0.0576132,
  0.0790318, 0.0424713, 0.176186, 0.134449, 4.75453 × 10-7}
```

```
In[61]:= theoryshake1225eV := {0.024445593895711295`,
  0.2542858655181715`, 0.10463317071295399`, 0.1268834091170801`,
  0.05761324660896346`, 0.07903178154288742`, 0.04247130599897231`,
  0.17618567967489823`, 0.13444947147785358`, 4.7545250793408493` * 10-7}
```

```
In[188]:= Total[ionyi]
```

```
Out[188]= 1.
```

```
In[189]:= tabionyi = Table[{doumyexpt1225eV[[i]],
  doumytheoryshake1225eV[[i]], ionyinorm[[i]]}, {i, 1, 10}];
```

```
In[190]:= BarChart[tabionyi, PlotRange → All,
  ChartLabels → {Placed[{"Ne+", "Ne2+", "Ne3+", "Ne4+", "Ne5+", "Ne6+",
    "Ne7+", "Ne8+", "Ne9+", "Ne10+"}, Below], Placed[{}, Above]},
  AxesLabel → {"", "Y"}, AxesStyle → {AbsoluteThickness[0.8],
    {Arrowheads[Automatic], AbsoluteThickness[0.8]}},
  LabelStyle → {FontFamily → "Helvetica", FontSize → 14},
  ChartLegends → Placed[{"Experiment", "Theory Doumy", "Theory CAESR"}, Bottom]]
```

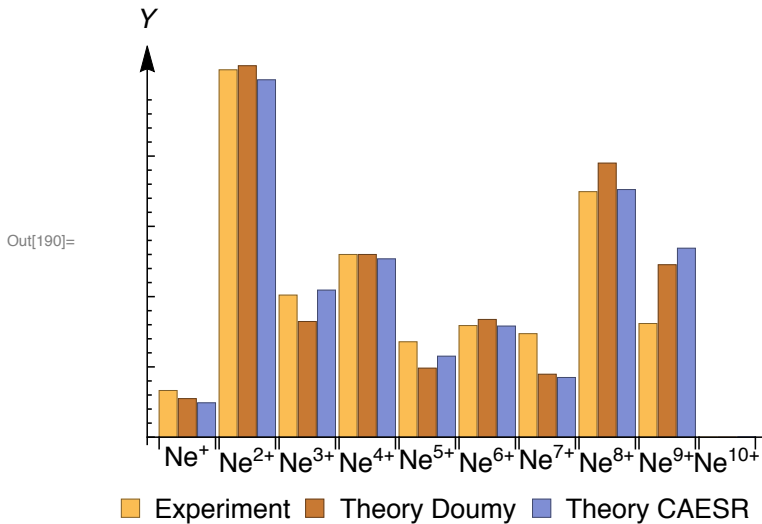

## Young data 800 eV

```
In[191]:= optdamp := 0.663 / 3
pulseenergy := optdamp * 2.4 * MilliJouleToHartree
omegaX := 800 * eVToHartree
tauX := 340 * FemtoSecondTot0
rhoXx := 1 * MicrometerToBohr
rhoYy := 2 * MicrometerToBohr

In[197]:= ionyi = ionyieldcrateranalysis[pulseenergy, omegaX, tauX, nintdata];
ionyinorm = 1 / Total[ionyi[[2 ;;]]] * ionyi[[2 ;;]]

Out[198]= {0.375618, 0.286078, 0.184387, 0.0999264,
  0.0402512, 0.0112731, 0.00224563, 0.000220995, 0., 0.}
```

```
In[62]:= theoryshake800eV :=
  {0.3756175189726977`, 0.2860777804276809`, 0.18438734377151983`,
    0.09992642276092975`, 0.040251189582459684`, 0.01127312072884545`,
    0.0022456283227884326`, 0.00022099543307843017`, 0., 0.}
```

```
In[200]:= Total[ionyi]
```

```
Out[200]= 1.
```

```
In[201]:= tabionyi = Table[
  {youngexpt800eV[[i]], theoryplain800eV[[i]], ionyinorm[[i]]}, {i, 1, 10}];
```



```
In[202]:= BarChart[tablyoni, PlotRange → {-0.05, 0.45},
  ChartLabels → {Placed[{"Ne+", "Ne2+", "Ne3+", "Ne4+", "Ne5+", "Ne6+", "Ne7+", "Ne8+",
    "Ne9+", "Ne10+"}, Below], Placed[{}, Above]}, AxesLabel → {"", "Y"},
  AxesStyle → {{Arrowheads[Automatic], AbsoluteThickness[0.6]},
    {Arrowheads[Automatic], AbsoluteThickness[0.6]}},
  LabelStyle → {FontFamily → "Helvetica", FontSize → 14}]
```

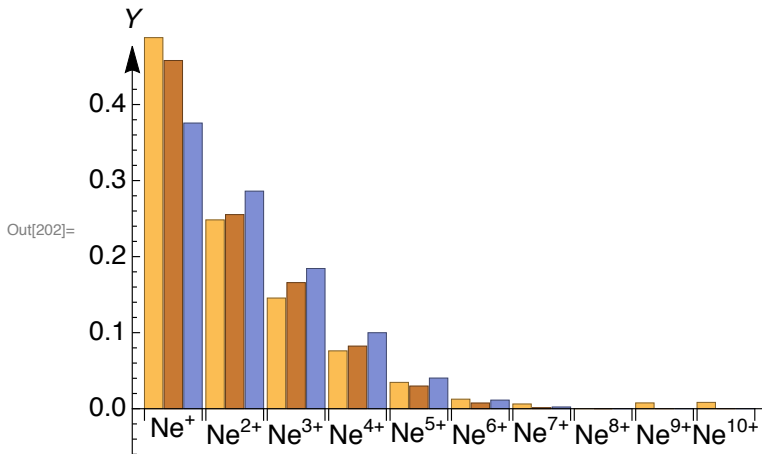

## Young data 1050 eV

```
In[203]:= optdamp := 0.699 / 3
pulseenergy := optdamp * 2.4 * MilliJouleToHartree
omegaX := 1050 * eVToHartree
tauX := 280 * FemtoSecondTot0
rhoXx := 1 * MicrometerToBohr
rhoYy := 2 * MicrometerToBohr

In[209]:= ioni = ionyieldcrateranalysis[pulseenergy, omegaX, tauX, nintdata];
ionynorm = 1 / Total[ioni[[2 ;;]]] * ioni[[2 ;;]]

Out[210]= {0.0195334, 0.192548, 0.0806604, 0.0975628, 0.0653195,
  0.313462, 0.204199, 0.0267037, 0.0000115419, 2.2938 × 10-17}
```

```
In[63]:= theoryshake1050eV := {0.01953343449577729`, 0.1925481214771152`,
  0.08066042995988204`, 0.0975627650448078`, 0.06531950438284863`,
  0.3134616188824682`, 0.204198868306359`, 0.02670371559565381`,
  0.000011541855088181606`, 2.2938009521743028` * ^-17}
```

```
In[212]:= Total[ioni]
```

```
Out[212]= 1.
```

```
In[213]:= tabiony = Table[
  {youngexpt1050eV[[i]], theoryplain1050eV[[i]], ionynorm[[i]]}, {i, 1, 10}];
```

```
In[214]:= BarChart[tabionyi, PlotRange → {-0.05, 0.45},
  ChartLabels → {Placed[{"Ne+", "Ne2+", "Ne3+", "Ne4+", "Ne5+", "Ne6+", "Ne7+", "Ne8+",
    "Ne9+", "Ne10+"}, Below], Placed[{}, Above]}, AxesLabel → {"", "Y"},
  AxesStyle → {{Arrowheads[Automatic], AbsoluteThickness[0.6]},
    {Arrowheads[Automatic], AbsoluteThickness[0.6]}},
  LabelStyle → {FontFamily → "Helvetica", FontSize → 14}]
```

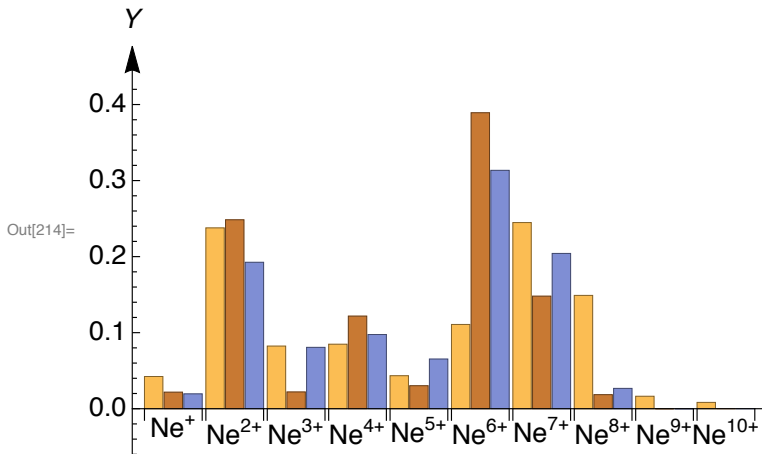

## Young data 2000 eV

### Original damping 0.584 / 3

```
In[215]:= optdamp := 0.584 / 3
pulseenergy := optdamp * 2.4 * MilliJouleToHartree
omegaX := 1999.999 * eVToHartree
tauX := 230 * FemtoSecondTot0
rhoXx := 1 * MicrometerToBohr
rhoYy := 2 * MicrometerToBohr

X-ray peak intensity:

In[221]:= J0Xfun[pulseenergy, omegaX, tauX, 0, 0] * omegaX * intensityAUtoSI
Out[221]= 8.4207 × 1016

In[222]:= ionyi = ionyieldcrateranalysis[pulseenergy, omegaX, tauX, nintdata];
ionyinorm = 1 / Total[ionyi[[2 ;;]]] * ionyi[[2 ;;]]
Out[223]= {0.0398482, 0.43697, 0.167696, 0.166091, 0.0621511,
  0.0614354, 0.0231968, 0.029786, 0.0108466, 0.00197818}

In[64]:= theoryshake2000eVo019 := {0.039848189564645184`,
  0.43697045088099257`, 0.16769645626997798`, 0.16609097144877094`,
  0.062151051046521216`, 0.06143535860875028`, 0.02319677944126449`,
  0.029785973571015072`, 0.01084659024867977`, 0.0019781789193824457`}
```

```
In[225]:= Total[ionyi]
```

```
Out[225]= 1.
```

```

In[226]:= tabionyi = Table[{youngexpt2000eV[[i]],
  theoryplain2000eVo019[[i]], ionyinorm[[i]]}, {i, 1, 10}];

In[227]:= BarChart[tabionyi, PlotRange → {-0.05, 0.45},
  ChartLabels → {Placed[{"Ne+", "Ne2+", "Ne3+", "Ne4+", "Ne5+", "Ne6+", "Ne7+", "Ne8+",
    "Ne9+", "Ne10+"}, Below], Placed[{}, Above]}, AxesLabel → {"", "Y"},
  AxesStyle → {{Arrowheads[Automatic], AbsoluteThickness[0.6]},
    {Arrowheads[Automatic], AbsoluteThickness[0.6]}},
  LabelStyle → {FontFamily → "Helvetica", FontSize → 14}]

```

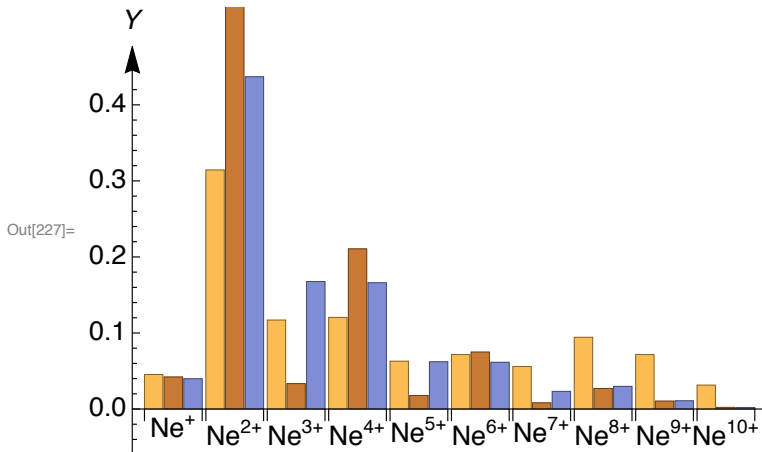

## Adjusted damping 0.635, adjusted pulse duration 140 fs

```

In[228]:= optdamp := 0.635
pulseenergy := optdamp * 2.4 * MilliJouleToHartree
omegaX := 1999.999 * eVToHartree
tauX := 140 * FemtoSecondTot0
rhoXx := 1 * MicrometerToBohr
rhoYy := 2 * MicrometerToBohr
X-ray peak intensity:

```

```

In[234]:= J0Xfun[pulseenergy, omegaX, tauX, 0, 0] * omegaX * intensityAUtoSI
Out[234]= 4.51264 × 1017

```

```

In[235]:= ionyi = ionyieldcrateranalysis[pulseenergy, omegaX, tauX, nintdata];
ionyinorm = 1 / Total[ionyi[[2 ;;]]] * ionyi[[2 ;;]]

```

```

Out[236]= {0.0250299, 0.279192, 0.113161, 0.138134, 0.0606067,
  0.0830378, 0.0407342, 0.0937906, 0.101076, 0.0652377}

```

```

In[65]:= theoryshake2000eVo064 := {0.025029938842445823`,
  0.2791919069303871`, 0.11316133778218797`, 0.1381339011793001`,
  0.06060674066153153`, 0.08303781516529352`, 0.04073415565225933`,
  0.09379063070966483`, 0.10107582831860605`, 0.06523774475832377`}

```

```

In[238]:= Total[ionyi]

```

```

Out[238]= 1.

```

```

In[239]:= tabionyi = Table[{youngexpt2000eV[[i]],
    theoryplain2000eVo064[[i]], ionyinorm[[i]]}, {i, 1, 10}];

In[240]:= BarChart[tabionyi, PlotRange → {-0.05, 0.45},
    ChartLabels → {Placed[{"Ne+", "Ne2+", "Ne3+", "Ne4+", "Ne5+", "Ne6+", "Ne7+", "Ne8+",
        "Ne9+", "Ne10+"}, Below], Placed[{}, Above]}, AxesLabel → {"", "Y"},
    AxesStyle → {{Arrowheads[Automatic], AbsoluteThickness[0.6]},
        {Arrowheads[Automatic], AbsoluteThickness[0.6]}},
    LabelStyle → {FontFamily → "Helvetica", FontSize → 14}]

```

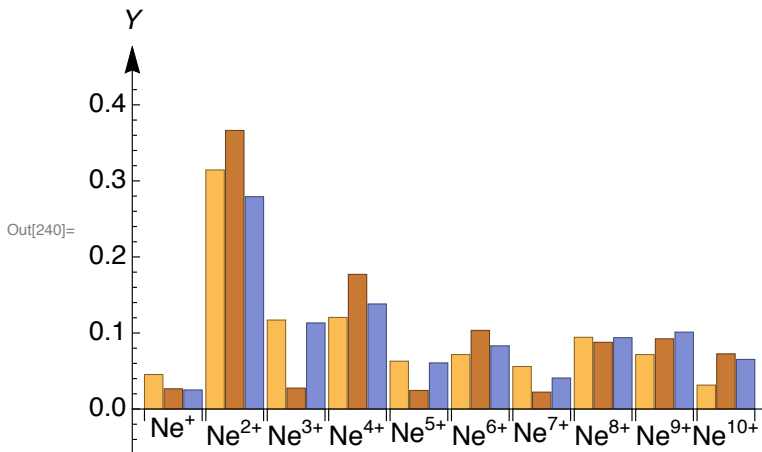

### Adjusted beam area, original damping 0.584 / 3

```

In[241]:= optdamp := 0.584 / 3
pulseenergy := optdamp * 2.4 * MilliJouleToHartree
omegaX := 1999.999 * eVToHartree
tauX := 230 * FemtoSecondTot0
rhoXx := 1 * MicrometerToBohr
rhoYy := rhoXx
X-ray peak intensity:

In[247]:= J0Xfun[pulseenergy, omegaX, tauX, 0, 0] * omegaX * intensityAUtoSI
Out[247]= 1.68414 × 1017

In[248]:= ionyi = ionyildcrateranalysis[pulseenergy, omegaX, tauX, nintdata];
ionyinorm = 1 / Total[ionyi[[2 ;;]]] * ionyi[[2 ;;]]

Out[249]= {0.0300013, 0.333807, 0.134233, 0.159238, 0.0673029,
    0.0862876, 0.038735, 0.0742226, 0.0540034, 0.0221694}

In[66]:= theoryshake2000eVo019beam := {0.030001327141234026`,
    0.33380696490662687`, 0.1342330276176335`, 0.1592378449419349`,
    0.06730286417137968`, 0.0862875930907281`, 0.038735036281640205`,
    0.07422257581135884`, 0.054003380052393704`, 0.02216938598507015`}

In[251]:= Total[ionyi]
Out[251]= 1.

```

```

In[252]:= tabionyi = Table[{youngexpt2000eV[[i]],
    theoryplain2000eVo019beam[[i]], ionyinorm[[i]]}, {i, 1, 10}];

In[253]:= BarChart[tabionyi, PlotRange → {-0.05, 0.45},
    ChartLabels → {Placed[{"Ne+", "Ne2+", "Ne3+", "Ne4+", "Ne5+", "Ne6+", "Ne7+", "Ne8+",
        "Ne9+", "Ne10+"}, Below], Placed[{}, Above]}, AxesLabel → {"", "Y"},
    AxesStyle → {{Arrowheads[Automatic], AbsoluteThickness[0.6]},
        {Arrowheads[Automatic], AbsoluteThickness[0.6]}},
    LabelStyle → {FontFamily → "Helvetica", FontSize → 14}]

```

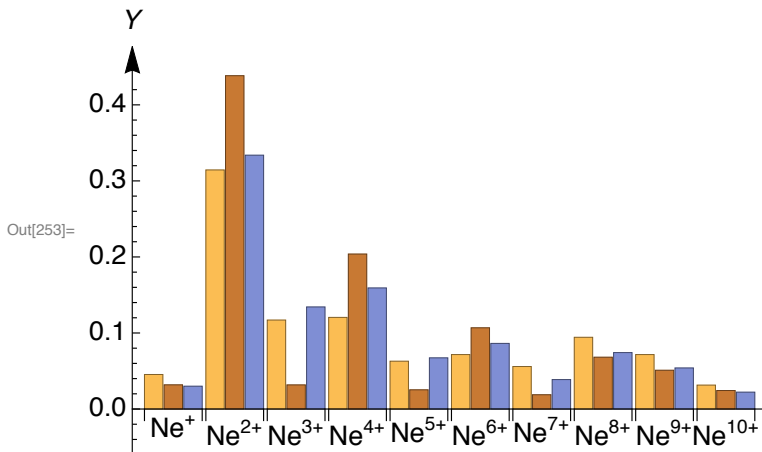

## Adjusted beam area, adjusted damping 0.25

```

In[254]:= optdamp := 0.25
pulseenergy := optdamp * 2.4 * MilliJouleToHartree
omegaX := 1999.999 * eVToHartree
tauX := 230 * FemtoSecondTot0
rhoXx := 1 * MicrometerToBohr
rhoYy := rhoXx
X-ray peak intensity:

```

```

In[260]:= J0Xfun[pulseenergy, omegaX, tauX, 0, 0] * omegaX * intensityAUtoSI
Out[260]= 2.16285 × 1017

```

```

In[261]:= ionyi = ionyieldcrateranalysis[pulseenergy, omegaX, tauX, nintdata];
ionyinorm = 1 / Total[ionyi[[2 ;;]]] * ionyi[[2 ;;]]
Out[262]= {0.027251, 0.303631, 0.122739, 0.148501, 0.0642719,
    0.0859041, 0.0403414, 0.0854474, 0.078413, 0.0434999}

```

```

In[67]:= theoryshake2000eVo025beam := {0.027250991484482966`,
    0.3036308759142831`, 0.12273907980900742`, 0.14850135959510807`,
    0.06427185311558209`, 0.08590410368640856`, 0.040341427697314`,
    0.08544739476445565`, 0.07841297739827753`, 0.043499936535080524` }

```

```

In[264]:= Total[ionyi]
Out[264]= 1.

```

```

In[265]:= tabionyi = Table[{youngexpt2000eV[[i]],
    theoryplain2000eVo025beam[[i]], ionyinorm[[i]]}, {i, 1, 10}];

In[266]:= BarChart[tabionyi, PlotRange → {-0.05, 0.45},
    ChartLabels → {Placed[{"Ne+", "Ne2+", "Ne3+", "Ne4+", "Ne5+", "Ne6+", "Ne7+", "Ne8+",
        "Ne9+", "Ne10+"}, Below], Placed[{}, Above]}, AxesLabel → {"", "Y"},
    AxesStyle → {{Arrowheads[Automatic], AbsoluteThickness[0.6]},
        {Arrowheads[Automatic], AbsoluteThickness[0.6]}},
    LabelStyle → {FontFamily → "Helvetica", FontSize → 14}]

```

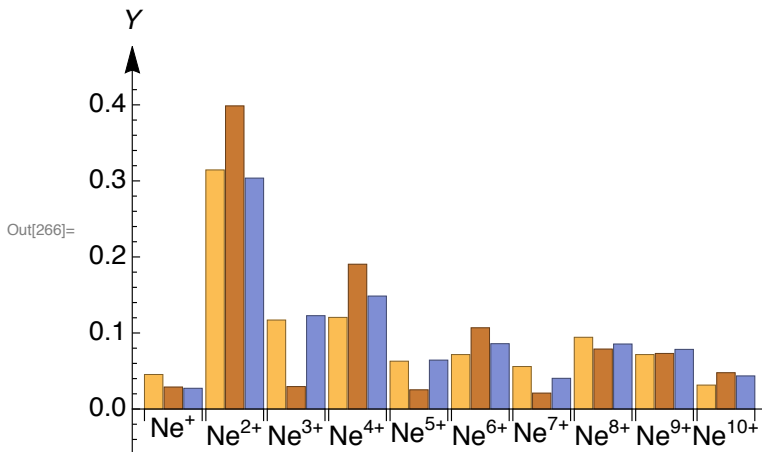

## Actual pulse energy

```

In[652]:= youngexpt800eVpartialionyi =
    youngexpt800eV[[1 ;; 2]] / Total[youngexpt800eV[[1 ;; 2]]];
theoryshake800eVpartialionyi =
    theoryshake800eV[[1 ;; 2]] / Total[theoryshake800eV[[1 ;; 2]]];

```

```

In[670]:= BarChart[
  Table[{youngexpt800eVpartialionyi[[i]], theoryshake800eVpartialionyi[[i]]},
    {i, 1, 2}], PlotRange → {0, 1}, Axes → False,
  LabelStyle → {FontFamily → "Helvetica", FontSize → 14}, ChartLabels →
    {Placed[Table[Style[i, labelcolor], {i, 1, 2}], Below], Placed[{}], Above}},
  ChartStyle → {Black, Red}, BarSpacing → {Small, 3}, Frame → True,
  FrameStyle → Thick, FrameTicks → {{{{0, "0.0"}, 0.1, 0.2, 0.3,
    0.4, 0.5, 0.6, 0.7, 0.8, 0.9, {1, "1.0"}}, False}, {True, False}},
  FrameTicksStyle → {{Thick, Transparent}, {Transparent, Transparent}},
  FrameLabel → {"Charge state  $i$ ", "Ion yield  $Y_i$ "}]

```

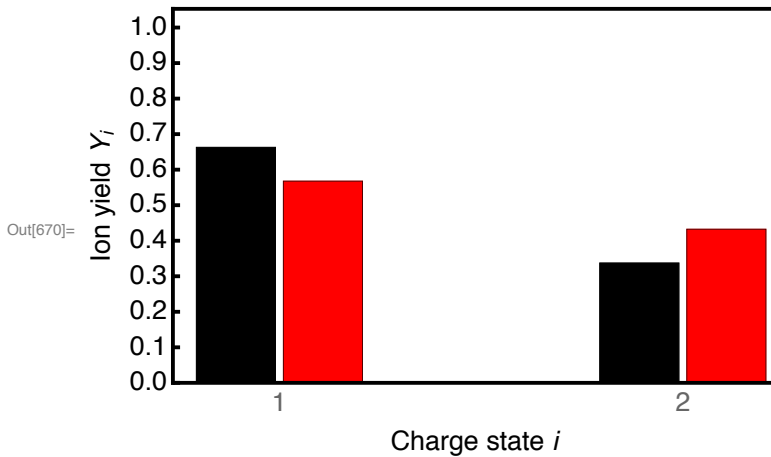

```

In[655]:= youngexpt1050eVpartialionyi =
  youngexpt1050eV[[1 ;; 2]] / Total[youngexpt1050eV[[1 ;; 2]]];
theoryshake1050eVpartialionyi =
  theoryshake1050eV[[1 ;; 2]] / Total[theoryshake1050eV[[1 ;; 2]]];

```

```

In[671]:= BarChart[
  Table[{youngexpt1050eVpartialionyi[[i]], theoryshake1050eVpartialionyi[[i]]},
    {i, 1, 2}], PlotRange → {0, 1}, Axes → False,
  LabelStyle → {FontFamily → "Helvetica", FontSize → 14}, ChartLabels →
    {Placed[Table[Style[i, labelcolor], {i, 1, 2}], Below], Placed[{}], Above}},
  ChartStyle → {Black, Red}, BarSpacing → {Small, 3}, Frame → True,
  FrameStyle → Thick, FrameTicks → {{{{0, "0.0"}, 0.1, 0.2, 0.3,
    0.4, 0.5, 0.6, 0.7, 0.8, 0.9, {1, "1.0"}}, False}, {True, False}},
  FrameTicksStyle → {{Thick, Transparent}, {Transparent, Transparent}},
  FrameLabel → {"Charge state  $i$ ", "Ion yield  $Y_i$ "}]

```

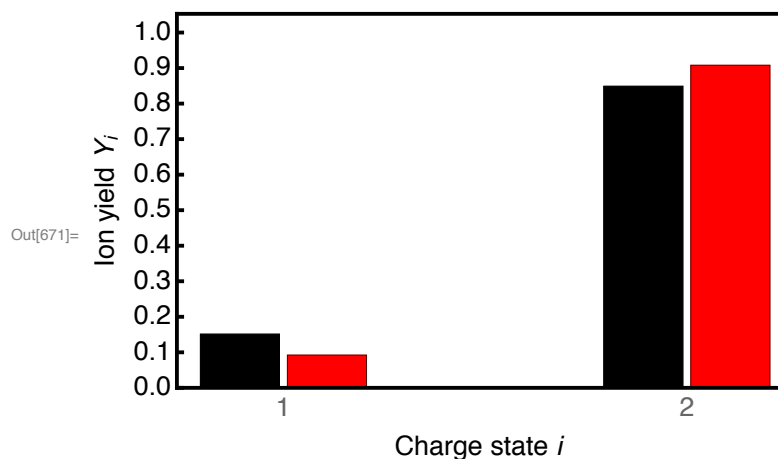

```

In[658]:= youngexpt2000eVpartialionyi =
  youngexpt2000eV[[1 ;; 2]] / Total[youngexpt2000eV[[1 ;; 2]]];
theoryshake2000eVpartialionyi = theoryshake2000eVo025beam[[1 ;; 2]] /
  Total[theoryshake2000eVo025beam[[1 ;; 2]]];

```



```

In[672]:= BarChart[
  Table[{youngexpt2000eVpartialionyi[[i]], theoryshake2000eVpartialionyi[[i]]},
    {i, 1, 2}], PlotRange → {0, 1}, Axes → False,
  LabelStyle → {FontFamily → "Helvetica", FontSize → 14}, ChartLabels →
    {Placed[Table[Style[i, labelcolor], {i, 1, 2}], Below], Placed[{}], Above}},
  ChartStyle → {Black, Red}, BarSpacing → {Small, 3}, Frame → True,
  FrameStyle → Thick, FrameTicks → {{{{0, "0.0"}, 0.1, 0.2, 0.3,
    0.4, 0.5, 0.6, 0.7, 0.8, 0.9, {1, "1.0"}}, False}, {True, False}},
  FrameTicksStyle → {{Thick, Transparent}, {Transparent, Transparent}},
  FrameLabel → {"Charge state  $i$ ", "Ion yield  $Y_i$ "}]

```

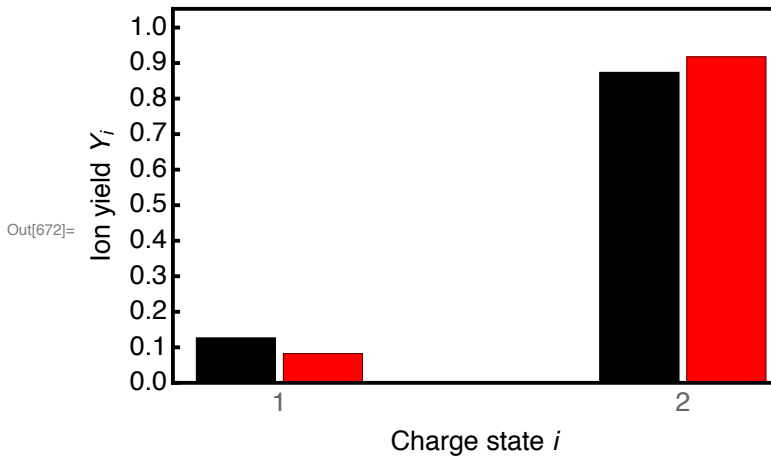

```

In[661]:= doumyexpt1110eVpartialionyi =
  doumyexpt1110eV[[1 ;; 2]] / Total[doumyexpt1110eV[[1 ;; 2]]];
theoryshake1110eVpartialionyi =
  theoryshake1110eV[[1 ;; 2]] / Total[theoryshake1110eV[[1 ;; 2]]];

```

```

In[673]:= BarChart[
  Table[{doumyexpt1110eVpartialionyi[[i]], theoryshake1110eVpartialionyi[[i]]},
    {i, 1, 2}], PlotRange → {0, 1}, Axes → False,
  LabelStyle → {FontFamily → "Helvetica", FontSize → 14}, ChartLabels →
    {Placed[Table[Style[i, labelcolor], {i, 1, 2}], Below], Placed[{}], Above}},
  ChartStyle → {Black, Red}, BarSpacing → {Small, 3}, Frame → True,
  FrameStyle → Thick, FrameTicks → {{{{0, "0.0"}, 0.1, 0.2, 0.3,
    0.4, 0.5, 0.6, 0.7, 0.8, 0.9, {1, "1.0"}}, False}, {True, False}},
  FrameTicksStyle → {{Thick, Transparent}, {Transparent, Transparent}},
  FrameLabel → {"Charge state  $i$ ", "Ion yield  $Y_i$ "}]

```

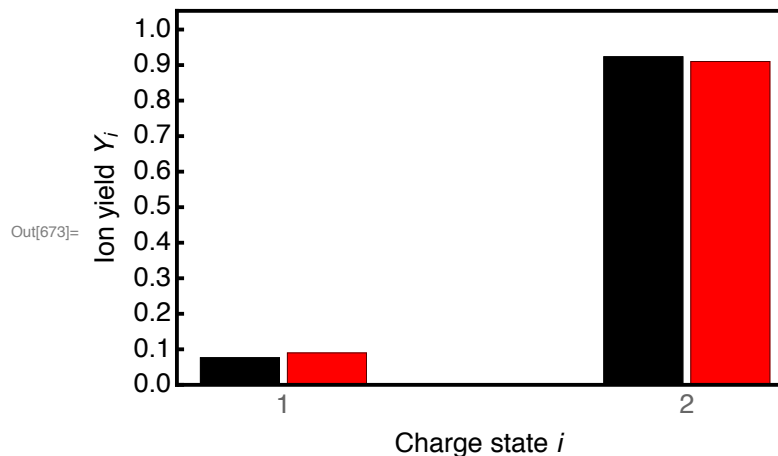

```

In[664]:= doumyexpt1225eVpartialionyi =
  doumyexpt1225eV[[1 ;; 2]] / Total[doumyexpt1225eV[[1 ;; 2]]];
theoryshake1225eVpartialionyi =
  theoryshake1225eV[[1 ;; 2]] / Total[theoryshake1225eV[[1 ;; 2]]];

```

```

In[674]:= BarChart[
  Table[{doumyexpt1225eVpartialionyi[[i]], theoryshake1225eVpartialionyi[[i]]},
    {i, 1, 2}], PlotRange → {0, 1}, Axes → False,
  LabelStyle → {FontFamily → "Helvetica", FontSize → 14}, ChartLabels →
    {Placed[Table[Style[i, labelcolor], {i, 1, 2}], Below], Placed[{}], Above}},
  ChartStyle → {Black, Red}, BarSpacing → {Small, 3}, Frame → True,
  FrameStyle → Thick, FrameTicks → {{{{0, "0.0"}, 0.1, 0.2, 0.3,
    0.4, 0.5, 0.6, 0.7, 0.8, 0.9, {1, "1.0"}}, False}, {True, False}},
  FrameTicksStyle → {{Thick, Transparent}, {Transparent, Transparent}},
  FrameLabel → {"Charge state i", "Ion yield  $Y_i$ "}]

```

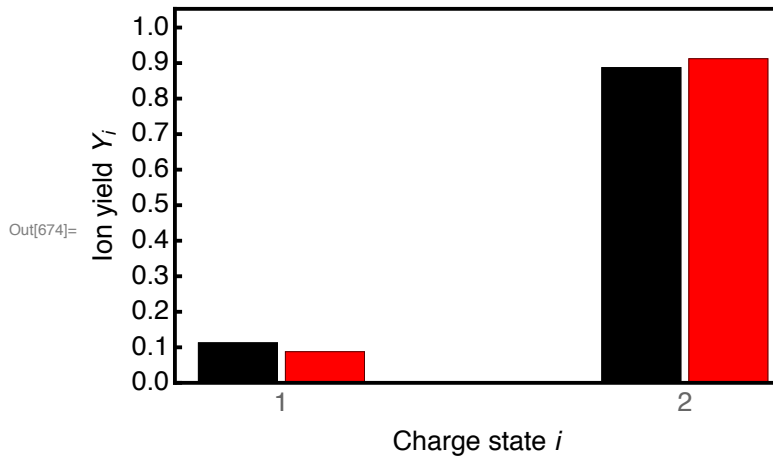

## Ion yields with shake off

```

In[97]:= da223v126 := 0
da214v126 := 0
da205v126 := 0
daTot126 := 0

```

### Young data 2000 eV

#### Original damping 0.584 / 3

```

In[101]:= optdamp := 0.584 / 3
pulseenergy := optdamp * 2.4 * MilliJouleToHartree
omegaX := 1999.999 * eVToHartree
tauX := 230 * FemtoSecondTot0
rhoXx := 1 * MicrometerToBohr
rhoYy := 2 * MicrometerToBohr

X-ray peak intensity:

In[107]:= J0Xfun[pulseenergy, omegaX, tauX, 0, 0] * omegaX * intensityAUtoSI
Out[107]= 8.4207 × 1016

```

```

In[108]:= ionyi = ionyielddcrateranalysis[pulseenergy, omegaX, tauX, nintdata];
ionyinorm = 1/Total[ionyi[[2 ;;]]] * ionyi[[2 ;;]]

Out[109]= {0.0398482, 0.464566, 0.139782, 0.175448, 0.0531974,
0.0645271, 0.0202524, 0.0294837, 0.0108582, 0.00203718}

In[110]:= Total[ionyi]

Out[110]= 1.

In[111]:= tabionyi = Table[{theoryshake2000eVo019[[i]], ionyinorm[[i]]}, {i, 1, 10}];

In[112]:= BarChart[tabionyi, PlotRange → {-0.05, 0.45},
ChartLabels → {Placed[{"Ne+", "Ne2+", "Ne3+", "Ne4+", "Ne5+", "Ne6+", "Ne7+", "Ne8+",
"Ne9+", "Ne10+"}, Below], Placed[{}, Above]}, AxesLabel → {"", "Y"},
AxesStyle → {{Arrowheads[Automatic], AbsoluteThickness[0.6]},
{Arrowheads[Automatic], AbsoluteThickness[0.6]}},
LabelStyle → {FontFamily → "Helvetica", FontSize → 14}]

```

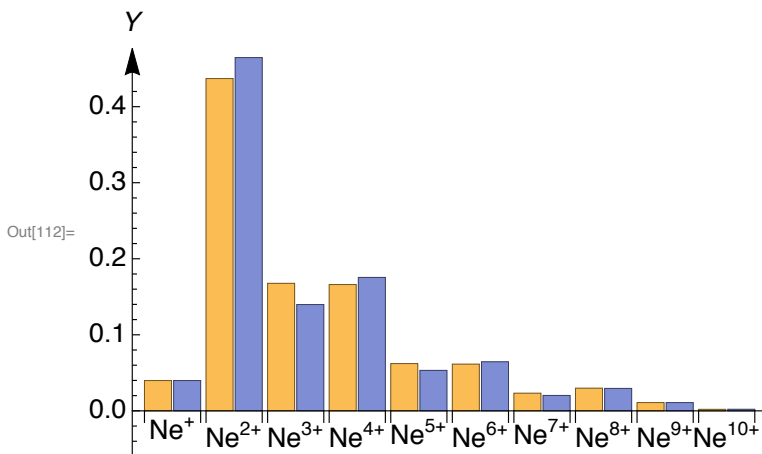

### Adjusted damping 0.635, adjusted pulse duration 140 fs

```

In[113]:= optdamp := 0.635
pulseenergy := optdamp * 2.4 * MilliJouleToHartree
omegaX := 1999.999 * eVToHartree
tauX := 140 * FemtoSecondTot0
rhoXx := 1 * MicrometerToBohr
rhoYy := 2 * MicrometerToBohr
X-ray peak intensity:

In[119]:= J0Xfun[pulseenergy, omegaX, tauX, 0, 0] * omegaX * intensityAUtoSI

Out[119]= 4.51264 × 1017

In[120]:= ionyi = ionyielddcrateranalysis[pulseenergy, omegaX, tauX, nintdata];
ionyinorm = 1/Total[ionyi[[2 ;;]]] * ionyi[[2 ;;]]

Out[121]= {0.0250299, 0.296814, 0.0952887, 0.145824, 0.0532783,
0.0871153, 0.0370876, 0.0928984, 0.0996632, 0.0670003}

```

```
In[122]:= Total[ionyi]
```

```
Out[122]= 1.
```

```
In[123]:= tabionyi = Table[{theoryshake2000eVo064[[i]], ionyinorm[[i]]}, {i, 1, 10}];
```

```
In[124]:= BarChart[tabionyi, PlotRange → {-0.05, 0.45},
  ChartLabels → {Placed[{"Ne+", "Ne2+", "Ne3+", "Ne4+", "Ne5+", "Ne6+", "Ne7+", "Ne8+",
    "Ne9+", "Ne10+"}, Below], Placed[{}, Above]}, AxesLabel → {"", "Y"},
  AxesStyle → {{Arrowheads[Automatic], AbsoluteThickness[0.6]},
    {Arrowheads[Automatic], AbsoluteThickness[0.6]}},
  LabelStyle → {FontFamily → "Helvetica", FontSize → 14}]
```

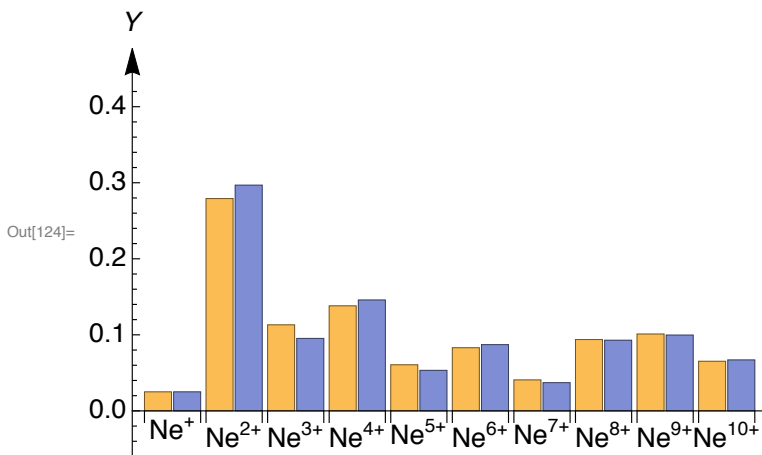

### Adjusted beam area, original damping 0.584 / 3

```
In[125]:= optdamp := 0.584 / 3
```

```
pulseenergy := optdamp * 2.4 * MilliJouleToHartree
```

```
omegaX := 1999.999 * eVToHartree
```

```
tauX := 230 * FemtoSecondTot0
```

```
rhoXx := 1 * MicrometerToBohr
```

```
rhoYy := rhoXx
```

X-ray peak intensity:

```
In[131]:= J0Xfun[pulseenergy, omegaX, tauX, 0, 0] * omegaX * intensityAUtoSI
```

```
Out[131]= 1.68414 × 1017
```

```
In[132]:= ionyi = ionyildcrateranalysis[pulseenergy, omegaX, tauX, nintdata];
```

```
ionyinorm = 1 / Total[ionyi[[2 ;;]]] * ionyi[[2 ;;]]
```

```
Out[133]= {0.0300013, 0.354878, 0.112868, 0.16817, 0.0587868,
  0.0905898, 0.034831, 0.0734115, 0.0536927, 0.0227715}
```

```
In[134]:= Total[ionyi]
```

```
Out[134]= 1.
```

```
In[135]:= tabionyi = Table[{theoryshake2000eVo019beam[[i]], ionyinorm[[i]]}, {i, 1, 10}];
```

```
In[136]:= BarChart[tablyoni, PlotRange → {-0.05, 0.45},
  ChartLabels → {Placed[{"Ne+", "Ne2+", "Ne3+", "Ne4+", "Ne5+", "Ne6+", "Ne7+", "Ne8+",
    "Ne9+", "Ne10+"}, Below], Placed[{}, Above]}, AxesLabel → {"", "Y"},
  AxesStyle → {{Arrowheads[Automatic], AbsoluteThickness[0.6]},
    {Arrowheads[Automatic], AbsoluteThickness[0.6]}},
  LabelStyle → {FontFamily → "Helvetica", FontSize → 14}]
```

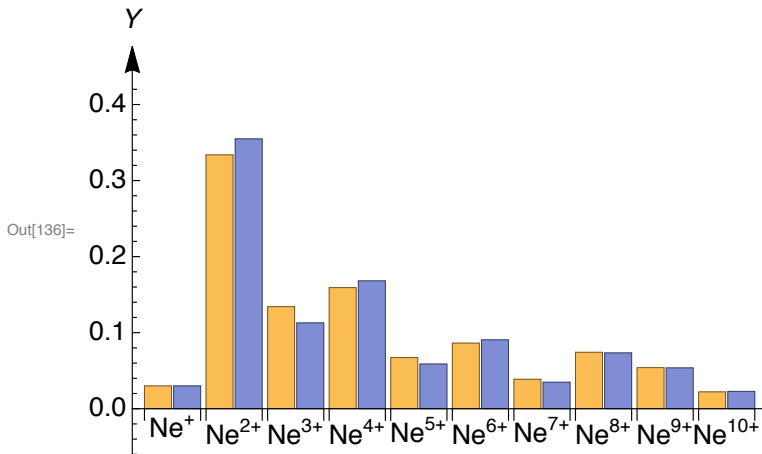

### Adjusted beam area, adjusted damping 0.25

```
In[137]:= optdamp := 0.25
pulseenergy := optdamp * 2.4 * MilliJouleToHartree
omegaX := 1999.999 * eVToHartree
tauX := 230 * FemtoSecondTot0
rhoXx := 1 * MicrometerToBohr
rhoYy := rhoXx
X-ray peak intensity:

In[143]:= J0Xfun[pulseenergy, omegaX, tauX, 0, 0] * omegaX * intensityAtoSI
```

Out[143]=  $2.16285 \times 10^{17}$

```
In[144]:= ionyi = ionyieldcrateranalysis[pulseenergy, omegaX, tauX, nintdata];
ionyinorm = 1 / Total[ionyi[[2 ;;]]] * ionyi[[2 ;;]]
```

Out[145]= {0.027251, 0.322796, 0.103301, 0.156824, 0.0563435,  
0.0901757, 0.0365213, 0.0844922, 0.0776766, 0.0446184}

```
In[146]:= Total[ionyi]
```

Out[146]= 1.

```
In[147]:= tabiony = Table[{theoryshake2000eVo025beam[[i]], ionyinorm[[i]]}, {i, 1, 10}];
```

```
In[148]:= BarChart[tabionyi, PlotRange → {-0.05, 0.45},
  ChartLabels → {Placed[{"Ne+", "Ne2+", "Ne3+", "Ne4+", "Ne5+", "Ne6+", "Ne7+", "Ne8+",
    "Ne9+", "Ne10+"}, Below], Placed[{}, Above]}, AxesLabel → {"", "Y"},
  AxesStyle → {{Arrowheads[Automatic], AbsoluteThickness[0.6]},
    {Arrowheads[Automatic], AbsoluteThickness[0.6]}},
  LabelStyle → {FontFamily → "Helvetica", FontSize → 14}]
```

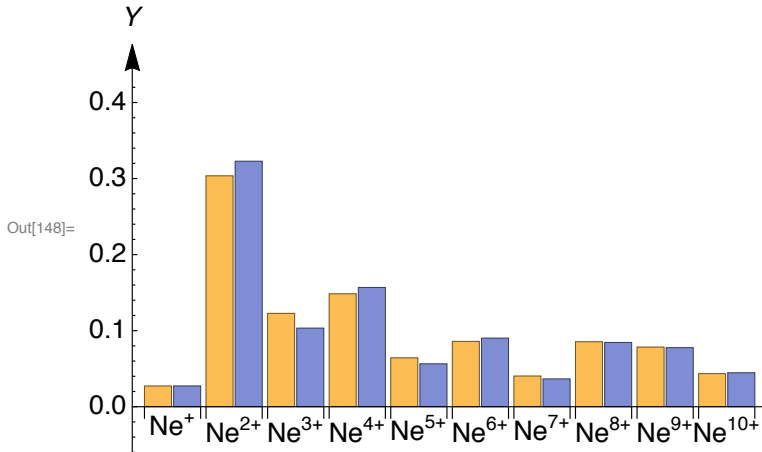

## Restore double Auger decay

```
In[149]:= da223v126 := p2pm3 / pNem3 * d
da214v126 := p2sm12pm2 / pNem3 * d
da205v126 := p2sm22pm1 / pNem3 * d
daTot126 := da223v126 + da214v126 + da205v126
```

## Ion yields with Bhalla's Auger decay widths

Doumy data 1225 eV:

Young data 1050 eV damping:  $0.699 / 3 = 0.233$

```
In[338]:= optdamp := 0.699 / 3
pulseenergy := optdamp * 1.45 * MilliJouleToHartree
omegaX := 1225 * eVToHartree
tauX := 100 * FemtoSecondTot0
rhoXx := 1 * MicrometerToBohr
rhoYy := 2 * MicrometerToBohr

In[344]:= ionyiref = ionyildcrateranalysis[pulseenergy, omegaX, tauX, nintdata];
ionyinormref = 1 / Total[ionyiref[[2 ;;]]] * ionyiref[[2 ;;]]

Out[345]= {0.0244456, 0.254286, 0.104633, 0.126883, 0.0576132,
  0.0790318, 0.0424713, 0.176186, 0.134449, 4.75453 × 10-7}
```

## Bhalla's data

### Total width of single core holes

```
In[346]:= bhGA126 := 88.066*^-4
          bhGA125 := 78.753*^-4
          bhGA124 := 66.278*^-4
          bhGA123 := 51.633*^-4
          bhGA122 := 36.687*^-4
          bhGA121 := 23.994*^-4
```

```
          bhGA116 := 80.428*^-4
          bhGA115 := 67.321*^-4
          bhGA114 := 51.162*^-4
          bhGA113 := 33.624*^-4
          bhGA112 := 17.113*^-4
          bhGA111 := 4.716*^-4
```

```
          bhGA106 := 77.901*^-4
          bhGA105 := 61.854*^-4
          bhGA104 := 43.571*^-4
          bhGA103 := 25.306*^-4
          bhGA102 := 9.682*^-4
```

```
In[363]:= GamATot126 := bhGA126
          GamATot125 := bhGA125
          GamATot124 := bhGA124
          GamATot123 := bhGA123
          GamATot122 := bhGA122
          GamATot121 := bhGA121
          GamATot116 := bhGA116
          GamATot115 := bhGA115
          GamATot114 := bhGA114
          GamATot113 := bhGA113
          GamATot112 := bhGA112
          GamATot111 := bhGA111
          GamATot106 := bhGA106
          GamATot105 := bhGA105
          GamATot104 := bhGA104
          GamATot103 := bhGA103
          GamATot102 := bhGA102
```



## 2p–2p decay of single core holes

```
In[380]:= bhGA224v126 := 55.284*^-4
          bhGA223v125 := 45.358*^-4
          bhGA222v124 := 33.070*^-4
          bhGA221v123 := 19.731*^-4
          bhGA220v122 := 7.698*^-4
```

```
          bhGA214v116 := 66.278*^-4
          bhGA213v115 := 53.548*^-4
          bhGA212v114 := 38.330*^-4
          bhGA211v113 := 22.495*^-4
          bhGA210v112 := 8.670*^-4
```

```
          bhGA204v106 := 77.901*^-4
          bhGA203v105 := 61.854*^-4
          bhGA202v104 := 43.571*^-4
          bhG201v103 := 25.306*^-4
          bhGA200v102 := 9.682*^-4
```

```
In[395]:= GamA224v126 := bhGA224v126
          GamA223v125 := bhGA223v125
          GamA222v124 := bhGA222v124
          GamA221v123 := bhGA221v123
          GamA220v122 := bhGA220v122
          GamA214v116 := bhGA214v116
          GamA213v115 := bhGA213v115
          GamA212v114 := bhGA212v114
          GamA211v113 := bhGA211v113
          GamA210v112 := bhGA210v112
          GamA204v106 := bhGA204v106
          GamA203v105 := bhGA203v105
          GamA202v104 := bhGA202v104
          GamA201v103 := bhG201v103
          GamA200v102 := bhGA200v102
```

## 2s–2p decay of single core holes

```
In[410]:= bhGA215v126 := 24.448*^-4
          bhGA214v125 := 24.002*^-4
          bhGA213v124 := 22.507*^-4
          bhGA212v123 := 19.682*^-4
          bhGA211v122 := 15.163*^-4
          bhGA210v121 := 8.606*^-4
```

```
          bhGA205v116 := 14.150*^-4
          bhGA204v115 := 13.773*^-4
          bhGA203v114 := 12.832*^-4
          bhGA202v113 := 11.129*^-4
          bhGA201v112 := 8.442*^-4
          bhGA200v111 := 4.716*^-4
```

```
In[422]:= GamA215v126 := bhGA215v126
          GamA214v125 := bhGA214v125
          GamA213v124 := bhGA213v124
          GamA212v123 := bhGA212v123
          GamA211v122 := bhGA211v122
          GamA210v121 := bhGA210v121
          GamA205v116 := bhGA205v116
          GamA204v115 := bhGA204v115
          GamA203v114 := bhGA203v114
          GamA202v113 := bhGA202v113
          GamA201v112 := bhGA201v112
          GamA200v111 := bhGA200v111
```

## 2s–2s decay of single core holes

```
In[434]:= bhGA206v126 := 8.334*^-4
          bhGA205v125 := 9.393*^-4
          bhGA204v124 := 10.701*^-4
          bhGA203v123 := 12.220*^-4
          bhGA202v122 := 13.827*^-4
          bhGA201v121 := 15.388*^-4
```

```
In[440]:= GamA206v126 := bhGA206v126
          GamA205v125 := bhGA205v125
          GamA204v124 := bhGA204v124
          GamA203v123 := bhGA203v123
          GamA202v122 := bhGA202v122
          GamA201v121 := bhGA201v121
```

## Total width of double core holes

```
In[446]:= bhGA026 := 129.860 * 2*^-4
          bhGA025 := 112.160 * 2*^-4
          bhGA024 := 91.009 * 2*^-4
          bhGA023 := 68.309 * 2*^-4
          bhGA022 := 46.790 * 2*^-4
          bhGA021 := 29.702 * 2*^-4
```

```
          bhGA016 := 119.128 * 2*^-4
          bhGA015 := 96.478 * 2*^-4
          bhGA014 := 70.982 * 2*^-4
          bhGA013 := 45.172 * 2*^-4
          bhGA012 := 22.201 * 2*^-4
          bhGA011 := 5.872 * 2*^-4
```

```
          bhGA006 := 116.220 * 2*^-4
          bhGA005 := 89.805 * 2*^-4
          bhGA004 := 61.849 * 2*^-4
          bhGA003 := 35.184 * 2*^-4
          bhGA002 := 13.161 * 2*^-4
```

```
In[463]:= GamATot026 := bhGA026
          GamATot025 := bhGA025
          GamATot024 := bhGA024
          GamATot023 := bhGA023
          GamATot022 := bhGA022
          GamATot021 := bhGA021
          GamATot016 := bhGA016
          GamATot015 := bhGA015
          GamATot014 := bhGA014
          GamATot013 := bhGA013
          GamATot012 := bhGA012
          GamATot011 := bhGA011
          GamATot006 := bhGA006
          GamATot005 := bhGA005
          GamATot004 := bhGA004
          GamATot003 := bhGA003
          GamATot002 := bhGA002
```

## 2p–2p decay of double core holes

```

In[480]:= bhGA124v026 := 85.925 * 2*^-4
          bhGA123v025 := 67.900 * 2*^-4
          bhGA122v024 := 47.598 * 2*^-4
          bhGA121v023 := 27.310 * 2*^-4
          bhGA120v022 := 10.233 * 2*^-4

          bhGA114v016 := 99.936 * 2*^-4
          bhGA113v015 := 78.032 * 2*^-4
          bhGA112v014 := 54.054 * 2*^-4
          bhGA111v013 := 30.757 * 2*^-4
          bhGA110v012 := 11.475 * 2*^-4

          bhGA104v006 := 116.220 * 2*^-4
          bhGA103v005 := 89.805 * 2*^-4
          bhGA102v004 := 61.849 * 2*^-4
          bhGA101v003 := 35.184 * 2*^-4
          bhGA100v002 := 13.161 * 2*^-4

In[495]:= GamA124v026 := bhGA124v026
          GamA123v025 := bhGA123v025
          GamA122v024 := bhGA122v024
          GamA121v023 := bhGA121v023
          GamA120v022 := bhGA120v022
          GamA114v016 := bhGA114v016
          GamA113v015 := bhGA113v015
          GamA112v014 := bhGA112v014
          GamA111v013 := bhGA111v013
          GamA110v012 := bhGA110v012
          GamA104v006 := bhGA104v006
          GamA103v005 := bhGA103v005
          GamA102v004 := bhGA102v004
          GamA101v003 := bhGA101v003
          GamA100v002 := bhGA100v002

```

## 2s–2p decay of double core holes

```
In[510]:= bhGA115v026 := 33.699 * 2*^-4
          bhGA114v025 := 32.558 * 2*^-4
          bhGA113v024 := 30.020 * 2*^-4
          bhGA112v023 := 25.753 * 2*^-4
          bhGA111v022 := 19.398 * 2*^-4
          bhGA110v021 := 10.772 * 2*^-4
```

```
          bhGA105v016 := 19.192 * 2*^-4
          bhGA104v015 := 18.446 * 2*^-4
          bhGA103v014 := 16.928 * 2*^-4
          bhGA102v013 := 14.415 * 2*^-4
          bhGA101v012 := 10.726 * 2*^-4
          bhGA100v011 := 5.872 * 2*^-4
```

```
In[522]:= GamA115v026 := bhGA115v026
          GamA114v025 := bhGA114v025
          GamA113v024 := bhGA113v024
          GamA112v023 := bhGA112v023
          GamA111v022 := bhGA111v022
          GamA110v021 := bhGA110v021
          GamA105v016 := bhGA105v016
          GamA104v015 := bhGA104v015
          GamA103v014 := bhGA103v014
          GamA102v013 := bhGA102v013
          GamA101v012 := bhGA101v012
          GamA100v011 := bhGA100v011
```

## 2s–2s decay of double core holes

```
In[534]:= bhGA106v026 := 10.239 * 2*^-4
          bhGA105v025 := 11.698 * 2*^-4
          bhGA104v024 := 13.390 * 2*^-4
          bhGA103v023 := 15.246 * 2*^-4
          bhGA102v022 := 17.160 * 2*^-4
          bhGA101v021 := 18.930 * 2*^-4
```

```
In[540]:= GamA106v026 := bhGA106v026
          GamA105v025 := bhGA105v025
          GamA104v024 := bhGA104v024
          GamA103v023 := bhGA103v023
          GamA102v022 := bhGA102v022
          GamA101v021 := bhGA101v021
```

## Ion yields with Bahalla's data

```
In[546]:= ionyi = ionyieldcrateranalysis[pulseenergy, omegaX, tauX, nintdata];
ionyinorm = 1/Total[ionyi[[2 ;;]]] * ionyi[[2 ;;]]
```

```
Out[547]:= {0.0250948, 0.254464, 0.105239, 0.126373, 0.0580922,
0.0787777, 0.0445779, 0.181892, 0.12549, 6.50347 × 10-7}
```

```
In[548]:= BarChart[Partition[Riffle[ionyinormref, ionyinorm], 2], PlotRange → All,
ChartLabels → {Placed[{"Ne+", "Ne2+", "Ne3+", "Ne4+", "Ne5+", "Ne6+", "Ne7+", "Ne8+",
"Ne9+", "Ne10+"}, Below], Placed[{}, Above]}, AxesLabel → {"", "Y(ω)"},
AxesStyle → {{Arrowheads[Automatic], AbsoluteThickness[0.6]},
{Arrowheads[Automatic], AbsoluteThickness[0.6]}},
LabelStyle → {FontFamily → "Helvetica"}]
```

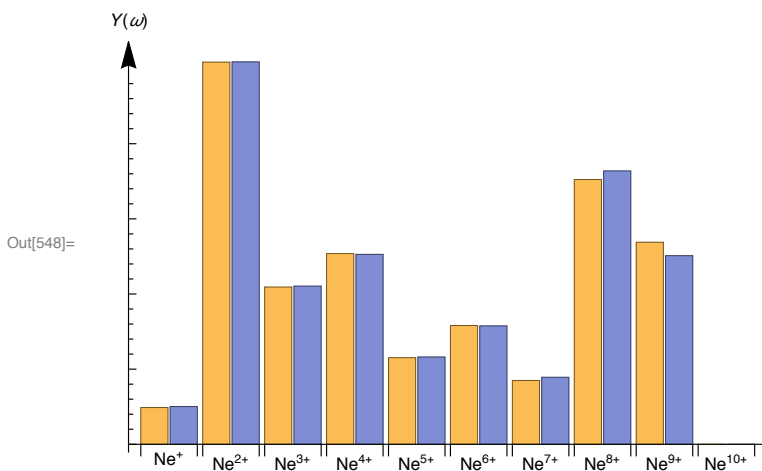

```
In[549]:= ionyinormref - ionyinorm
```

```
Out[549]:= {-0.000649237, -0.000177704, -0.000606043, 0.000510575, -0.000478918,
0.000254754, -0.00210658, -0.00570617, 0.0089595, -1.74895 × 10-7}
```

```
In[550]:= BarChart[(ionyinormref - ionyinorm) * 100, PlotRange -> All,
  ChartLabels -> {"Ne+", "Ne2+", "Ne3+", "Ne4+", "Ne5+", "Ne6+",
    "Ne7+", "Ne8+", "Ne9+", "Ne10+"}, AxesLabel -> {"", "Y( $\omega$ )"},
  AxesStyle -> {{Arrowheads[Automatic], AbsoluteThickness[0.6]},
    {Arrowheads[Automatic], AbsoluteThickness[0.6]}},
  LabelStyle -> {FontFamily -> "Helvetica"}]
```

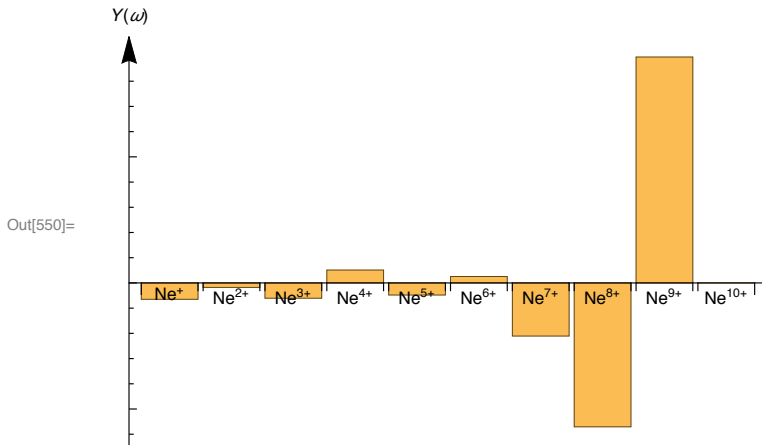

```
In[551]:= BarChart[(ionyinormref - ionyinorm) / ionyinormref * 100,
  PlotRange -> All, ChartLabels -> {"Ne+", "Ne2+", "Ne3+", "Ne4+", "Ne5+",
    "Ne6+", "Ne7+", "Ne8+", "Ne9+", "Ne10+"}, AxesLabel -> {"", "Y( $\omega$ )"},
  AxesStyle -> {{Arrowheads[Automatic], AbsoluteThickness[0.6]},
    {Arrowheads[Automatic], AbsoluteThickness[0.6]}},
  LabelStyle -> {FontFamily -> "Helvetica"}]
```

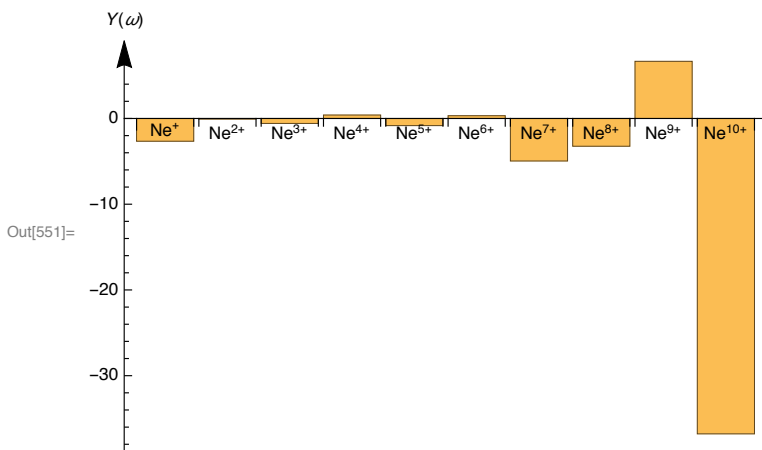

## Presentation graphics

```
In[68]:= lightred := Lighter[Red, 0.7]
green := Darker[Green, 0.5]
lightgreen := Lighter[green, 0.7]
labelcolor := RGBColor[102/255, 102/255, 102/255]
```

```
In[642]:= ColorConvert[Black, "RGB"] // InputForm
```

```
Out[642]//InputForm=
```

```
RGBColor[0., 0., 0.]
```

```
In[643]:= ColorConvert[Red, "RGB"] // InputForm
```

```
Out[643]//InputForm=
```

```
RGBColor[1., 0., 0.]
```

```
In[644]:= ColorConvert[lightred, "RGB"] // InputForm
```

```
Out[644]//InputForm=
```

```
RGBColor[1., 0.7, 0.7]
```

```
In[645]:= ColorConvert[green, "RGB"] // InputForm
```

```
Out[645]//InputForm=
```

```
RGBColor[0., 0.5, 0.]
```

```
In[646]:= ColorConvert[lightgreen, "RGB"] // InputForm
```

```
Out[646]//InputForm=
```

```
RGBColor[0.7, 0.85, 0.7]
```

```
In[647]:= BarChart[
```

```
Table[{youngexpt800eV[[i]], youngtheory800eV[[i]], theoryplain800eV[[i]],
  theoryshake800eV[[i]]}, {i, 1, 10}], PlotRange → {0, 0.5},
Axes → False, LabelStyle → {FontFamily → "Helvetica", FontSize → 14},
ChartStyle → {Black, lightred, Red, green},
BarSpacing → {Small, 3}, Frame → True, FrameStyle → Thick,
FrameTicks → {{{{0, "0.0"}, 0.1, 0.2, 0.3, 0.4, 0.5}, False}, {True, False}},
FrameTicksStyle → {{Thick, Transparent}, {Transparent, Transparent}},
FrameLabel → {None, ""}]
```

```
Out[647]=
```

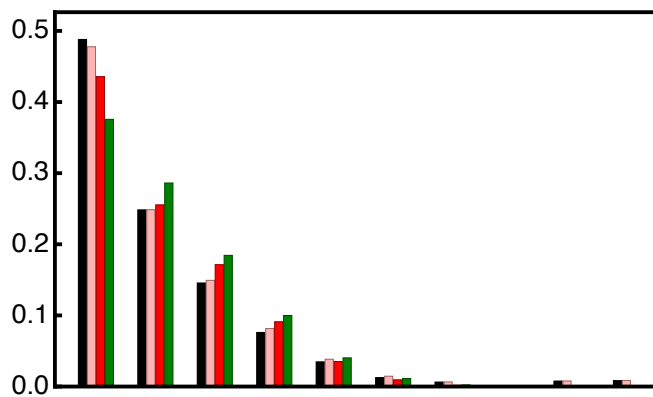



```

In[648]:= BarChart[
  Table[{youngexpt1050eV[[i]], youngtheory1050eV[[i]], theoryplain1050eV[[i]],
    theoryshake1050eV[[i]]}, {i, 1, 10}], PlotRange → {0, 0.5},
  Axes → False, LabelStyle → {FontFamily → "Helvetica", FontSize → 14},
  ChartStyle → {Black, lightred, Red, green},
  BarSpacing → {Small, 3}, Frame → True, FrameStyle → Thick,
  FrameTicks → {{{{0, "0.0"}, 0.1, 0.2, 0.3, 0.4, 0.5}, False}, {True, False}},
  FrameTicksStyle → {{Thick, Transparent}, {Transparent, Transparent}},
  FrameLabel → {None, "Ion yield  $Y_i$ "}

```

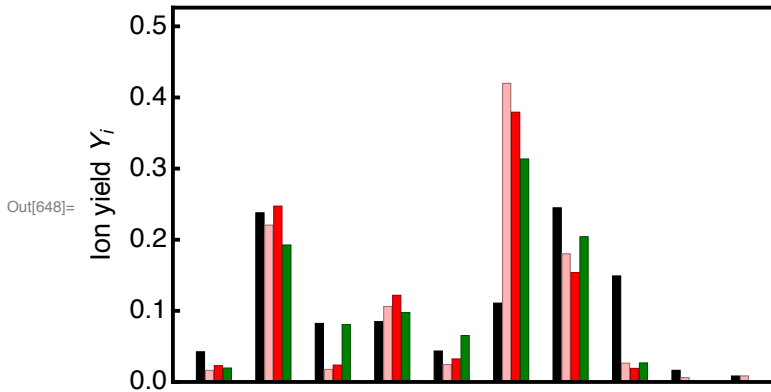

```

In[649]:= BarChart[Table[{youngexpt2000eV[[i]], youngtheory2000eV[[i]],
  theoryplain2000eVo025beam[[i]], theoryshake2000eVo025beam[[i]]},
  {i, 1, 10}], PlotRange → {0, 0.5}, Axes → False,
  LabelStyle → {FontFamily → "Helvetica", FontSize → 14}, ChartLabels →
  {Placed[Table[Style[i, labelcolor], {i, 1, 10}], Below], Placed[{}, Above]},
  ChartStyle → {Black, lightred, Red, green}, BarSpacing → {Small, 3},
  Frame → True, FrameStyle → Thick,
  FrameTicks → {{{{0, "0.0"}, 0.1, 0.2, 0.3, 0.4, 0.5}, False}, {True, False}},
  FrameTicksStyle → {{Thick, Transparent}, {Transparent, Transparent}},
  FrameLabel → {"Charge state  $i$ ", ""}]

```

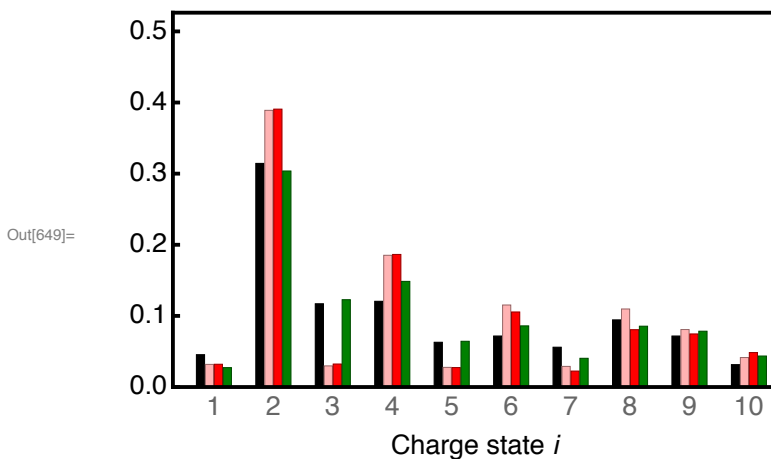

```

In[650]:= BarChart[Table[{doumyexpt1110eV[[i]], doumytheoryplain1110eV[[i]],
  theoryplain1110eV[[i]], doumytheoryshake1110eV[[i]], theoryshake1110eV[[i]]},
  {i, 1, 10}], PlotRange → {0, 0.35}, Axes → False,
LabelStyle → {FontFamily → "Helvetica", FontSize → 14},
ChartStyle → {Black, lightred, Red, lightgreen, green},
BarSpacing → {Small, 3}, Frame → True, FrameStyle → Thick,
FrameTicks → {{{{0, "0.0"}, 0.1, 0.2, 0.3}, False}, {True, False}},
FrameTicksStyle → {{Thick, Transparent}, {Transparent, Transparent}},
FrameLabel → {None, "Ion yield  $Y_i$ "}]

```

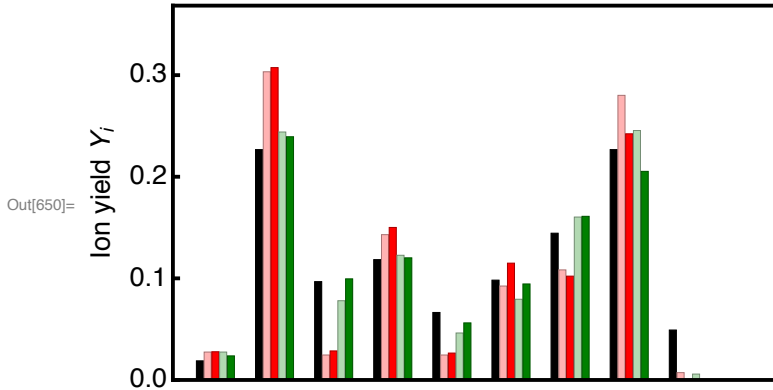

```

In[651]:= BarChart[Table[{doumyexpt1225eV[[i]], doumytheoryplain1225eV[[i]],
  theoryplain1225eV[[i]], doumytheoryshake1225eV[[i]], theoryshake1225eV[[i]]},
  {i, 1, 10}], PlotRange → {0, 0.35}, Axes → False,
LabelStyle → {FontFamily → "Helvetica", FontSize → 14}, ChartLabels →
  {Placed[Table[Style[i, labelcolor], {i, 1, 10}], Below], Placed[{}, Above]},
ChartStyle → {Black, lightred, Red, lightgreen, green},
BarSpacing → {Small, 3}, Frame → True, FrameStyle → Thick,
FrameTicks → {{{{0, "0.0"}, 0.1, 0.2, 0.3}, False}, {True, False}},
FrameTicksStyle → {{Thick, Transparent}, {Transparent, Transparent}},
FrameLabel → {"Charge state  $i$ ", "Ion yield  $Y_i$ "}]

```

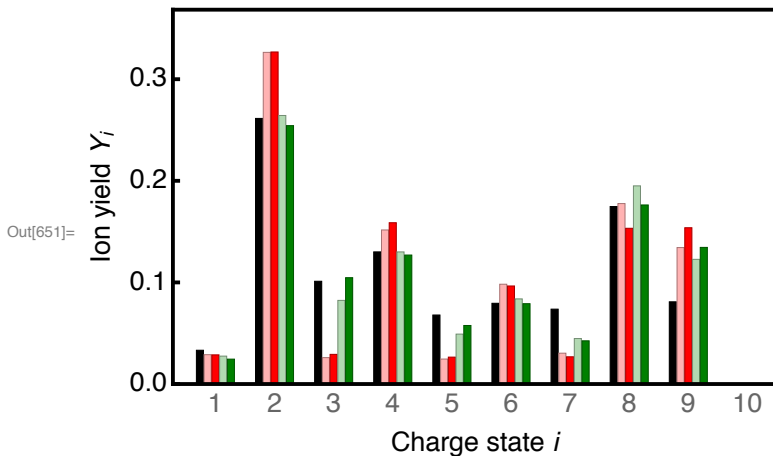

## References

- [1] Christian Buth, Ji-Cai Liu, Mau Hsiung Chen, James P. Cryan, Li Fang, James M. Glownia,

- Matthias Hoener, Ryan N. Coffee, Nora Berrah, *Ultrafast absorption of intense x rays by nitrogen molecules*, J. Chem. Phys. **136**, 214310 (2012), <http://dx.doi.org/10.1063/1.4722756>.
- [2] Y. Hikosaka, T. Kaneyasu, P. Lablanquie, F. Penent, E. Shigemasa, K. Ito, *Multiple Auger decay of the neon 1s-core-hole state studied by multielectron coincidence spectroscopy*, Phys. Rev. A **92**, 033413 (2015), <http://dx.doi.org/10.1103/PhysRevA.92.033413>.
- [3] N. Saito, I. H. Suzuki, *Shake-off processes in photoionization and Auger transition for rare gases irradiated by soft X-rays*, Phys. Scr. **49**, 80–85 (1994), <http://dx.doi.org/10.1088/0031-8949/49/1/011>.
- [4] G. Doumy, C. Roedig, S.-K. Son, C. I. Blaga, A. D. DiChiara, R. Santra, N. Berrah, C. Bostedt, J. D. Bozek, P. H. Bucksbaum, J. P. Cryan, L. Fang, S. Ghimire, J. M. Glowia, M. Hoener, E. P. Kanter, B. Krässig, M. Kuebel, M. Messerschmidt, G. G. Paulus, D. A. Reis, N. Rohringer, L. Young, P. Agostini, L. F. DiMauro, *Nonlinear atomic response to intense ultrashort x rays*, Phys. Rev. Lett. **106**, 83002 (2011), <http://dx.doi.org/10.1103/PhysRevLett.106.083002>.
- [5] L. Young, E.P. Kanter, B. Krässig, Y. Li, A.M. March, S.T. Pratt, R. Santra, S.H. Southworth, N. Rohringer, L.F. DiMauro, G. Doumy, C.A. Roedig, N. Berrah, L. Fang, M. Hoener, P.H. Bucksbaum, J.P. Cryan, S. Ghimire, J.M. Glowia, D.A. Reis, J.D. Bozek, C. Bostedt, M. Messerschmidt, *Femtosecond electronic response of atoms to ultra-intense x-rays*, Nature **466**, 56 (2010), <http://dx.doi.org/10.1038/nature09177>.
- [6] B. Kanngießer, M. Jainz, S. Brünken, W. Bente, C. Gerth, K. Godehusen, K. Tiedtke, P. van Kampen, A. Tutay, P. Zimmermann, V. F. Demekhin, A. G. Kochur, Phys. Rev. A **62**, 14702 (2000), <http://dx.doi.org/10.1103/PhysRevA.62.014702>.
