# Supplementary material for: Neon in ultrashort and intense x rays from free electron lasers
Source: arXiv:1705.07521 ancillary file (2022-11-07)
Supplement: Supplementary file 4 [file neon_trajectory.pdf]

```
In[45]:= SetDirectory[NotebookDirectory[]]
Get["NeonRateEquations.m"]
```

```
Out[45]= /Volumes/Home/cbuth/Desktop/Neon
```

```
In[47]:= HartreeToeV := 27.2113845
eVToHartree := 1/HartreeToeV
JouleToHartree := 2.29371269*^17
MilliJouleToHartree := 1*^-3 * JouleToHartree
BohrToAngstroem := 0.5291772083
AngstroemToBohr := 1/BohrToAngstroem
MicrometerToBohr := 1*^4 * AngstroemToBohr
BohrToMicrometer := 1/MicrometerToBohr
t0ToSecond := 24.18884326505*^-18
t0ToFemtoSecond := 24.18884326505*^-3
FemtoSecondTot0 := 1/t0ToFemtoSecond
crossSectionAUtoBarn := 1*^8 * BohrToAngstroem^2
crossSectionAUtocm2 := crossSectionAUtoBarn * 1*^-24
crossSectioncm2toAU := 1/crossSectionAUtocm2
```

```
In[61]:= neginfinity := -10 000 * FemtoSecondTot0
posinfinity := 10 000 * FemtoSecondTot0
```

# Paths of a neon atom in LCLS radiation

Christian Buth, 13 May 2017

Theoretische Chemie, Physikalisch-Chemisches Institut, Ruprecht-Karls-Universität Heidelberg, Im Neuenheimer Feld 229, 69120 Heidelberg, Germany

---

## LCLS x-ray pulse

LCLS x-ray energy:

```
In[63]:= omegaX := 1200 * eVToHartree
```

LCLS FWHM pulse duration:

```
In[64]:= tauX := 100 * FemtoSecondTot0
```

LCLS around 900 eV produces a fluence of  $8^{*11}$  photons / shot /  $\mu\text{m}^2$ :

```
In[65]:= J0X := 2 * Sqrt[Log[2] / Pi] * 8*^11 / (1*^4 / BohrToAngstroem) ^ 2 / tauX
```

Gaussian x-ray flux pulse shape (See Eq. (7) in Ref. [1]):

```
In[66]:= jxgaussian[J0Xj_, tX_, t_] :=
  J0Xj * Exp[-4 * Log[2] * (t / tX) ^ 2] * UnitStep[t + 2 * tX] * UnitStep[2 * tX - t]
flux[t_] := jxgaussian[J0X, tauX, t]
```

```
In[68]:= Plot[{flux[t / t0ToFemtoSecond], 1 / 2 * flux[0] *
  UnitStep[t / t0ToFemtoSecond + tauX / 2] * UnitStep[tauX / 2 - t / t0ToFemtoSecond]},
  {t, -100, 100}, PlotStyle -> {{Red, Thick}, {Green, Thick}}, PlotRange -> All]
```

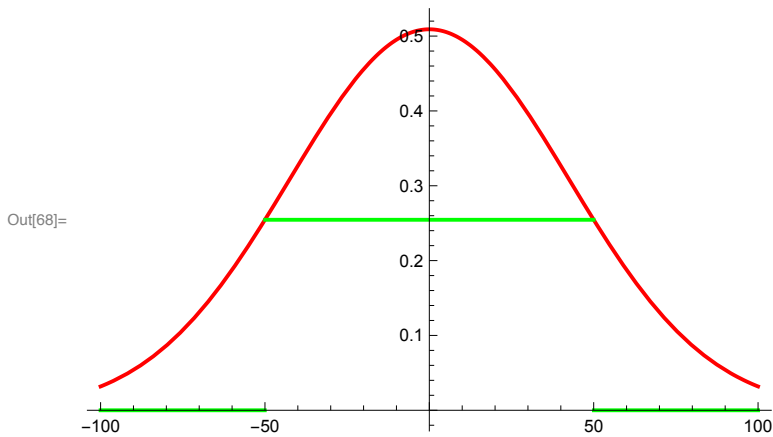

## Path probabilities

```
In[69]:= idxconfig = <|Table[configurations[[i]] -> i, {i, 1, Length[configurations]}]|>
```

```
Out[69]= <| 226 -> 1, 225 -> 2, 216 -> 3, 126 -> 4, 224 -> 5, 215 -> 6, 206 -> 7, 125 -> 8,
  116 -> 9, 026 -> 10, 223 -> 11, 214 -> 12, 205 -> 13, 124 -> 14, 115 -> 15, 106 -> 16,
  025 -> 17, 016 -> 18, 222 -> 19, 213 -> 20, 204 -> 21, 123 -> 22, 114 -> 23, 105 -> 24,
  024 -> 25, 015 -> 26, 006 -> 27, 221 -> 28, 212 -> 29, 203 -> 30, 122 -> 31, 113 -> 32,
  104 -> 33, 023 -> 34, 014 -> 35, 005 -> 36, 220 -> 37, 211 -> 38, 202 -> 39, 121 -> 40,
  112 -> 41, 103 -> 42, 022 -> 43, 013 -> 44, 004 -> 45, 210 -> 46, 201 -> 47, 120 -> 48,
  111 -> 49, 102 -> 50, 021 -> 51, 012 -> 52, 003 -> 53, 200 -> 54, 110 -> 55, 101 -> 56,
  020 -> 57, 011 -> 58, 002 -> 59, 100 -> 60, 010 -> 61, 001 -> 62, 000 -> 63 |>
```

## Radiative decay of certain configurations

### Configurations which decay exclusively radiatively

```
In[70]:= Table[If[! existsGamAtot[[i]] && existsGamRtot[[i]], configurations[[i]], ""],
  {i, 1, Length[existsGamAtot]}
```

```
Out[70]= {, , 216, , , 215, 206, , , , 214, 205, , , , , 213, 204, , , , , , 212, 203, ,
  , , , , , 211, 202, , , , , , 201, , , , , , , 110, 101, , , , , 010, 001, }
```

```
In[71]:= {GamRTot216, GamRTot215, GamRTot206, GamRTot214, GamRTot205, GamRTot213,
          GamRTot204, GamRTot212, GamRTot203, GamRTot211, GamRTot202, GamRTot201,
          GamRTot110, GamRTot101, GamRTot010, GamRTot001} * posinfinity
```

```
Out[71]= {0.201701, 0.161539, 0.191075, 0.115628, 0.147279,
          0.071781, 0.0989526, 0.0360639, 0.0556178, 0.0119578, 0.0237782,
          0.00585518, 7.44227 × 10-8, 23.3024, 2.51004 × 10-7, 62.5627}
```

```
In[72]:= 1 / GamRTot110 * t0ToSecond * 1*^6
```

```
Out[72]= 134.368
```

```
In[73]:= {GamATot126, GamATot125, GamATot124, GamATot123, GamATot122, GamATot121,
          GamATot116, GamATot115, GamATot114, GamATot113, GamATot112, GamATot111,
          GamATot106, GamATot105, GamATot104, GamATot103, GamATot102} * posinfinity
```

```
Out[73]= {4193.8, 3754.43, 3179.21, 2509.36, 1817.75, 1222.32, 3521.07, 2972.37, 2306.89,
          1555.06, 822.556, 239.908, 3625.32, 2902.15, 2077.78, 1228.81, 469.109}
```

```
In[74]:= 1 / GamATot111 * t0ToFemtoSecond
```

```
Out[74]= 41.6827
```

## Decay matrix with exclusively radiative decay widths

```
In[75]:= matRad:=SparseArray[{
  (* No core holes *)
  {idxconfig["216"],idxconfig["216"]}→-GamRTot216,{idxconfig["225"],idxconfig["216"]}→Ga
  {idxconfig["215"],idxconfig["215"]}→-GamRTot215,{idxconfig["224"],idxconfig["215"]}→Ga
  {idxconfig["206"],idxconfig["206"]}→-GamRTot206,{idxconfig["215"],idxconfig["206"]}→Ga
  {idxconfig["214"],idxconfig["214"]}→-GamRTot214,{idxconfig["223"],idxconfig["214"]}→Ga
  {idxconfig["205"],idxconfig["205"]}→-GamRTot205,{idxconfig["214"],idxconfig["205"]}→Ga
  {idxconfig["213"],idxconfig["213"]}→-GamRTot213,{idxconfig["222"],idxconfig["213"]}→Ga
  {idxconfig["204"],idxconfig["204"]}→-GamRTot204,{idxconfig["213"],idxconfig["204"]}→Ga
  {idxconfig["212"],idxconfig["212"]}→-GamRTot212,{idxconfig["221"],idxconfig["212"]}→Ga
  {idxconfig["203"],idxconfig["203"]}→-GamRTot203,{idxconfig["212"],idxconfig["203"]}→Ga
  {idxconfig["211"],idxconfig["211"]}→-GamRTot211,{idxconfig["220"],idxconfig["211"]}→Ga
  {idxconfig["202"],idxconfig["202"]}→-GamRTot202,{idxconfig["211"],idxconfig["202"]}→Ga
  {idxconfig["201"],idxconfig["201"]}→-GamRTot201,{idxconfig["210"],idxconfig["201"]}→Ga

  (* Single core holes *)
  {idxconfig["110"],idxconfig["110"]}→-GamRTot110,{idxconfig["200"],idxconfig["110"]}→Ga
  {idxconfig["101"],idxconfig["101"]}→-GamRTot101,{idxconfig["200"],idxconfig["101"]}→Ga
  {idxconfig["110"],idxconfig["101"]}→GamR110v101,

  (* Double core holes *)
  {idxconfig["010"],idxconfig["010"]}→-GamRTot010,{idxconfig["100"],idxconfig["010"]}→Ga
  {idxconfig["001"],idxconfig["001"]}→-GamRTot001,{idxconfig["100"],idxconfig["001"]}→Ga
  {idxconfig["010"],idxconfig["001"]}→GamR010v001,
  {Length[configurations],Length[configurations]}]}
```



```
In[84]:= posinfinityrad := 1*^10 * posinfinity
```

```
In[85]:= expIntGam = Transpose[Eigenvectors[matRad]].DiagonalMatrix[
  diagelemint[posinfinityrad]].Inverse[Transpose[Eigenvectors[matRad]]];
```

## Branching ratios

```
In[86]:= sol = solveRateEquations[omegaX, flux, neginfinity, posinfinity, 1/3000];
```

```
In[87]:= solProb[sol_, Pxxx_, t1_] := Replace[Pxxx[t], sol[[1]]] /. {t -> t1}
```

```
In[88]:= timePvec[sol_, t1_] := Values[sol[[1]]] /. {t -> t1}
```

## Probabilities at posinfinity, radiative decay has not fully taken place

```
In[89]:= Pvec[sol_] := Values[sol[[1]]] /. {t -> posinfinity}
```

```
In[90]:= pvecsol = Pvec[sol]
```

```
Out[90]= {2.78244 × 10-7, 7.54247 × 10-7, 2.00338 × 10-7, 0., 0.0000352847, 6.1845 × 10-6,
  6.43978 × 10-7, 0., 0., 0., 0.0000256788, 0.0000460765, 5.36251 × 10-6, 0.,
  0., 0., 0., 0.000155981, 0.000300838, 0.000161007, 3.71092 × 10-292,
  1.0101 × 10-288, -4.73842 × 10-307, 0., 0., 0., 0.0000502567, 0.000412682,
  0.000337745, -1.51369 × 10-270, -9.56346 × 10-267, 2.40101 × 10-282, 0., 0., 0.,
  0.0000683434, 0.00110303, 0.00231938, -4.70914 × 10-252, -1.05923 × 10-247,
  2.21847 × 10-259, 0., 0., 0., 0.0030536, 0.00485412, 1.6967 × 10-118,
  2.41293 × 10-113, -8.82327 × 10-204, -9.55351 × 10-291, -1.0398 × 10-285, 0.,
  0.245817, 0.0610461, 1.7782 × 10-11, 3.92265 × 10-224, 7.05598 × 10-218,
  2.67231 × 10-264, 0.680193, 3.39441 × 10-6, 2.23652 × 10-32, 3.07356 × 10-6}
```

```
In[91]:= Total[pvecsol]
```

```
Out[91]= 1.
```

```
In[92]:= expGamInf.timePvec[sol, posinfinity] - expGamInf.timePvec[sol, posinfinity/10]
```

```
Out[92]= {0., -2.11758 × 10-21, 0., 1.95181 × 10-27, 4.74338 × 10-20, 0., 0., -1.31129 × 10-26,
  1.08564 × 10-26, 4.34115 × 10-33, 4.06576 × 10-20, 0., 0., -6.35103 × 10-25,
  -4.52901 × 10-25, 4.94306 × 10-27, 7.78657 × 10-33, -2.58997 × 10-32, 0., 0.,
  0., 4.09258 × 10-25, -2.09147 × 10-24, -2.9693 × 10-25, -1.52257 × 10-30,
  -7.46924 × 10-31, 6.91812 × 10-32, 2.1684 × 10-18, 0., 0., -4.85683 × 10-25,
  -4.15477 × 10-25, 1.89412 × 10-24, 4.04402 × 10-30, -1.91938 × 10-30,
  3.81114 × 10-31, 2.94903 × 10-17, 0., 0., 3.09534 × 10-27, -4.75562 × 10-25,
  -2.03155 × 10-26, -1.50569 × 10-27, -1.41438 × 10-27, -3.74909 × 10-28,
  7.5032 × 10-14, 0., -7.12771 × 10-18, -1.01365 × 10-12, -3.59442 × 10-23,
  -6.30726 × 10-30, 1.35142 × 10-27, 1.17396 × 10-27, 9.39415 × 10-13, 0., 0.,
  3.50913 × 10-33, 1.23958 × 10-27, -2.8297 × 10-31, -1.13243 × 10-14, 0., 0., 0.}
```

```
In[93]:= pvec = expGamInf.pvecsol
```

```
Out[93]= {2.78244 × 10-7, 9.54585 × 10-7, 0., 0., 0.0000421132, 0., 0., 0.,
0., 0., 0.0000771178, 0., 0., 0., 0., 0., 0., 0.000617826, 0., 0.,
3.71092 × 10-292, 1.0101 × 10-288, -4.73842 × 10-307, 0., 0., 0., 0.000800683,
0., 0., -1.51369 × 10-270, -9.56346 × 10-267, 2.40101 × 10-282, 0., 0., 0.,
0.00349075, 0., 0., -4.70914 × 10-252, -1.05923 × 10-247, 2.21847 × 10-259, 0.,
0., 0., 0.00790772, 0., 1.6967 × 10-118, 2.41293 × 10-113, -8.82327 × 10-204,
-9.55351 × 10-291, -1.0398 × 10-285, 0., 0.306863, 0., 0., 3.92265 × 10-224,
7.05598 × 10-218, 2.67231 × 10-264, 0.680196, 0., 0., 3.07356 × 10-6}
```

```
In[94]:= Total[pvec]
```

```
Out[94]= 1.
```

```
In[95]:= Chop[pvec]
```

```
Out[95]= {2.78244 × 10-7, 9.54585 × 10-7, 0, 0, 0.0000421132, 0, 0, 0, 0, 0, 0.0000771178,
0, 0, 0, 0, 0, 0, 0, 0.000617826, 0, 0, 0, 0, 0, 0, 0, 0.000800683, 0,
0, 0, 0, 0, 0, 0, 0.00349075, 0, 0, 0, 0, 0, 0, 0, 0.00790772, 0,
0, 0, 0, 0, 0, 0, 0.306863, 0, 0, 0, 0, 0, 0.680196, 0, 0, 3.07356 × 10-6}
```

```
In[96]:= pvecsol - pvec
```

```
Out[96]= {0., -2.00338 × 10-7, 2.00338 × 10-7, 0., -6.82848 × 10-6, 6.1845 × 10-6,
6.43978 × 10-7, 0., 0., 0., -0.000051439, 0.0000460765, 5.36251 × 10-6,
0., 0., 0., 0., 0., -0.000461845, 0.000300838, 0.000161007, 0., 0.,
0., 0., 0., -0.000750426, 0.000412682, 0.000337745, 0., 0., 0., 0.,
0., 0., -0.00342241, 0.00110303, 0.00231938, 0., 0., 0., 0., 0., 0.,
-0.00485412, 0.00485412, 0., 0., 0., 0., 0., 0., -0.0610461, 0.0610461,
1.7782 × 10-11, 0., 0., 0., -3.39441 × 10-6, 3.39441 × 10-6, 2.23652 × 10-32, 0.}
```

```
In[97]:= intProb[sol_, Pxxx_] := NIntegrate[solProb[sol, Pxxx, t1],
{t1, neginfinity, posinfinity}, AccuracyGoal → 10,
MinRecursion → 5, MaxRecursion → 20, Method → "LocalAdaptive"]
```

```
In[98]:= intProbSol = NIntegrate[Values[sol[[1]]] /. {t → t1},
{t1, neginfinity, posinfinity}, AccuracyGoal → 10,
MinRecursion → 5, MaxRecursion → 20, Method → "LocalAdaptive"]
```

```
Out[98]= {410396., 32.7107, 46.9086, 85.1303, 550.761, 245.624, 80.5041, 3.41802,
5.73894, 1.43989, 31.5494, 81.4117, 19.0622, 59.8478, 30.8923, 9.41375,
0.100372, 0.217154, 193.83, 351.98, 220.923, 4.92735, 14.2129, 3.53745,
1.76049, 1.12254, 0.354648, 24.8548, 222.01, 188.797, 41.1826, 72.1592,
38.5048, 0.243865, 0.851377, 0.194012, 37.9307, 563.88, 1173.79, 5.26827,
39.7641, 24.845, 2.77648, 6.15325, 2.51494, 1268.06, 2082.29, 16.9445,
409.998, 340.288, 0.227728, 4.73442, 1.77101, 97663.8, 25256.5, 4077.07,
0.00112337, 0.170211, 0.192627, 280784., 1.40358, 0.188645, 1.26675}
```

```
In[99]:= intProbRad = intProbSol + expIntGam . pvecsol
```

```
Out[99]= {1.15071 × 109, 3.94639 × 109, 47.3192, 85.1303, 1.74102 × 1011, 263.099, 81.8974,
3.41802, 5.73894, 1.43989, 3.18816 × 1011, 265.326, 34.1148, 59.8478,
30.8923, 9.41375, 0.100372, 0.217154, 2.55418 × 1012, 3011.92, 893.594,
4.92735, 14.2129, 3.53745, 1.76049, 1.12254, 0.354648, 3.31013 × 1012,
8824.42, 2699.29, 41.1826, 72.1592, 38.5048, 0.243865, 0.851377, 0.194012,
1.44312 × 1013, 118 886., 41 499.1, 5.26827, 39.7641, 24.845, 2.77648, 6.15325,
2.51494, 3.26916 × 1013, 344 815., 16.9445, 409.998, 340.288, 0.227728,
4.73442, 1.77101, 1.26827 × 1015, 3.39108 × 1011, 4077.07, 0.00112337,
0.170211, 0.192627, 2.81203 × 1015, 5.59072 × 106, 0.188645, 1.27065 × 1010}
```

```
In[100]:= intProbRad - intProbSol
```

```
Out[100]= {1.1503 × 109, 3.94639 × 109, 0.410621, 0., 1.74102 × 1011, 17.4755, 1.39332, 0.,
0., 0., 3.18816 × 1011, 183.914, 15.0526, 0., 0., 0., 0., 2.55418 × 1012,
2659.94, 672.671, 0., 0., 0., 0., 0., 3.31013 × 1012, 8602.41, 2510.5, 0.,
0., 0., 0., 0., 1.44312 × 1013, 118 322., 40 325.3, 0., 0., 0., 0., 0., 0.,
3.26916 × 1013, 342 733., 0., 0., 0., 0., 0., 0., 1.26827 × 1015, 3.39108 × 1011,
3.15476 × 10-7, 0., 0., 0., 2.81203 × 1015, 5.59072 × 106, 0., 1.27065 × 1010}
```

```
In[101]:= intProbFlux[sol_, Pxxx_] := NIntegrate[solProb[sol, Pxxx, t1] * flux[t1],
{t1, neginfinity, posinfinity}, AccuracyGoal → 10,
MinRecursion → 5, MaxRecursion → 20, Method → "LocalAdaptive"]
```

```
In[102]:= intProbFluxSol = NIntegrate[(Values[sol[[1]]] /. {t → t1}) * flux[t1],
{t1, neginfinity, posinfinity}, AccuracyGoal → 10,
MinRecursion → 5, MaxRecursion → 20, Method → "LocalAdaptive"]
```

```
Out[102]= {148.395, 6.03032, 8.0474, 12.8926, 106.308, 46.4293, 14.5264, 0.932049,
1.47548, 0.338168, 7.09088, 19.4052, 5.08137, 17.3075, 8.70628, 2.52316,
0.0330571, 0.0683504, 43.6897, 75.043, 49.3616, 1.85768, 5.29198, 1.27851,
0.610893, 0.381382, 0.115549, 2.88572, 21.5337, 18.5938, 15.8984, 28.1208,
14.7693, 0.100429, 0.347627, 0.0772424, 4.98263, 48.9021, 86.4089, 2.2995,
17.3457, 10.8243, 1.17078, 2.61327, 1.05235, 9.77629, 36.0317, 7.44967,
154.913, 144.486, 0.103759, 2.15733, 0.805775, 104.374, 77.2041, 236.518,
0.000523832, 0.0742308, 0.0886591, 605.062, 0.00385276, 0.0242003, 0.00188413}
```

## Determine the probabilities for branching into photoionization, Auger decay, or radiative decay

```

In[104]:= totprobrad[lmn_] :=
Module[{slmn, xscTotlmn, GamATotlmn, GamRTotlmn, px, pa, pr},
  slmn = ToString[lmn];
  xscTotlmn = Symbol["xscTot" <> slmn];
  GamATotlmn = Symbol["GamATot" <> slmn];
  GamRTotlmn = Symbol["GamRTot" <> slmn];
  If[existsxsctot[[idxconfig[slmn]]],
    px = xscTotlmn[omegaX] * intProbFluxSol[[idxconfig[slmn]]],
    px = 0
  ];
  If[existsGamAtot[[idxconfig[slmn]]],
    pa = GamATotlmn * intProbRad[[idxconfig[slmn]]],
    pa = 0
  ];
  If[existsGamRtot[[idxconfig[slmn]]],
    pr = GamRTotlmn * intProbRad[[idxconfig[slmn]]],
    pr = 0
  ];
  If[px + pa + pr != 0,
    {px / (px + pa + pr), pa / (px + pa + pr), pr / (px + pa + pr)},
    {0, 0, 0}
  ]
]

```



```

In[111]:= branching =
  Table[totprobrad[configurations[[i]]], {i, 1, Length[configurations]}]
Out[111]:= {{1., 0., 0.}, {1., 0., 0.}, {0.99957, 0., 0.000430293},
  {0.0529713, 0.931264, 0.0157652}, {1., 0., 0.}, {0.999596, 0., 0.000403538},
  {0.999589, 0., 0.000410656}, {0.0832073, 0.900888, 0.0159051},
  {0.109319, 0.874579, 0.0161016}, {0.00610051, 0.976422, 0.0174773},
  {1., 0., 0.}, {0.999158, 0., 0.000841642}, {0.999539, 0., 0.000461467},
  {0.0846384, 0.898627, 0.0167349}, {0.104539, 0.877443, 0.0180182},
  {0.0993518, 0.880504, 0.020144}, {0.00817303, 0.973319, 0.0185079},
  {0.00701531, 0.973017, 0.0199674}, {1., 0., 0.},
  {0.998447, 0., 0.00155322}, {0.999031, 0., 0.000969308},
  {0.127865, 0.855293, 0.0168421}, {0.15347, 0.826834, 0.019696},
  {0.129887, 0.847569, 0.0225439}, {0.00919127, 0.970949, 0.0198596},
  {0.00732073, 0.970067, 0.022612}, {0.00474327, 0.971749, 0.0235076},
  {1., 0., 0.}, {0.991952, 0., 0.00804784}, {0.995337, 0., 0.0046626},
  {0.164465, 0.81907, 0.016465}, {0.202588, 0.774404, 0.023008},
  {0.151661, 0.821163, 0.0271752}, {0.0133367, 0.965136, 0.0215272},
  {0.00948566, 0.963845, 0.0266688}, {0.00524128, 0.967027, 0.0277322},
  {1., 0., 0.}, {0.986543, 0., 0.0134567}, {0.993569, 0., 0.00643135},
  {0.138962, 0.847037, 0.0140011}, {0.260073, 0.710226, 0.0297015},
  {0.156518, 0.805937, 0.0375453}, {0.0205769, 0.956705, 0.0227184},
  {0.0141848, 0.952134, 0.0336811}, {0.006099, 0.959431, 0.0344696},
  {1., 0., 0.}, {0.972145, 0., 0.0278552}, {0.103801, 0.896199, 9.72602 × 10-10},
  {0.133551, 0.802428, 0.064021}, {0.0249001, 0.89456, 0.0805396},
  {0.0377214, 0.942726, 0.0195531}, {0.0273439, 0.924789, 0.0478668},
  {0.00860578, 0.943108, 0.0482865}, {1., 0., 0.}, {0.264269, 0., 0.735731},
  {0.0407442, 0., 0.959256}, {0.0620051, 0.937995, 2.3441 × 10-10},
  {0.0924147, 0.818527, 0.0890588}, {0.016477, 0.894218, 0.0893054},
  {0, 0, 0}, {0.250891, 0., 0.749109}, {0.0635307, 0., 0.936469}, {0, 0, 0}}

```

## Convert symbolic representation of path weights into numbers

```

In[112]:= numpathset = pathset;
In[113]:= DeleteFile["numpathset.m"]
  Save["numpathset.m", numpathset]
In[115]:= Get["numpathset.m"];
In[117]:= Table[Length[numpathset[[i]]], {i, 1, Length[numpathset]}]
Out[117]:= {1, 2, 1, 1, 9, 6, 2, 3, 2, 1, 45, 33, 13, 13, 12, 5, 4, 3, 237, 179, 76, 62, 65, 37,
  17, 19, 8, 1261, 962, 419, 316, 342, 222, 79, 101, 64, 6719, 5142, 2261, 1656,
  1800, 1227, 395, 522, 387, 27403, 12086, 8770, 9515, 6592, 2051, 2717, 2136,
  185016, 85553, 35097, 10821, 14283, 11445, 574522, 171482, 60825, 806829}

```

## Sum over all path weights for each configuration

```

In[118]:= totalpathset = Table[Total[numpathset[[i]]], {i, 1, Length[numpathset]}]
Out[118]= {1, 0.0190385, 0.0536532, 0.927331, 0.522572, 0.253055, 0.0921747, 0.0201602,
  0.0558885, 0.0416692, 0.017815, 0.0794475, 0.0226981, 0.511349, 0.251268,
  0.0937546, 0.00151307, 0.00566399, 0.217811, 0.332193, 0.219111, 0.0192116,
  0.0868073, 0.0254171, 0.0360662, 0.0236954, 0.00873338, 0.0085571, 0.0767943,
  0.0624667, 0.220408, 0.345377, 0.233889, 0.00212916, 0.0123065, 0.00323445,
  0.0388605, 0.248702, 0.363605, 0.00976504, 0.0899033, 0.0741699, 0.029719,
  0.0631365, 0.0336821, 0.0403003, 0.113381, 0.0431299, 0.287514, 0.422144,
  0.000875271, 0.020648, 0.0114692, 0.859005, 0.0589063, 0.173519, 3.05541 × 10-6,
  0.000205133, 0.000488128, 0.882274, 3.39609 × 10-6, 0.0000237935, 2.36367 × 10-6}

In[119]:= Total[totalpathset]
Out[119]= 9.7687

In[120]:= Total[totalpathset[[{idxconfig["225"], idxconfig["216"], idxconfig["126"]}]]]
Out[120]= 1.00002

In[121]:= Total[totalpathset[[{idxconfig["224"], idxconfig["215"], idxconfig["125"],
  idxconfig["206"], idxconfig["116"], idxconfig["026"]}]]]
Out[121]= 0.98552

In[122]:= Total[totalpathset[[{idxconfig["100"], idxconfig["010"], idxconfig["001"]}]]]
Out[122]= 0.882301

In[123]:= Total[totalpathset[[{idxconfig["000"]}]]]
Out[123]= 2.36367 × 10-6

```

## Determine terminal probabilities as the sum over all configurations of a charge state

```

In[125]:= terminalcfg = Map[idxconfig,
  {"226", "225", "224", "223", "222", "221", "220", "210", "200", "100", "000"}]
Out[125]= {1, 2, 5, 11, 19, 28, 37, 46, 54, 60, 63}

In[126]:= totalPvec[cfgs_] := Total[pvec[[Map[idxconfig, cfgs]]]]

```

```

In[127]:= pstayvec = Normal[SparseArray[
  terminalcfg → {
    totalPvec[{"226"}],
    totalPvec[{"225", "216", "126"}],
    totalPvec[{"224", "215", "206", "125", "116", "026"}],
    totalPvec[{"223", "214", "205", "124", "115", "106", "025", "016"}],
    totalPvec[{"222", "213", "204", "123", "114", "105", "024", "015", "006"}],
    totalPvec[{"221", "212", "203", "122", "113", "104", "023", "014", "005"}],
    totalPvec[{"220", "211", "202", "121", "112", "103", "022", "013", "004"}],
    totalPvec[{"210", "201", "120", "111", "102", "021", "012", "003"}],
    totalPvec[{"200", "110", "101", "020", "011", "002"}],
    totalPvec[{"100", "010", "001"}],
    totalPvec[{"000"}]
  ],
  Length[pvec], 0
]]

Out[127]= {2.78244 × 10-7, 9.54585 × 10-7, 0, 0, 0.0000421132, 0, 0, 0, 0, 0, 0.0000771178,
  0, 0, 0, 0, 0, 0, 0, 0.000617826, 0, 0, 0, 0, 0, 0, 0, 0.000800683, 0,
  0, 0, 0, 0, 0, 0, 0, 0.00349075, 0, 0, 0, 0, 0, 0, 0, 0.00790772, 0,
  0, 0, 0, 0, 0, 0, 0.306863, 0, 0, 0, 0, 0, 0.680196, 0, 0, 3.07356 × 10-6}

In[128]:= Total[pstayvec]

Out[128]= 1.

```

## Calculation of the probability of the paths

```

In[129]:= pathprob = Table[
  If[numpathset[[i]] == {}, {0}, numpathset[[i]] / safeTot[totalpathset[[i]]],
  {i, 1, Length[numpathset]}] * pstayvec;

In[130]:= Total[Table[Total[pathprob[[i]]], {i, 1, Length[pathprob]}]]

Out[130]= 1.

```

## Find path with maximum probability

```

In[131]:= tabmaxval = Table[Max[pathprob[[i]]], {i, 1, Length[pathprob]}]

Out[131]= {2.78244 × 10-7, 9.53428 × 10-7, 0., 0., 0.0000420789, 0., 0., 0., 0., 0.,
  0.0000378612, 0., 0., 0., 0., 0., 0., 0.00058307, 0., 0., 0., 0.,
  0., 0., 0., 0., 0.000233198, 0., 0., 0., 0., 0., 0., 0., 0.0027556,
  0., 0., 0., 0., 0., 0., 0., 0.00123469, 0., 0., 0., 0., 0.,
  0., 0.0200333, 0., 0., 0., 0., 0., 0.0432349, 0., 0., 2.19841 × 10-7}

```

```

In[132]:= tabmaxpos = Flatten[Table[
  FirstPosition[pathprob[[i]], Max[pathprob[[i]]]], {i, 1, Length[pathprob]}]]
Out[132]= {1, 1, 1, 1, 7, 1, 1, 1, 1, 1, 7, 1, 1, 1, 1, 1, 1, 189, 1, 1, 1,
  1, 1, 1, 1, 189, 1, 1, 1, 1, 1, 1, 1, 5419, 1, 1, 1, 1, 1, 1, 1,
  10936, 1, 1, 1, 1, 1, 1, 1, 158362, 1, 1, 1, 1, 1, 491943, 1, 1, 321145}

In[136]:= Table[{configurations[[i]],
  pathstr[[i, tabmaxpos[[i]]]], ScientificForm[tabmaxval[[i]]],
  ScientificForm[pstayvec[[i]]]}, {i, terminalcfg}] // TableForm
Out[136]//TableForm=

```

|     |            |                          |                          |
|-----|------------|--------------------------|--------------------------|
| 226 |            | $2.78244 \times 10^{-7}$ | $2.78244 \times 10^{-7}$ |
| 225 | V          | $9.53428 \times 10^{-7}$ | $9.54585 \times 10^{-7}$ |
| 224 | CA         | $4.20789 \times 10^{-5}$ | $4.21132 \times 10^{-5}$ |
| 223 | VCA        | $3.78612 \times 10^{-5}$ | $7.71178 \times 10^{-5}$ |
| 222 | CACA       | $5.8307 \times 10^{-4}$  | $6.17826 \times 10^{-4}$ |
| 221 | VCACA      | $2.33198 \times 10^{-4}$ | $8.00683 \times 10^{-4}$ |
| 220 | CACACA     | $2.7556 \times 10^{-3}$  | $3.49075 \times 10^{-3}$ |
| 210 | VCACACA    | $1.23469 \times 10^{-3}$ | $7.90772 \times 10^{-3}$ |
| 200 | CACACACA   | $2.00333 \times 10^{-2}$ | $3.06863 \times 10^{-1}$ |
| 100 | CACACACAC  | $4.32349 \times 10^{-2}$ | $6.80196 \times 10^{-1}$ |
| 000 | VCACACDVVV | $2.19841 \times 10^{-7}$ | $3.07356 \times 10^{-6}$ |

## Find $n$ paths with highest probability

```

In[292]:= cfgana[cfg_, rm_] := Module[{ind, tabmaxval, tabmaxpos},
  ind = idxconfig[cfg];
  tabmaxval = TakeLargest[pathprob[[ind]], rm];
  tabmaxpos =
    Flatten[Table[FirstPosition[pathprob[[ind]], tabmaxval[[i]]], {i, 1, rm}]];
  {Table[{i, pathstr[[ind, tabmaxpos[[i]]]], ScientificForm[tabmaxval[[i]]]},
    {i, 1, rm}] // TableForm, ScientificForm[Total[tabmaxval]],
    ScientificForm[Chop[pstayvec[[ind]]]]}
]

In[293]:= cfgana["226", 1]
Out[293]= {1      2.78244 × 10-7 , 2.78244 × 10-7 , 2.78244 × 10-7}

In[294]:= cfgana["225", 2]
Out[294]= {1      V      9.53428 × 10-7 , 9.54585 × 10-7 , 9.54585 × 10-7}
           {2      VR     1.15756 × 10-9 , 9.54585 × 10-7 , 9.54585 × 10-7}

In[295]:= cfgana["224", 2]
Out[295]= {1      CA      4.20789 × 10-5 , 4.21049 × 10-5 , 4.21132 × 10-5}
           {2      VV      2.60003 × 10-8 , 4.21049 × 10-5 , 4.21132 × 10-5}

In[296]:= cfgana["223", 3]
Out[296]= {1      VCA      3.78612 × 10-5
           {2      CAV      3.35438 × 10-5 , 7.67551 × 10-5 , 7.71178 × 10-5}
           {3      CVA      5.35001 × 10-6

```

In[297]:= `cfgana["222", 3]`

Out[297]= 

|   |       |                          |
|---|-------|--------------------------|
| 1 | CACA  | $5.8307 \times 10^{-4}$  |
| 2 | CDA A | $3.20995 \times 10^{-5}$ |
| 3 | CACAR | $7.01489 \times 10^{-7}$ |

,  $6.15871 \times 10^{-4}$ ,  $6.17826 \times 10^{-4}$

In[351]:= `cfgana["221", 9]`

Out[351]= 

|   |        |                          |
|---|--------|--------------------------|
| 1 | VCACA  | $2.33198 \times 10^{-4}$ |
| 2 | CAVCA  | $2.06606 \times 10^{-4}$ |
| 3 | CACAV  | $1.79113 \times 10^{-4}$ |
| 4 | CACVA  | $4.97668 \times 10^{-5}$ |
| 5 | CVACA  | $3.29522 \times 10^{-5}$ |
| 6 | VCDAA  | $2.08786 \times 10^{-5}$ |
| 7 | VCACAR | $1.48294 \times 10^{-5}$ |
| 8 | CAVCAR | $1.2745 \times 10^{-5}$  |
| 9 | CDAAV  | $9.86061 \times 10^{-6}$ |

,  $7.59948 \times 10^{-4}$ ,  $8.00683 \times 10^{-4}$

In[299]:= `cfgana["220", 10]`

Out[299]= 

|    |         |                          |
|----|---------|--------------------------|
| 1  | CACACA  | $2.7556 \times 10^{-3}$  |
| 2  | CACDAA  | $2.51287 \times 10^{-4}$ |
| 3  | CDAACA  | $1.51703 \times 10^{-4}$ |
| 4  | CACACAR | $8.99957 \times 10^{-5}$ |
| 5  | CACACAR | $8.64075 \times 10^{-5}$ |
| 6  | CACACAR | $7.78194 \times 10^{-5}$ |
| 7  | CDADAA  | $1.3834 \times 10^{-5}$  |
| 8  | CACDAAR | $1.03939 \times 10^{-5}$ |
| 9  | CACDAAR | $7.09645 \times 10^{-6}$ |
| 10 | CACDAAR | $6.47788 \times 10^{-6}$ |

,  $3.45062 \times 10^{-3}$ ,  $3.49075 \times 10^{-3}$

In[300]:= `cfgana["210", 10]`

Out[300]= 

|    |         |                          |
|----|---------|--------------------------|
| 1  | VCACACA | $1.23469 \times 10^{-3}$ |
| 2  | CAVCACA | $1.06115 \times 10^{-3}$ |
| 3  | CACAVCA | $8.17686 \times 10^{-4}$ |
| 4  | CACACAV | $3.64647 \times 10^{-4}$ |
| 5  | CACACVA | $3.19984 \times 10^{-4}$ |
| 6  | VCACDAA | $2.22954 \times 10^{-4}$ |
| 7  | CAVCDAA | $1.91618 \times 10^{-4}$ |
| 8  | CACVACA | $1.89389 \times 10^{-4}$ |
| 9  | VCACACA | $1.77668 \times 10^{-4}$ |
| 10 | CAVCACA | $1.71994 \times 10^{-4}$ |

,  $4.75178 \times 10^{-3}$ ,  $7.90772 \times 10^{-3}$

In[301]:= `cfgana["200", 10]`

Out[301]= 

|    |          |                          |
|----|----------|--------------------------|
| 1  | CACACACA | $2.00333 \times 10^{-2}$ |
| 2  | CACACACA | $1.96674 \times 10^{-2}$ |
| 3  | CACACACA | $1.93517 \times 10^{-2}$ |
| 4  | CACACACA | $1.92346 \times 10^{-2}$ |
| 5  | CACACACA | $1.9153 \times 10^{-2}$  |
| 6  | CACACACA | $1.73228 \times 10^{-2}$ |
| 7  | CACACACA | $1.32802 \times 10^{-2}$ |
| 8  | CACACACA | $1.27507 \times 10^{-2}$ |
| 9  | CACACACA | $1.25228 \times 10^{-2}$ |
| 10 | CACACACA | $9.22615 \times 10^{-3}$ |

,  $1.62543 \times 10^{-1}$ ,  $3.06863 \times 10^{-1}$

```
In[302]:= cfgana["100", 10]
```

|    |           |                          |
|----|-----------|--------------------------|
| 1  | CACACACAC | $4.32349 \times 10^{-2}$ |
| 2  | CACACACAC | $4.24453 \times 10^{-2}$ |
| 3  | CACACACAC | $4.1764 \times 10^{-2}$  |
| 4  | CACACACAC | $4.15111 \times 10^{-2}$ |
| 5  | CACACACAC | $4.13351 \times 10^{-2}$ |
| 6  | CACACACAC | $3.73853 \times 10^{-2}$ |
| 7  | CACACACAC | $2.86607 \times 10^{-2}$ |
| 8  | CACACACAC | $2.7518 \times 10^{-2}$  |
| 9  | CACACACAC | $2.70261 \times 10^{-2}$ |
| 10 | CACACACAC | $1.99114 \times 10^{-2}$ |

```
Out[302]= { 5 CACACACAC 4.13351 × 10-2, 3.50792 × 10-1, 6.80196 × 10-1 }
```

```
In[303]:= cfgana["000", 10]
```

|    |            |                          |
|----|------------|--------------------------|
| 1  | VCACACDVVV | $2.19841 \times 10^{-7}$ |
| 2  | CAVCACDVVV | $1.88942 \times 10^{-7}$ |
| 3  | VCACACDVVV | $1.76751 \times 10^{-7}$ |
| 4  | CAVCACDVVV | $1.51908 \times 10^{-7}$ |
| 5  | CACAVCDVVV | $1.45592 \times 10^{-7}$ |
| 6  | CACAVCDVVV | $1.17055 \times 10^{-7}$ |
| 7  | VCACACDVVV | $1.04878 \times 10^{-7}$ |
| 8  | CAVCACDVVV | $9.01373 \times 10^{-8}$ |
| 9  | CACAVCDVVV | $6.94568 \times 10^{-8}$ |
| 10 | CACACVDVVV | $5.69742 \times 10^{-8}$ |

```
Out[303]= { 5 CACAVCDVVV 1.45592 × 10-7, 1.32153 × 10-6, 3.07356 × 10-6 }
```

---

## Sum of path probabilities of duplicate strings

```
In[149]:= uniquestrings = Table[DeleteDuplicates[pathstr[[i]]], {i, terminalcfg}];
```

```
In[305]:= Table[{i, configurations[[terminalcfg[[i]]]],
  Length[pathstr[[terminalcfg[[i]]]]], Length[uniquestrings[[i]]]},
  {i, 1, Length[terminalcfg]}] // TableForm
```

```
Out[305]//TableForm=
```

|    |     |         |        |
|----|-----|---------|--------|
| 1  | 226 | 1       | 1      |
| 2  | 225 | 2       | 2      |
| 3  | 224 | 9       | 8      |
| 4  | 223 | 45      | 30     |
| 5  | 222 | 237     | 115    |
| 6  | 221 | 1261    | 441    |
| 7  | 220 | 6719    | 1693   |
| 8  | 210 | 27 403  | 4128   |
| 9  | 200 | 185 016 | 19 067 |
| 10 | 100 | 574 522 | 58 364 |
| 11 | 000 | 806 829 | 81 803 |

```
In[151]:= strProb[cfg_, str_] := Module[{pos},
  pos = Flatten[Position[pathstr[[cfg]], str]];
  Total[pathprob[[cfg, pos]]]
]
```

```
In[153]:= tabstrProb = Table[Table[{str, strProb[terminalcfg[[i]], str]},
  {str, uniquestrings[[i]]}], {i, 1, Length[terminalcfg]}];
```

```
In[154]:= DeleteFile["duplstrprob.m"]
Save["duplstrprob.m", tabstrProb]
```

```
In[156]:= Get["duplstrprob.m"];
```

```
In[157]:= configurations[[terminalcfg[[3]]]]
```

```
Out[157]= 224
```

```
In[158]:= Sort[tabsrProb[[3]], #1[[2]] > #2[[2]] &][[1 ;; 2]] // TableForm
```

```
Out[158]//TableForm=
```

|    |                          |
|----|--------------------------|
| CA | 0.0000420789             |
| VV | $2.60003 \times 10^{-8}$ |

```
In[159]:= configurations[[terminalcfg[[4]]]]
```

```
Out[159]= 223
```

```
In[160]:= Sort[tabsrProb[[4]], #1[[2]] > #2[[2]] &][[1 ;; 3]] // TableForm
```

```
Out[160]//TableForm=
```

|     |                          |
|-----|--------------------------|
| VCA | 0.0000378612             |
| CAV | 0.0000335438             |
| CVA | $5.35001 \times 10^{-6}$ |

```
In[161]:= Total[Sort[tabsrProb[[4]], #1[[2]] > #2[[2]] &][[1 ;; 2]]]
```

```
Out[161]= {CAV + VCA, 0.0000714051}
```

```
In[162]:= configurations[[terminalcfg[[5]]]]
```

```
Out[162]= 222
```

```
In[163]:= Sort[tabsrProb[[5]], #1[[2]] > #2[[2]] &][[1 ;; 3]] // TableForm
```

```
Out[163]//TableForm=
```

|       |                          |
|-------|--------------------------|
| CACA  | 0.00058307               |
| CDAA  | 0.0000320995             |
| CACAR | $1.37501 \times 10^{-6}$ |

```
In[164]:= Total[Sort[tabsrProb[[5]], #1[[2]] > #2[[2]] &][[1 ;; 2]]]
```

```
Out[164]= {CACA + CDAA, 0.000615169}
```

```
In[165]:= configurations[[terminalcfg[[6]]]]
```

```
Out[165]= 221
```

```
In[350]:= Sort[tabsrProb[[6]], #1[[2]] > #2[[2]] &][[1 ;; 10]] // TableForm
```

```
Out[350]//TableForm=
```

|        |                          |
|--------|--------------------------|
| VCACA  | 0.000233198              |
| CAVCA  | 0.000206606              |
| CACAV  | 0.000179113              |
| CACVA  | 0.0000497668             |
| CVACA  | 0.0000329522             |
| VCDA   | 0.0000208786             |
| VCACAR | 0.0000189914             |
| CAVCAR | 0.0000166076             |
| CACAVR | 0.0000133187             |
| CDAAV  | $9.86061 \times 10^{-6}$ |

```
In[304]:= Total[Sort[tabsrProb[[6]], #1[[2]] > #2[[2]] &][[1 ;; 9]]]
```

```
Out[304]= {CACAV + CACAVR + CACVA + CAVCA + CAVCAR + CVACA + VCACA + VCACAR + VCDA, 0.000771431}
```

```
In[168]:= configurations[[terminalcfg[[7]]]]
```

```
Out[168]= 220
```

```
In[349]:= Sort[tabsrProb[[7]], #1[[2]] > #2[[2]] &][[1 ;; 8]] // TableForm
```

```
Out[349]//TableForm=
```

|         |                          |
|---------|--------------------------|
| CACACA  | 0.0027556                |
| CACACAR | 0.000254223              |
| CACDAA  | 0.000251287              |
| CDAACA  | 0.000151703              |
| CACDAAR | 0.0000239682             |
| CDADAA  | 0.000013834              |
| CDAACAR | 0.000013061              |
| CACARCA | $6.49833 \times 10^{-6}$ |

```
In[170]:= configurations[[terminalcfg[[8]]]]
```

```
Out[170]= 210
```

```
In[171]:= Sort[tabsrProb[[8]], #1[[2]] > #2[[2]] &][[1 ;; 36]] // TableForm
```

```
Out[171]//TableForm=
```

|          |                          |
|----------|--------------------------|
| VCACACA  | 0.00171558               |
| CAVCACA  | 0.00150179               |
| CACAVCA  | 0.00121211               |
| CACACAV  | 0.000598892              |
| CACACVA  | 0.000497191              |
| VCACDAA  | 0.000295014              |
| CACVACA  | 0.000292469              |
| CAVCDAA  | 0.000258094              |
| VCDAACA  | 0.000190308              |
| CVACACA  | 0.000188184              |
| VCACACAR | 0.000142581              |
| CAVCACAR | 0.000123957              |
| CACAVCAR | 0.000105364              |
| CACACAVR | 0.0000687317             |
| CDAAVCA  | 0.0000651869             |
| CACDAAV  | 0.0000553373             |
| CACVDAA  | 0.000049659              |
| CACDAVA  | 0.0000459102             |
| CACACVAR | 0.0000408128             |
| CACACARV | 0.0000358499             |
| VCDADAA  | 0.0000330419             |
| CDAACAV  | 0.0000321094             |
| CVACDAA  | 0.0000318931             |
| CDAACVA  | 0.0000266925             |
| CACVACAR | 0.0000246644             |
| VCACDAAR | 0.0000215299             |
| CVDAACA  | 0.0000202934             |
| CACDVAA  | 0.00001919               |
| CAVCDAAR | 0.0000187176             |
| VCACARCA | 0.0000168656             |
| CDAVACA  | 0.0000157027             |
| CVACACAR | 0.0000155281             |
| VCDAACAR | 0.0000147242             |
| CAVCARCA | 0.000014694              |
| CACAVRCA | 0.0000121603             |
| CDVAACA  | $7.85105 \times 10^{-6}$ |

```
In[172]:= configurations[[terminalcfg[[9]]]]
```

```
Out[172]= 200
```



```
In[173]:= Sort[tabsrProb[[9]], #1[[2]] > #2[[2]] &][[1 ;; 10]] // TableForm
Out[173]//TableForm=
CACACACA      0.162543
CACACDAA      0.0316112
CACDAACA      0.0148556
CACACACVR     0.0121094
VCACACACR     0.0108461
CAVCACACR     0.00944267
CDAACACA      0.00814421
CACAVCACR     0.00794335
CACACAVCR     0.00493466
CACACVACR     0.0031125
```

```
In[174]:= configurations[[terminalcfg[[10]]]]
Out[174]= 100
```

```
In[175]:= Sort[tabsrProb[[10]], #1[[2]] > #2[[2]] &][[1 ;; 10]] // TableForm
Out[175]//TableForm=
CACACACAC     0.350792
CACACDAAC     0.0682218
CACDAACAC     0.0320606
CACACACVRC    0.0261339
VCACACACRC    0.0234075
CAVCACACRC    0.0203787
CDAACACAC     0.0175764
CACAVCACRC    0.017143
CACACAVCRC    0.0106497
CACACVACRC    0.00671724
```

```
In[176]:= configurations[[terminalcfg[[11]]]]
Out[176]= 000
```

```
In[177]:= Sort[tabsrProb[[11]], #1[[2]] > #2[[2]] &][[1 ;; 10]] // TableForm
Out[177]//TableForm=
VCACACDVVV    7.5944 × 10-7
CAVCACDVVV    6.64767 × 10-7
CACAVCDVVV    5.40066 × 10-7
CACACVDVVV    2.21993 × 10-7
CACACDVVVV    1.426 × 10-7
CACVACDVVV    1.30805 × 10-7
VCACDADVVV    1.28699 × 10-7
CAVCDADVVV    1.12593 × 10-7
CVACACDVVV    8.41441 × 10-8
VCDAACDVVV    8.32263 × 10-8
```

---

## Sum of path probabilities of normalized strings

```
In[307]:= normstr[str_] := StringJoin[AlphabeticSort[Characters[str]]]
In[308]:= tabnormstrProbDupl =
Table[Table[{normstr[tabsrProb[[j, i, 1]]], tabsrProb[[j, i, 2]]},
  {i, 1, Length[tabsrProb[[j]]}], {j, 1, Length[terminalcfg]}];
```

```

In[309]:= normstrProb[cfg_, str_] := Module[{pos},
  pos = Flatten[Position[tanormstrProbDupl[[cfg, ;;, 1]], str]];
  Total[tanormstrProbDupl[[cfg, pos, 2]]]
]

In[310]:= tanormstr = Table[DeleteDuplicates[tanormstrProbDupl[[i, ;;, 1]],
  {i, 1, Length[terminalcfg]}];

In[306]:= Table[{i, configurations[[terminalcfg[[i]]]],
  Length[pathstr[[terminalcfg[[i]]]], Length[tanormstr[[i]]]},
  {i, 1, Length[terminalcfg]}] // TableForm
Out[306]//TableForm=


|    |     |        |     |
|----|-----|--------|-----|
| 1  | 226 | 1      | 1   |
| 2  | 225 | 2      | 2   |
| 3  | 224 | 9      | 6   |
| 4  | 223 | 45     | 8   |
| 5  | 222 | 237    | 18  |
| 6  | 221 | 1261   | 22  |
| 7  | 220 | 6719   | 41  |
| 8  | 210 | 27403  | 41  |
| 9  | 200 | 185016 | 119 |
| 10 | 100 | 574522 | 175 |
| 11 | 000 | 806829 | 175 |



In[311]:= tanormstrprob = Table[Table[{str, normstrProb[i, str]}, {str, tanormstr[[i]]}],
  {i, 1, Length[terminalcfg]}];

In[312]:= configurations[[terminalcfg[[1]]]]
Out[312]= 226

In[324]:= ScientificForm[Sort[tanormstrprob[[1]], #1[[2]] > #2[[2]] &] // TableForm]
Out[324]//ScientificForm=


|  |                          |
|--|--------------------------|
|  | $2.78244 \times 10^{-7}$ |
|--|--------------------------|



In[192]:= configurations[[terminalcfg[[2]]]]
Out[192]= 225

In[323]:= ScientificForm[Sort[tanormstrprob[[2]], #1[[2]] > #2[[2]] &] // TableForm]
Out[323]//ScientificForm=


|    |                          |
|----|--------------------------|
| V  | $9.53428 \times 10^{-7}$ |
| RV | $1.15756 \times 10^{-9}$ |



In[194]:= configurations[[terminalcfg[[3]]]]
Out[194]= 224

In[322]:= ScientificForm[
  Sort[tanormstrprob[[3]], #1[[2]] > #2[[2]] &][[1 ;; 2]] // TableForm]
Out[322]//ScientificForm=


|    |                          |
|----|--------------------------|
| AC | $4.20789 \times 10^{-5}$ |
| VV | $2.60003 \times 10^{-8}$ |



In[196]:= configurations[[terminalcfg[[4]]]]
Out[196]= 223

```

```
In[321]:= ScientificForm[
  Sort[tabnormstrprob[[4]], #1[[2]] > #2[[2]] &][[1 ;; 2]] // TableForm]
```

```
Out[321]//ScientificForm=
  ACV      7.67551 × 10-5
  ACRV     3.41611 × 10-7
```

```
In[198]:= configurations[[terminalcfg[[5]]]]
```

```
Out[198]= 222
```

```
In[320]:= ScientificForm[
  Sort[tabnormstrprob[[5]], #1[[2]] > #2[[2]] &][[1 ;; 3]] // TableForm]
```

```
Out[320]//ScientificForm=
  AACC      5.8307 × 10-4
  AACD      3.20995 × 10-5
  AACCR     1.48803 × 10-6
```

```
In[200]:= configurations[[terminalcfg[[6]]]]
```

```
Out[200]= 221
```

```
In[319]:= ScientificForm[
  Sort[tabnormstrprob[[6]], #1[[2]] > #2[[2]] &][[1 ;; 4]] // TableForm]
```

```
Out[319]//ScientificForm=
  AACCV      7.01635 × 10-4
  AACCRV     5.6689 × 10-5
  AACDV      3.8096 × 10-5
  AACDRV     3.37801 × 10-6
```

```
In[202]:= Total[Sort[tabnormstrprob[[6]], #1[[2]] > #2[[2]] &][[1 ;; 3]]]
```

```
Out[202]= {AACCRV + AACCV + AACDV, 0.00079642}
```

```
In[203]:= configurations[[terminalcfg[[7]]]]
```

```
Out[203]= 220
```

```
In[343]:= ScientificForm[
  Sort[tabnormstrprob[[7]], #1[[2]] > #2[[2]] &][[1 ;; 4]] // TableForm]
```

```
Out[343]//ScientificForm=
  AAACCC     2.7556 × 10-3
  AAACCD     4.0299 × 10-4
  AAACCCR     2.61255 × 10-4
  AAACCDR     3.74013 × 10-5
```

```
In[341]:= Total[Sort[tabnormstrprob[[7]], #1[[2]] > #2[[2]] &][[1 ;; 3]]]
```

```
Out[341]= {AAACCC + AAACCCR + AAACCD, 0.00341985}
```

```
In[206]:= configurations[[terminalcfg[[8]]]]
```

```
Out[206]= 210
```

```

In[344]:= ScientificForm[
  Sort[tabnormstrprob[[8]], #1[[2]] > #2[[2]] &][[1 ;; 4]] // TableForm]
Out[344]//ScientificForm=
  AAACCCV       $6.00622 \times 10^{-3}$ 
  AAACCDV       $1.11324 \times 10^{-3}$ 
  AAACCCRV      $6.14346 \times 10^{-4}$ 
  AAACCDRV      $9.5873 \times 10^{-5}$ 

In[342]:= Total[Sort[tabnormstrprob[[8]], #1[[2]] > #2[[2]] &][[1 ;; 3]]]
Out[342]= {AAACCCRV + AAACCCV + AAACCDV, 0.0077338}

In[209]:= configurations[[terminalcfg[[9]]]]
Out[209]= 200

In[345]:= ScientificForm[
  Sort[tabnormstrprob[[9]], #1[[2]] > #2[[2]] &][[1 ;; 5]] // TableForm]
Out[345]//ScientificForm=
  AAAACCCC      $1.62543 \times 10^{-1}$ 
  AAAACCCD      $5.4611 \times 10^{-2}$ 
  AAACCCCRV     $5.14423 \times 10^{-2}$ 
  AAACCCDRV     $1.91834 \times 10^{-2}$ 
  AAACCCVV      $6.23143 \times 10^{-3}$ 

In[211]:= Total[Sort[tabnormstrprob[[9]], #1[[2]] > #2[[2]] &][[1 ;; 4]]]
Out[211]= {AAAACCCC + AAAACCCD + AAACCCRV + AAACCCDRV, 0.287779}

In[212]:= configurations[[terminalcfg[[10]]]]
Out[212]= 100

In[346]:= ScientificForm[
  Sort[tabnormstrprob[[10]], #1[[2]] > #2[[2]] &][[1 ;; 7]] // TableForm]
Out[346]//ScientificForm=
  AAAACCCCC     $3.50792 \times 10^{-1}$ 
  AAAACCCCD     $1.17859 \times 10^{-1}$ 
  AAACCCCRV     $1.1102 \times 10^{-1}$ 
  AAACCCDRV     $4.14008 \times 10^{-2}$ 
  AAACCCVV      $2.46493 \times 10^{-2}$ 
  AAAACCCDD     $1.12645 \times 10^{-2}$ 
  AAACCCDVV     $7.6202 \times 10^{-3}$ 

In[214]:= Total[Sort[tabnormstrprob[[10]], #1[[2]] > #2[[2]] &][[1 ;; 6]]]
Out[214]= {AAAACCCCC + AAAACCCCD + AAAACCCDD + AAACCCCRV + AAACCCDRV + AAACCCVV, 0.656985}

In[215]:= configurations[[terminalcfg[[11]]]]
Out[215]= 000

In[347]:= ScientificForm[
  Sort[tabnormstrprob[[11]], #1[[2]] > #2[[2]] &][[1 ;; 3]] // TableForm]
Out[347]//ScientificForm=
  AACCCDVVVV    $2.54381 \times 10^{-6}$ 
  AACCCDVVVV    $4.70654 \times 10^{-7}$ 
  AACCCDRVVVV    $3.0023 \times 10^{-8}$ 

```

```
In[217]:= Total[Sort[tabnormstrprob[[1]], #1[[2]] > #2[[2]] &] [[1 ;; 2]]]
Out[217]:= {AACCCDVVVV + AACCCDDVVVV, 3.01447 × 10-6}
```

## Sum of path probabilities of string lengths

```
In[354]:= tabstrlenProbDupl =
  Table[Table[{StringLength[tabstrProb[[j, i, 1]]], tabstrProb[[j, i, 2]]},
    {i, 1, Length[tabstrProb[[j]]}], {j, 1, Length[terminalcfg]}];

In[355]:= strlenProb[cfg_, len_] := Module[{pos},
  pos = Flatten[Position[tabstrlenProbDupl[[cfg, ;;, 1]], len]];
  Total[tabstrlenProbDupl[[cfg, pos, 2]]]
];

In[356]:= tabstrlen = Table[
  DeleteDuplicates[tabstrlenProbDupl[[i, ;;, 1]], {i, 1, Length[terminalcfg]}]
];

Out[356]:= {{0}, {1, 2}, {2, 3, 4}, {3, 4, 5, 6}, {4, 5, 6, 7, 8}, {5, 6, 7, 8, 9, 10},
  {6, 7, 8, 9, 10, 11, 12}, {7, 8, 9, 10, 11, 12, 13}, {8, 9, 10, 11, 12, 13, 14, 15},
  {9, 10, 11, 12, 13, 14, 15, 16}, {10, 11, 12, 13, 14, 15, 16, 17}}

In[357]:= Table[{i, configurations[[terminalcfg[[i]]]],
  Length[pathstr[[terminalcfg[[i]]]], Length[tabstrlen[[i]]],
  {i, 1, Length[terminalcfg]}} // TableForm

Out[357]//TableForm=


|    |     |        |   |
|----|-----|--------|---|
| 1  | 226 | 1      | 1 |
| 2  | 225 | 2      | 2 |
| 3  | 224 | 9      | 3 |
| 4  | 223 | 45     | 4 |
| 5  | 222 | 237    | 5 |
| 6  | 221 | 1261   | 6 |
| 7  | 220 | 6719   | 7 |
| 8  | 210 | 27403  | 7 |
| 9  | 200 | 185016 | 8 |
| 10 | 100 | 574522 | 8 |
| 11 | 000 | 806829 | 8 |



In[226]:= tabstrlenprob = Table[Table[{str, strlenProb[i, str]}, {str, tabstrlen[[i]]}],
  {i, 1, Length[terminalcfg]}];

In[229]:= configurations[[terminalcfg[[1]]]]

Out[229]= 226

In[340]:= ScientificForm[Sort[tabstrlenprob[[1]], #1[[2]] > #2[[2]] &] // TableForm]
Out[340]//ScientificForm=


|   |                            |
|---|----------------------------|
| 0 | 2.78244 × 10 <sup>-7</sup> |
|---|----------------------------|



In[231]:= configurations[[terminalcfg[[2]]]]

Out[231]= 225
```

```
In[339]:= ScientificForm[Sort[tabsrtenprob[[2]], #1[[2]] > #2[[2]] &] // TableForm]
```

```
Out[339]//ScientificForm=
```

```
1    9.53428 × 10-7
2    1.15756 × 10-9
```

```
In[362]:= Total[Sort[tabsrtenprob[[2]], #1[[2]] > #2[[2]] &][[1 ;; 2]][[2]] //
ScientificForm
```

```
Out[362]//ScientificForm=
```

```
9.54585 × 10-7
```

```
In[233]:= configurations[[terminalcfg[[3]]]]
```

```
Out[233]= 224
```

```
In[338]:= ScientificForm[Sort[tabsrtenprob[[3]], #1[[2]] > #2[[2]] &] // TableForm]
```

```
Out[338]//ScientificForm=
```

```
2    4.21049 × 10-5
3    8.25976 × 10-9
4    1.27232 × 10-12
```

```
In[235]:= configurations[[terminalcfg[[4]]]]
```

```
Out[235]= 223
```

```
In[337]:= ScientificForm[Sort[tabsrtenprob[[4]], #1[[2]] > #2[[2]] &] // TableForm]
```

```
Out[337]//ScientificForm=
```

```
3    7.67758 × 10-5
4    3.41919 × 10-7
5    8.58774 × 10-11
6    9.64625 × 10-15
```

```
In[361]:= Total[Sort[tabsrtenprob[[4]], #1[[2]] > #2[[2]] &][[1 ;; 2]][[2]] //
ScientificForm
```

```
Out[361]//ScientificForm=
```

```
7.71177 × 10-5
```

```
In[237]:= configurations[[terminalcfg[[5]]]]
```

```
Out[237]= 222
```

```
In[336]:= ScientificForm[Sort[tabsrtenprob[[5]], #1[[2]] > #2[[2]] &] // TableForm]
```

```
Out[336]//ScientificForm=
```

```
4    6.16245 × 10-4
5    1.5797 × 10-6
6    1.21943 × 10-9
7    1.27307 × 10-13
8    1.08889 × 10-17
```

```
In[363]:= Total[Sort[tabsrtenprob[[5]], #1[[2]] > #2[[2]] &][[1 ;; 2]][[2]] //
ScientificForm
```

```
Out[363]//ScientificForm=
```

```
6.17825 × 10-4
```

```
In[239]:= configurations[[terminalcfg[[6]]]]
```

```
Out[239]= 221
```

```
In[335]:= ScientificForm[Sort[tabsrtenprob[[6]], #1[[2]] > #2[[2]] &] // TableForm]
```

```
Out[335]//ScientificForm=
```

|    |                           |
|----|---------------------------|
| 5  | $7.40227 \times 10^{-4}$  |
| 6  | $6.01768 \times 10^{-5}$  |
| 7  | $2.78937 \times 10^{-7}$  |
| 8  | $1.51032 \times 10^{-10}$ |
| 9  | $2.26655 \times 10^{-14}$ |
| 10 | $2.05806 \times 10^{-18}$ |

```
In[364]:= Total[Sort[tabsrtenprob[[6]], #1[[2]] > #2[[2]] &][[1 ;; 2]][[2]] //  
ScientificForm
```

```
Out[364]//ScientificForm=
```

$8.00404 \times 10^{-4}$

```
In[241]:= configurations[[terminalcfg[[7]]]]
```

```
Out[241]= 220
```

```
In[334]:= ScientificForm[Sort[tabsrtenprob[[7]], #1[[2]] > #2[[2]] &] // TableForm]
```

```
Out[334]//ScientificForm=
```

|    |                           |
|----|---------------------------|
| 6  | $3.18233 \times 10^{-3}$  |
| 7  | $3.05163 \times 10^{-4}$  |
| 8  | $3.25822 \times 10^{-6}$  |
| 9  | $2.57095 \times 10^{-9}$  |
| 10 | $1.28074 \times 10^{-12}$ |
| 11 | $1.38856 \times 10^{-16}$ |
| 12 | $1.14468 \times 10^{-20}$ |

```
In[365]:= Total[Sort[tabsrtenprob[[7]], #1[[2]] > #2[[2]] &][[1 ;; 2]][[2]] //  
ScientificForm
```

```
Out[365]//ScientificForm=
```

$3.48749 \times 10^{-3}$

```
In[243]:= configurations[[terminalcfg[[8]]]]
```

```
Out[243]= 210
```

```
In[333]:= ScientificForm[Sort[tabsrtenprob[[8]], #1[[2]] > #2[[2]] &] // TableForm]
```

```
Out[333]//ScientificForm=
```

|    |                           |
|----|---------------------------|
| 7  | $7.18455 \times 10^{-3}$  |
| 8  | $7.19168 \times 10^{-4}$  |
| 9  | $3.99138 \times 10^{-6}$  |
| 10 | $9.71853 \times 10^{-9}$  |
| 11 | $5.01064 \times 10^{-12}$ |
| 12 | $7.29799 \times 10^{-16}$ |
| 13 | $6.52807 \times 10^{-20}$ |

```
In[366]:= Total[Sort[tabsrtenprob[[8]], #1[[2]] > #2[[2]] &][[1 ;; 2]][[2]] //  
ScientificForm
```

```
Out[366]//ScientificForm=
```

$7.90372 \times 10^{-3}$

```
In[245]:= configurations[[terminalcfg[[9]]]]
```

```
Out[245]= 200
```

```
In[332]:= ScientificForm[Sort[tabsrtenprob[[9]], #1[[2]] > #2[[2]] &] // TableForm]
```

```
Out[332]//ScientificForm=
```

|    |                           |
|----|---------------------------|
| 8  | $2.29976 \times 10^{-1}$  |
| 9  | $7.54903 \times 10^{-2}$  |
| 10 | $1.39004 \times 10^{-3}$  |
| 11 | $6.82674 \times 10^{-6}$  |
| 12 | $1.36504 \times 10^{-8}$  |
| 13 | $6.88241 \times 10^{-12}$ |
| 14 | $9.85705 \times 10^{-16}$ |
| 15 | $8.74615 \times 10^{-20}$ |

```
In[368]:= Total[Sort[tabsrtenprob[[9]], #1[[2]] > #2[[2]] &][[1 ;; 3]][[2]] //  
ScientificForm
```

```
Out[368]//ScientificForm=
```

$3.06856 \times 10^{-1}$

```
In[247]:= configurations[[terminalcfg[[10]]]]
```

```
Out[247]= 100
```

```
In[331]:= ScientificForm[Sort[tabsrtenprob[[10]], #1[[2]] > #2[[2]] &] // TableForm]
```

```
Out[331]//ScientificForm=
```

|    |                           |
|----|---------------------------|
| 9  | $5.13396 \times 10^{-1}$  |
| 10 | $1.6378 \times 10^{-1}$   |
| 11 | $3.00491 \times 10^{-3}$  |
| 12 | $1.4744 \times 10^{-5}$   |
| 13 | $2.94652 \times 10^{-8}$  |
| 14 | $1.48541 \times 10^{-11}$ |
| 15 | $2.12737 \times 10^{-15}$ |
| 16 | $1.88755 \times 10^{-19}$ |

```
In[369]:= Total[Sort[tabsrtenprob[[10]], #1[[2]] > #2[[2]] &][[1 ;; 3]][[2]] //  
ScientificForm
```

```
Out[369]//ScientificForm=
```

$6.80182 \times 10^{-1}$

```
In[249]:= configurations[[terminalcfg[[11]]]]
```

```
Out[249]= 000
```

```
In[330]:= ScientificForm[Sort[tabsrtenprob[[11]], #1[[2]] > #2[[2]] &] // TableForm]
```

```
Out[330]//ScientificForm=
```

|    |                           |
|----|---------------------------|
| 10 | $3.04136 \times 10^{-6}$  |
| 11 | $3.20953 \times 10^{-8}$  |
| 12 | $1.05745 \times 10^{-10}$ |
| 13 | $5.49896 \times 10^{-14}$ |
| 14 | $8.2023 \times 10^{-18}$  |
| 15 | $7.38029 \times 10^{-22}$ |
| 16 | $1.23156 \times 10^{-30}$ |
| 17 | 0.                        |

```
In[370]:= Total[Sort[tabsrtenprob[[11]], #1[[2]] > #2[[2]] &][[1 ;; 2]][[2]] //  
ScientificForm
```

```
Out[370]//ScientificForm=
```

$3.07346 \times 10^{-6}$



# Graph

```

In[251]:= vertices = Join[{{0, 10}},
  Table[{i - 2, 9}, {i, 1, 3}],
  Table[{i - 3.5, 8}, {i, 1, 6}],
  Table[{i - 4.5, 7}, {i, 1, 8}],
  Table[{i - 5, 6}, {i, 1, 9}],
  Table[{i - 5, 5}, {i, 1, 9}],
  Table[{i - 5, 4}, {i, 1, 9}],
  Table[{i - 4.5, 3}, {i, 1, 8}],
  Table[{i - 3.5, 2}, {i, 1, 6}],
  Table[{i - 2, 1}, {i, 1, 3}],
  {{0, 0}}
];

In[252]:= gr = Graph[edges, VertexCoordinates → vertices,
  VertexLabels → Table[i -> configurations[[i]], {i, 1, 63}],
  VertexLabelStyle → Directive[Brown, 10]]

```

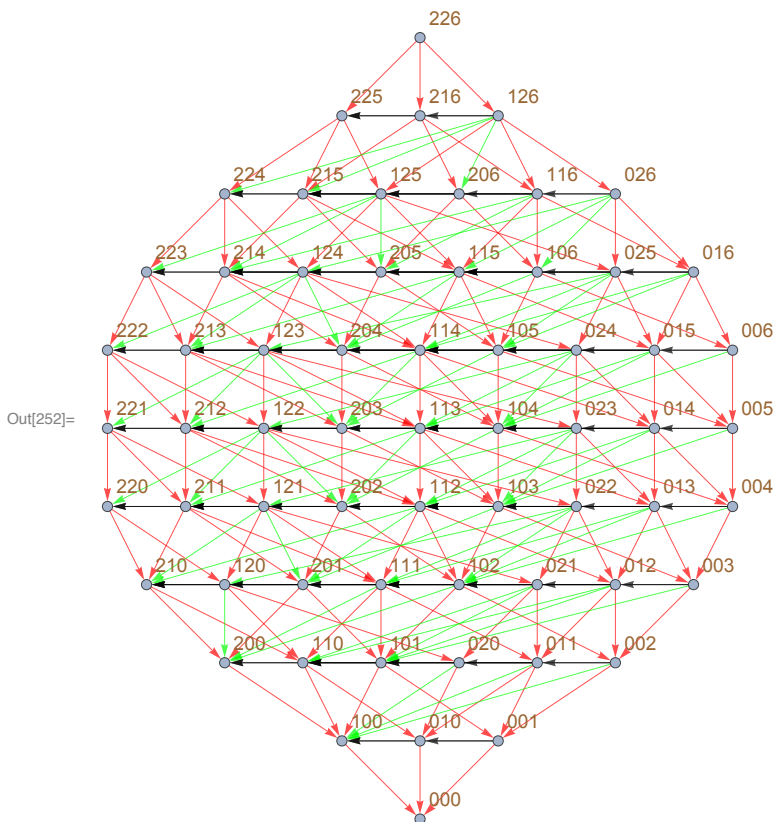

```

In[254]:= probflow[t1_] := Module[{timevec, vertstyle},
  timevec = ArcTan[100 * timePvec[sol, t1]] / (Pi / 2);
  vertstyle =
    Table[{Style[i, ColorData["TemperatureMap"][timevec[[i]]]}], {i, 1, 63}];
  HighlightGraph[gr, vertstyle, VertexSize → Large]
]

```

```

In[256]:= ani = Animate[probflow[t1 * FemtoSecondTot0],
  {t1, -150, 200}, AnimationRunning → False, DefaultDuration → 10]

```

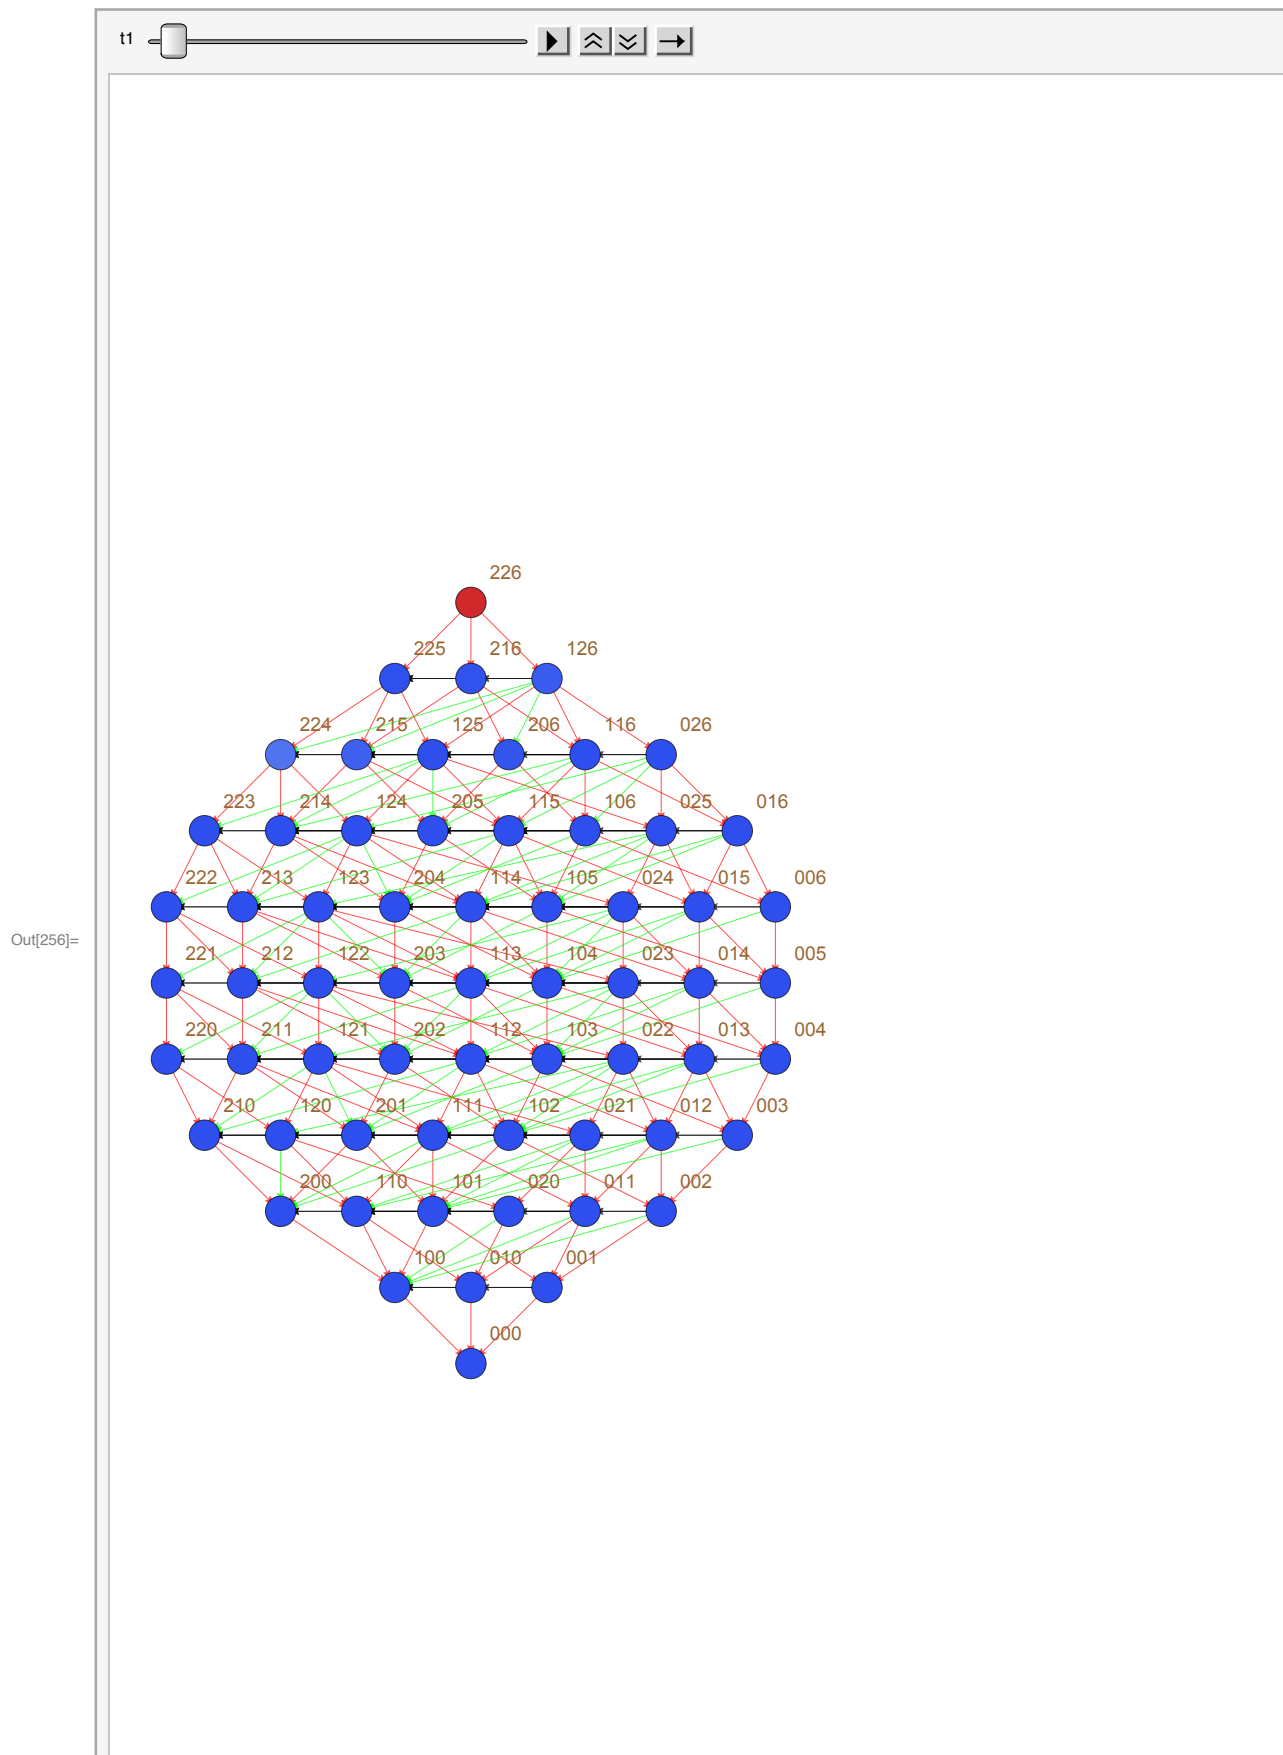

```
In[257]:= Export["req.mov", ani]
```

```
Out[257]= req.mov
```

```
In[258]:= SimpleGraphQ[gr]
```

```
Out[258]= True
```

```
In[262]:= ConnectedGraphQ[gr]
```

```
Out[262]= False
```

```
In[263]:= WeaklyConnectedGraphQ[gr]
```

```
Out[263]= True
```

```
In[261]:= DirectedGraphQ[gr]
```

```
Out[261]= True
```

---

## References

- [1] Christian Buth, Ji-Cai Liu, Mau Hsiung Chen, James P. Cryan, Li Fang, James M. Glowonia, Matthias Hoener, Ryan N. Coffee, Nora Berrah, *Ultrafast absorption of intense x rays by nitrogen molecules*, J. Chem. Phys. **136**, 214310 (2012), <http://dx.doi.org/10.1063/1.4722756>.
