# Supplementary material for: Neon in ultrashort and intense x rays from free electron lasers
Source: arXiv:1705.07521 ancillary file (2022-11-07)
Supplement: Supplementary file 5 [file neon_trends.pdf]

```
Get["NeonRateEquations.m", Path -> NotebookDirectory[]]
```

```
HartreeToeV := 27.2113845
eVToHartree := 1/HartreeToeV
HartreeTomeV := 1000 * HartreeToeV
JouleToHartree := 2.29371269*^17
MilliJouleToHartree := 1*^-3 * JouleToHartree
BohrToAngstroem := 0.5291772083
AngstroemToBohr := 1/BohrToAngstroem
MicrometerToBohr := 1*^4 * AngstroemToBohr
BohrToMicrometer := 1/MicrometerToBohr
t0ToSecond := 24.18884326505*^-18
t0ToFemtoSecond := 24.18884326505*^-3
FemtoSecondTot0 := 1/t0ToFemtoSecond
crossSectionAUtoBarn := 1*^8 * BohrToAngstroem^2
crossSectionAUtocm2 := crossSectionAUtoBarn * 1*^-24
crossSectioncm2toAU := 1/crossSectionAUtocm2
intensityAUtoSI := 6.436409085121321*^15
intensitySItoAU := 1/intensityAUtoSI
```

# Decay widths and fluorescence yields for neon

Christian Buth, 06 May 2017

Theoretische Chemie, Physikalisch-Chemisches Institut, Ruprecht-Karls-Universität Heidelberg, Im Neuenheimer Feld 229, 69120 Heidelberg, Germany

---

## Auger widths

### Total width of single core holes

```
ga = {{GamATot126, GamATot116, GamATot106},
      {GamATot125, GamATot115, GamATot105}, {GamATot124, GamATot114, GamATot104},
      {GamATot123, GamATot113, GamATot103}, {GamATot122, GamATot112, GamATot102},
      {GamATot121, GamATot111, 0}} * HartreeTomeV
{{276.041, 231.761, 238.623}, {247.121, 195.645, 191.023},
 {209.259, 151.842, 136.762}, {165.169, 102.356, 80.882},
 {119.647, 54.1416, 30.8773}, {80.4545, 15.791, 0.}}
```

```
ColorConvert[Lighter[Red], "RGB"] // InputForm
RGBColor[1., 0.3333333333333333, 0.3333333333333333]
```

```
ColorConvert[Lighter[Green], "RGB"] // InputForm
RGBColor[0.3333333333333333, 1., 0.3333333333333333]
```

```
labelcolor := RGBColor[102/255, 102/255, 102/255]
```

```
BarChart[ga, PlotRange → {0, 300},
  ImagePadding → {{All, All}, {40, All}}, Axes → False,
  LabelStyle → {FontFamily → "Helvetica", FontSize → 14}, ChartLabels →
    {Placed[Table[Style[i, labelcolor], {i, 6, 1, -1}], Below], Placed[{}, Above]},
  ChartStyle → {labelcolor, Lighter[Red], Lighter[Green]}, BarSpacing → {Small, 3},
  Frame → True, FrameStyle → Thick, FrameTicks → {{True, True}, {True, False}},
  FrameTicksStyle → {{Thick, Thick}, {Transparent, Thick}},
  FrameLabel → {"Outer valence configuration  $2p^n$ ", "Total decay width  $\Gamma$  [meV]"}]
```

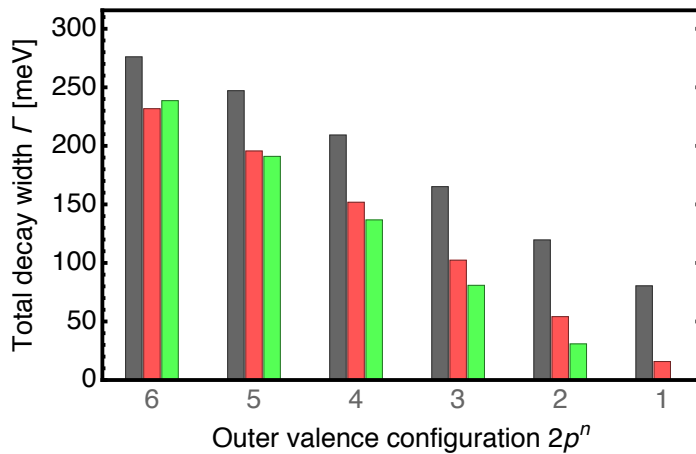

## Total width of double core holes

```
ga = {{GamATot026, GamATot016, GamATot006},
  {GamATot025, GamATot015, GamATot005}, {GamATot024, GamATot014, GamATot004},
  {GamATot023, GamATot013, GamATot003}, {GamATot022, GamATot012, GamATot002},
  {GamATot021, GamATot011, 0}} * HartreeToMeV
{{768.907, 690.597, 651.163}, {663.892, 561.463, 503.193},
  {542.17, 417.905, 352.396}, {408.466, 269.874, 202.918},
  {279.554, 134.942, 75.7072}, {174.531, 35.1239, 0.}}
```

```
BarChart[ga, PlotRange → All,
  ChartLabels → {Placed[{6, 5, 4, 3, 2, 1}, Below], Placed[{}], Above}},
  AxesLabel → {"2p^n", "Γ [meV]"},
  AxesStyle → {{Arrowheads[Automatic], AbsoluteThickness[0.6]},
    {Arrowheads[Automatic], AbsoluteThickness[0.6]}},
  LabelStyle → {FontFamily → "Helvetica"}]
```

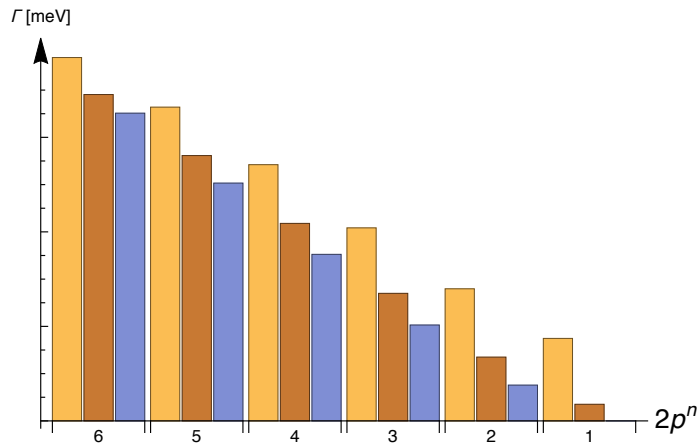

## Radiative widths

### Total width of single core holes

```
ga = {{GamRTot126, GamRTot116, GamRTot106},
  {GamRTot125, GamRTot115, GamRTot105}, {GamRTot124, GamRTot114, GamRTot104},
  {GamRTot123, GamRTot113, GamRTot103}, {GamRTot122, GamRTot112, GamRTot102},
  {GamRTot121, GamRTot111, GamRTot101}} * HartreeToMeV
{{4.67304, 4.26689, 5.45916}, {4.36289, 4.01756, 5.0809},
 {3.89697, 3.61704, 4.52593}, {3.25244, 3.04105, 3.76797},
 {2.40515, 2.26419, 2.77996}, {1.32987, 1.25987, 1.53379}}
```

```
BarChart[ga, PlotRange → {0, 6},
  ImagePadding → {{All, All}, {40, All}}, Axes → False,
  LabelStyle → {FontFamily → "Helvetica", FontSize → 14}, ChartLabels →
    {Placed[Table[Style[i, labelcolor], {i, 6, 1, -1}], Below], Placed[{}], Above}},
  ChartStyle → {labelcolor, Lighter[Red], Lighter[Green]}, BarSpacing → {Small, 3},
  Frame → True, FrameStyle → Thick, FrameTicks → {{True, True}, {True, False}},
  FrameTicksStyle → {{Thick, Thick}, {Transparent, Thick}},
  FrameLabel → {"Outer valence configuration 2pn", "Total decay width  $\Gamma$  [meV]"}]
```

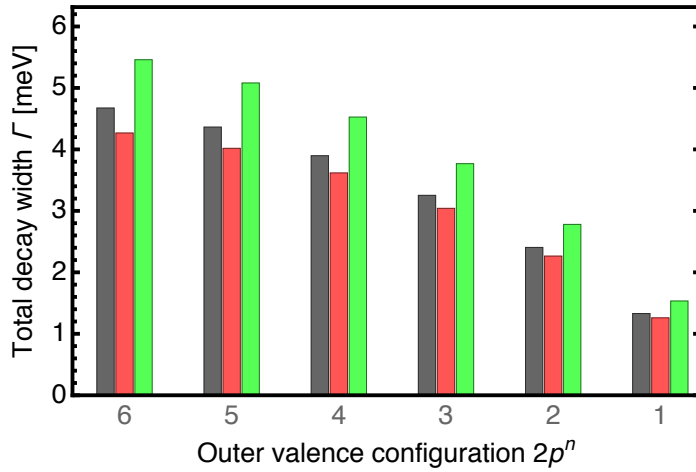

## Total width of double core holes

```
ga = {{GamRTot026, GamRTot016, GamRTot006},
  {GamRTot025, GamRTot015, GamRTot005}, {GamRTot024, GamRTot014, GamRTot004},
  {GamRTot023, GamRTot013, GamRTot003}, {GamRTot022, GamRTot012, GamRTot002},
  {GamRTot021, GamRTot011, GamRTot001}} * HartreeToMeV
{{13.7629, 14.1719, 15.7523}, {12.6241, 13.0875, 14.4304},
{11.0894, 11.5631, 12.6606}, {9.11078, 9.54662, 10.3893},
{6.63844, 6.98454, 7.56087}, {3.61996, 3.82161, 4.11795}}
```

```
BarChart[ga, PlotRange → All,
  ChartLabels → {Placed[{6, 5, 4, 3, 2, 1}, Below], Placed[{}, Above]},
  AxesLabel → {"2pn", "Γ [meV]"},
  AxesStyle → {{Arrowheads[Automatic], AbsoluteThickness[0.6]},
    {Arrowheads[Automatic], AbsoluteThickness[0.6]}},
  LabelStyle → {FontFamily → "Helvetica"}]
```

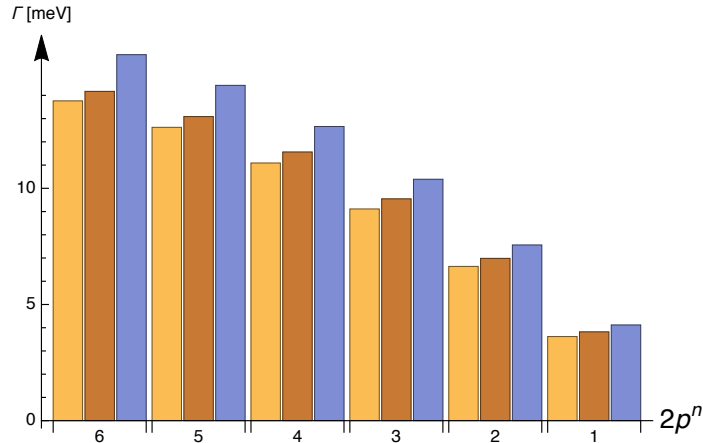

## Fluorescence yields

The fluorescence yield is only approximately determined using Eq. (1) from Ref. [1]. See Ref. [1] for details on probabilistically averaging over fine-structure resolved fluorescence yields.

### Fluorescence yields of single core holes

```
ga = {{GamATot126, GamATot116, GamATot106},
  {GamATot125, GamATot115, GamATot105}, {GamATot124, GamATot114, GamATot104},
  {GamATot123, GamATot113, GamATot103}, {GamATot122, GamATot112, GamATot102},
  {GamATot121, GamATot111, 0}} * HartreeToMeV

{{276.041, 231.761, 238.623}, {247.121, 195.645, 191.023},
 {209.259, 151.842, 136.762}, {165.169, 102.356, 80.882},
 {119.647, 54.1416, 30.8773}, {80.4545, 15.791, 0.}}

gr = {{GamRTot126, GamRTot116, GamRTot106},
  {GamRTot125, GamRTot115, GamRTot105}, {GamRTot124, GamRTot114, GamRTot104},
  {GamRTot123, GamRTot113, GamRTot103}, {GamRTot122, GamRTot112, GamRTot102},
  {GamRTot121, GamRTot111, GamRTot101}} * HartreeToMeV

{{4.67304, 4.26689, 5.45916}, {4.36289, 4.01756, 5.0809},
 {3.89697, 3.61704, 4.52593}, {3.25244, 3.04105, 3.76797},
 {2.40515, 2.26419, 2.77996}, {1.32987, 1.25987, 1.53379}}

gr / (ga + gr)

{{0.016647, 0.0180779, 0.0223661}, {0.0173486, 0.0201217, 0.0259092},
 {0.0182822, 0.0232668, 0.0320334}, {0.0193114, 0.0288534, 0.0445123},
 {0.019706, 0.0401411, 0.0825962}, {0.0162607, 0.073889, 1.}}
```

```
BarChart[gr / (ga + gr), PlotRange → {-0.005, 0.13},
  ChartLabels → {Placed[{6, 5, 4, 3, 2, 1}, Below], Placed[{}], Above}},
  AxesLabel → {"2p^n", " $\omega$ "},
  AxesStyle → {{Arrowheads[Automatic], AbsoluteThickness[0.6]},
    {Arrowheads[Automatic], AbsoluteThickness[0.6]}},
  LabelStyle → {FontFamily → "Helvetica"}]
```

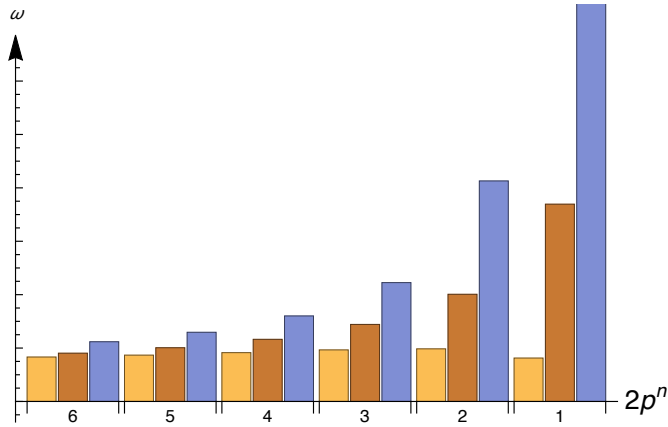

## Fluorescence yields of double core holes

```
ga = {{GamATot026, GamATot016, GamATot006},
  {GamATot025, GamATot015, GamATot005}, {GamATot024, GamATot014, GamATot004},
  {GamATot023, GamATot013, GamATot003}, {GamATot022, GamATot012, GamATot002},
  {GamATot021, GamATot011, 0}} * HartreeTomeV

{{768.907, 690.597, 651.163}, {663.892, 561.463, 503.193},
  {542.17, 417.905, 352.396}, {408.466, 269.874, 202.918},
  {279.554, 134.942, 75.7072}, {174.531, 35.1239, 0.}}

gr = {{GamRTot026, GamRTot016, GamRTot006},
  {GamRTot025, GamRTot015, GamRTot005}, {GamRTot024, GamRTot014, GamRTot004},
  {GamRTot023, GamRTot013, GamRTot003}, {GamRTot022, GamRTot012, GamRTot002},
  {GamRTot021, GamRTot011, GamRTot001}} * HartreeTomeV

{{13.7629, 14.1719, 15.7523}, {12.6241, 13.0875, 14.4304},
  {11.0894, 11.5631, 12.6606}, {9.11078, 9.54662, 10.3893},
  {6.63844, 6.98454, 7.56087}, {3.61996, 3.82161, 4.11795}}

gr / (ga + gr)

{{0.0175845, 0.0201085, 0.0236196}, {0.0186605, 0.0227787, 0.0278783},
  {0.0200438, 0.0269242, 0.0346811}, {0.0218182, 0.0341658, 0.0487056},
  {0.0231957, 0.0492124, 0.0908015}, {0.0203196, 0.0981272, 1.}}
```

```
BarChart[gr / (ga + gr), PlotRange → {-0.005, 0.13},
  ChartLabels → {Placed[{6, 5, 4, 3, 2, 1}, Below], Placed[{}], Above}},
  AxesLabel → {"2p^n", " $\omega$ "},
  AxesStyle → {{Arrowheads[Automatic], AbsoluteThickness[0.6]},
    {Arrowheads[Automatic], AbsoluteThickness[0.6]}},
  LabelStyle → {FontFamily → "Helvetica"}]
```

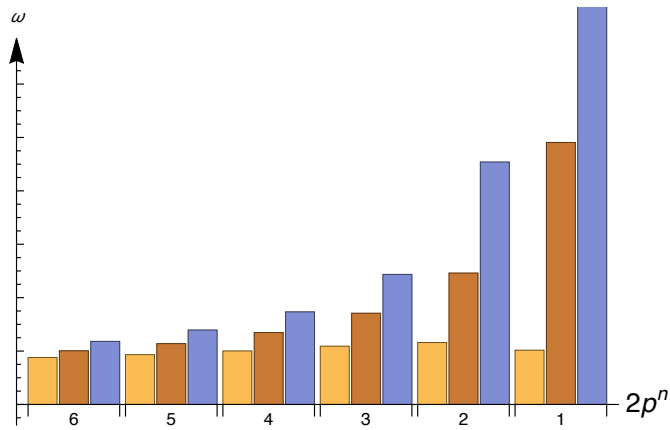

## References

- [1] C. P. Bhalla, *Theoretical fluorescence yields for neon*, Phys. Rev. A **12**, 122 (1975), <http://doi.org/10.1103/PhysRevA.12.122>.
